# Supplementary material for: Modal input-output theory for quantum nanophotonics from the first-order Maxwell operator
Source: arXiv:2610.04043 source file (2026-10-02)
Supplement: Supplementary file 1 [file appendix.tex]

\section{Derivation of the incoming boundary-field commutator}
\label{app:boundary_commutator}
%%%%%%%%%%%%%%%%%%%%%%%%%%%%%%%%%%%%%%%%%%%%

In the main text we used the equal-frequency commutator for the incoming boundary field,
\begin{multline}
\big[
(\bar n\times\hat{\mathcal E}_{\rm in})_i(s,\omega),
(\bar n\times\hat{\mathcal E}_{\rm in}^{\dagger})_j(s',\omega')
\big]
\\
=
-\frac{\hbar k_0}{2\pi\varepsilon_0}
(\bar n\times)_{ij}\,
\delta_S(s-s')\,
\delta(\omega-\omega') .
\label{eq:app_boundary_comm_result}
\end{multline}
% This appendix derives Eq.~\eqref{eq:app_boundary_comm_result} 
Here we derive it from the canonical commutation relations of the incoming modal annihilation and creation operators. 
% The derivation also clarifies the origin of the minus sign: with the surface normal chosen outward from the scattering volume, incoming fields carry negative flux through the boundary.
% We use the same dual-field notation as in the main text and in Ref.~\cite{partI},
% \begin{equation}
% \mathcal E =
% \begin{bmatrix}
% \mathbf E\\
% Z_0\mathbf H
% \end{bmatrix}.
% \end{equation}
On a boundary surface $S$ with outward unit normal $\hat{\mathbf n}$, define the dual tangential trace operator
\begin{equation}
B \equiv \bar n\times
=
\begin{bmatrix}
0 & \hat{\mathbf n}\times\\
-\hat{\mathbf n}\times & 0
\end{bmatrix},
\label{eq:app_B_def}
\end{equation}
such that its operation on the dual field,
\begin{equation}
B\mathcal E
=
\begin{bmatrix}
\hat{\mathbf n}\times Z_0\mathbf H\\
-\hat{\mathbf n}\times \mathbf E
\end{bmatrix}.
\label{eq:app_B_trace}
\end{equation}
highlights the role of operator $B$ as the surface equivalent of the flux metric used throughout the waveguide formalism. It is important to note that $B$ is not invertible on the full six-component field space, since the cross product with $\hat{\mathbf {n}} $ annihilates the normal components. However, $B$ is invertible only after restriction to the tangential subspace, on tangential fields,
\begin{equation}
B^2=\Pi_t,
\label{eq:app_B_square}
\end{equation}
where
\begin{equation}
\Pi_t =
\begin{bmatrix}
I_t & 0\\
0 & I_t
\end{bmatrix},
\qquad
I_t=\mathbf 1-\hat{\mathbf n}\hat{\mathbf n}.
\end{equation}
In the subsequent derivation, we avoid using $B^{-1}$ and instead use the flux-metric closure relation directly.

Let $\{\mathcal E_\mu^{\rm in}(s,\omega)\}$ be a complete set of incoming channel modes on the boundary $S$ at fixed frequency $\omega$. These may be waveguide modes or, in the free-space limit, radiative modes. The only assumptions needed are that the modes are complete on the incoming tangential subspace and are normalized with respect to the boundary flux form.

The boundary flux pairing is
\begin{equation}
\langle \mathcal E_\mu|B|\mathcal E_\nu\rangle_S
\equiv
\int_S
\mathcal E_\mu^\dagger(s,\omega)\,
B\,
\mathcal E_\nu(s,\omega)\,dS .
\label{eq:app_flux_pairing}
\end{equation}
For self-pairing this quantity is proportional to the power flux through $S$,
\begin{equation}
\langle \mathcal E|B|\mathcal E\rangle_S
=
4Z_0\int_S \hat{\mathbf n}\cdot \mathbf S_{\rm avg}\,dS ,
\label{eq:app_flux_power}
\end{equation}
with $\mathbf S_{\rm avg}=\frac{1}{2}\mathrm{Re}(\mathbf E\times\mathbf H^*)$.
Therefore, for a mode incident into the scattering volume through an outward-oriented boundary, the flux is negative:
\begin{equation}
\hat{\mathbf n}\cdot\mathbf S_{\rm avg}<0 .
\end{equation}
We choose the incoming modes to be flux normalized according to
\begin{equation}
\langle \mathcal E_\mu^{\rm in}|B|\mathcal E_\nu^{\rm in}\rangle_S
=
-\delta_{\mu\nu}.
\label{eq:app_incoming_flux_norm}
\end{equation}
The minus sign is purely a convention associated with the outward normal. If the normal were chosen to point into the scattering volume, the same incoming modes would have positive flux norm.

The corresponding closure relation on the incoming tangential subspace is
\begin{equation}
\sum_{\mu\in{\rm in}}
\mathcal E_\mu^{\rm in}(s,\omega)
\mathcal E_\mu^{{\rm in}\dagger}(s',\omega)\,
B
=
-P_{\rm in}(s,s') ,
\label{eq:app_incoming_closure}
\end{equation}
where $P_{\rm in}$ is the projector onto incoming tangential boundary fields. More explicitly, acting on an incoming tangential field $\mathcal F_{\rm in}$,
\begin{equation}
\int_S P_{\rm in}(s,s')\mathcal F_{\rm in}(s')\,dS'
=
\mathcal F_{\rm in}(s).
\end{equation}
For a complete set of both incoming and outgoing channels, Eq.~\eqref{eq:app_incoming_closure} is the incoming-sector part of the full flux closure relation,
\begin{equation}
\sum_{\mu}
\sigma_\mu\,
\mathcal E_\mu(s,\omega)
\mathcal E_\mu^\dagger(s',\omega)\,
B
=
\Pi_t\,\delta_S(s-s'),
\label{eq:app_full_flux_closure}
\end{equation}
where $\sigma_\mu=+1$ for modes carrying outward flux and $\sigma_\mu=-1$ for modes carrying inward flux. Equation~\eqref{eq:app_incoming_closure} follows from Eq.~\eqref{eq:app_full_flux_closure} after restricting to the incoming subspace, where all $\sigma_\mu=-1$.


We now expand the incoming quantum field on $S$ in this flux-normalized basis:
\begin{equation}
\hat{\mathcal E}_{\rm in}(s,\omega)
=
\sqrt{\frac{\hbar k_0}{2\pi\varepsilon_0}}\,
\sum_{\mu\in{\rm in}}
\mathcal E_\mu^{\rm in}(s,\omega)\,
\hat a_\mu(\omega).
\label{eq:app_Ein_mode_expansion}
\end{equation}
The numerical prefactor fixes the physical normalization of the continuum-frequency electric field in the conventions used in the main text. Equivalently, one could absorb this prefactor into the definition of the mode profiles; here we keep the flux-normalized modes dimensionless and write the field normalization explicitly.

The incoming modal operators obey
\begin{equation}
[
\hat a_\mu(\omega),
\hat a_\nu^\dagger(\omega')
]
=
\delta_{\mu\nu}\delta(\omega-\omega'),
\label{eq:app_a_comm}
\end{equation}
with all other annihilation-annihilation and creation-creation commutators vanishing.

Applying the tangential trace operator $B$ to Eq.~\eqref{eq:app_Ein_mode_expansion} gives
\begin{equation}
B\hat{\mathcal E}_{\rm in}(s,\omega)
=
\sqrt{\frac{\hbar k_0}{2\pi\varepsilon_0}}\,
\sum_{\mu\in{\rm in}}
B\mathcal E_\mu^{\rm in}(s,\omega)\,
\hat a_\mu(\omega).
\label{eq:app_BEin_mode_expansion}
\end{equation}
Because $B$ is a c-number operator acting only on the spatial and vector components of the field, it commutes with the modal operators.

We compute the component commutator of the tangential incoming field:
\begin{multline}
\big[
(B\hat{\mathcal E}_{\rm in})_i(s,\omega),
(B\hat{\mathcal E}_{\rm in}^{\dagger})_j(s',\omega')
\big]
\\
=
\frac{\hbar k_0}{2\pi\varepsilon_0}
\sum_{\mu,\nu\in{\rm in}}
(B\mathcal E_\mu^{\rm in})_i(s,\omega)
(B\mathcal E_\nu^{\rm in})_j^*(s',\omega')
\\
\times
[
\hat a_\mu(\omega),
\hat a_\nu^\dagger(\omega')
].
\label{eq:app_comm_step1}
\end{multline}
Using Eq.~\eqref{eq:app_a_comm}, the double sum collapses:
\begin{multline}
\big[
(B\hat{\mathcal E}_{\rm in})_i(s,\omega),
(B\hat{\mathcal E}_{\rm in}^{\dagger})_j(s',\omega')
\big]
\\
=
\frac{\hbar k_0}{2\pi\varepsilon_0}
\sum_{\mu\in{\rm in}}
(B\mathcal E_\mu^{\rm in})_i(s,\omega)
(B\mathcal E_\mu^{\rm in})_j^*(s',\omega)
\,
\delta(\omega-\omega').
\label{eq:app_comm_step2}
\end{multline}
In operator notation the mode sum in Eq.~\eqref{eq:app_comm_step2} is
\begin{equation}
\sum_{\mu\in{\rm in}}
B\mathcal E_\mu^{\rm in}(s)
\mathcal E_\mu^{{\rm in}\dagger}(s')B
=
B
\left[
\sum_{\mu\in{\rm in}}
\mathcal E_\mu^{\rm in}(s)
\mathcal E_\mu^{{\rm in}\dagger}(s')
\right]
B .
\label{eq:app_mode_sum_B}
\end{equation}
We now use the incoming closure relation Eq.~\eqref{eq:app_incoming_closure}. Multiplying Eq.~\eqref{eq:app_incoming_closure} on the left by $B$ gives
\begin{equation}
B
\left[
\sum_{\mu\in{\rm in}}
\mathcal E_\mu^{\rm in}(s)
\mathcal E_\mu^{{\rm in}\dagger}(s')
\right]
B
=
-BP_{\rm in}(s,s').
\label{eq:app_closure_left_B}
\end{equation}
When the resulting distribution acts on incoming tangential boundary data, $P_{\rm in}$ is the identity on that subspace. Thus, within the incoming boundary field algebra,
\begin{equation}
B
\left[
\sum_{\mu\in{\rm in}}
\mathcal E_\mu^{\rm in}(s)
\mathcal E_\mu^{{\rm in}\dagger}(s')
\right]
B
=
-B\,\delta_S(s-s').
\label{eq:app_closure_simplified}
\end{equation}
Componentwise this reads
\begin{equation}
\sum_{\mu\in{\rm in}}
(B\mathcal E_\mu^{\rm in})_i(s)
(B\mathcal E_\mu^{\rm in})_j^*(s')
=
-B_{ij}\,\delta_S(s-s').
\label{eq:app_tangential_mode_sum}
\end{equation}
Substituting Eq.~\eqref{eq:app_tangential_mode_sum} into Eq.~\eqref{eq:app_comm_step2} yields
\begin{multline}
\big[
(B\hat{\mathcal E}_{\rm in})_i(s,\omega),
(B\hat{\mathcal E}_{\rm in}^{\dagger})_j(s',\omega')
\big]
\\
=
-\frac{\hbar k_0}{2\pi\varepsilon_0}
B_{ij}
\delta_S(s-s')
\delta(\omega-\omega').
\label{eq:app_boundary_comm_B}
\end{multline}
Finally restoring $B=\bar n\times$, we recover
\begin{multline}
\big[
(\bar n\times\hat{\mathcal E}_{\rm in})_i(s,\omega),
(\bar n\times\hat{\mathcal E}_{\rm in}^{\dagger})_j(s',\omega')
\big]
\\
=
-\frac{\hbar k_0}{2\pi\varepsilon_0}
(\bar n\times)_{ij}
\delta_S(s-s')
\delta(\omega-\omega'),
\end{multline}
which is Eq.~\eqref{eq:app_boundary_comm_result}.

Several points are worth emphasizing.

First, the sign in Eq.~\eqref{eq:app_boundary_comm_result} is not an independent assumption. It follows from the convention that $\hat{\mathbf n}$ points outward from the scattering volume, whereas $\hat{\mathcal E}_{\rm in}$ propagates into the volume. The flux form is proportional to $\hat{\mathbf n}\cdot\mathbf S_{\rm avg}$, so incoming modes have negative flux norm:
\begin{equation}
\langle \mathcal E_\mu^{\rm in}|B|\mathcal E_\mu^{\rm in}\rangle_S=-1.
\end{equation}
Had the normal been chosen inward for the input surface, the same derivation would give the opposite sign.

Second, the prefactor $\hbar k_0/(2\pi\varepsilon_0)$ is a normalization convention. In Eq.~\eqref{eq:app_Ein_mode_expansion} we chose the mode profiles to be flux normalized according to Eq.~\eqref{eq:app_incoming_flux_norm}. With this convention the physical field amplitude carries the factor $\sqrt{\hbar k_0/(2\pi\varepsilon_0)}$. If this factor is instead absorbed into the mode profiles, the same derivation gives the dimensionless algebraic structure
\begin{equation}
[
B\hat{\mathcal E}_{\rm in},
B\hat{\mathcal E}_{\rm in}^{\dagger}
]
\propto
-B\,\delta_S,
\end{equation}
and the proportionality constant is fixed by matching the continuum-frequency field normalization.

Third, no inverse of $B=\bar n\times$ is required. This is important because $B$ annihilates normal field components and is therefore singular on the full six-component field space. The derivation only uses $B$ acting on tangential boundary data and the flux closure relation Eq.~\eqref{eq:app_incoming_closure}. This makes the result independent of any arbitrary extension of the tangential boundary fields into the normal components.

Finally, Eq.~\eqref{eq:app_boundary_comm_result} is the surface analogue of the bulk Langevin-noise commutator. The bulk commutator is weighted by the material loss tensor $\bar\varepsilon_I$, while the boundary commutator is weighted by the surface flux metric $B=\bar n\times$. In the full field commutator, the two corresponding contributions combine through the generalized optical theorem of Ref.~\cite{partI}, giving
\begin{equation}
[
\hat{\mathcal E}_i(\mathbf r,\omega),
\hat{\mathcal E}_j^\dagger(\mathbf r',\omega')
]
=
\frac{\hbar k_0}{\pi\varepsilon_0}
\operatorname{Im}g_{ij}(\mathbf r,\mathbf r',\omega)
\delta(\omega-\omega').
\end{equation}
Thus the boundary commutator derived here is precisely the modal representation of the boundary-flux term required by macroscopic quantum electrodynamics for finite open systems.

\section{Canonical output commutator from the optical theorem}
\label{app:output_channel_commutator}
\label{app:projected_langevin_noise}

In the main text the output channel operators obey
\begin{equation}
\hat b_m(\omega)
=
\sum_n S_{mn}(\omega)\hat a_n(\omega)
+
\hat\xi_m(\omega).
\label{eq:app_modal_io_start}
\end{equation}
This appendix verifies directly that these operators are canonical,
\begin{equation}
[
\hat b_m(\omega),
\hat b_{m'}^\dagger(\omega')
]
=
\delta_{mm'}\delta(\omega-\omega'),
\label{eq:app_b_canonical}
\end{equation}
by inserting the Green-function expressions for both the scattering amplitude and the Langevin noise.  The proof uses only the canonical incoming-channel algebra, the Langevin polarization-noise commutator, and the generalized optical theorem.

We use the shorthand
\begin{equation}
B_{\rm in}\equiv \bar n_{\rm in}\times,
\qquad
B_{\rm out}\equiv \bar n_{\rm out}\times,
\end{equation}
where the normals point outward from the scattering volume.  The normalized channel operators are defined with
\begin{equation}
\alpha
=
\sqrt{\frac{2\pi\varepsilon_0}{\hbar k_0}},
\label{eq:app_alpha}
\end{equation}
so that the incoming boundary field expansion is
\begin{equation}
\hat{\mathcal E}_{\rm in}(\mathbf s,\omega)
=
\alpha^{-1}\sum_n
\mathcal E_n^{\rm in}(\mathbf s,\omega)\hat a_n(\omega),
\label{eq:app_in_expansion}
\end{equation}
with
\begin{equation}
[
\hat a_n(\omega),
\hat a_{n'}^\dagger(\omega')
]
=
\delta_{nn'}\delta(\omega-\omega').
\label{eq:app_a_comm_oc}
\end{equation}
The output projection is
\begin{equation}
\hat b_m(\omega)
=
\alpha
\int_{S_{\rm out}}
\mathcal E_m^{{\rm out}\dagger}(\mathbf r,\omega)
B_{\rm out}
\hat{\mathcal E}_{\rm out}(\mathbf r,\omega)
dS .
\label{eq:app_b_definition}
\end{equation}

The quantum Stratton--Chu relation gives the output field as the sum of a propagated boundary input and a Langevin-noise field,
\begin{multline}
\hat{\mathcal E}_{\rm out}(\mathbf r,\omega)
=
-i\int_{S_{\rm in}}
g(\mathbf r,\mathbf s,\omega)B_{\rm in}
\hat{\mathcal E}_{\rm in}(\mathbf s,\omega)dS
\\
+
k_0\int_V
g(\mathbf r,\mathbf x,\omega)
\hat{\mathcal P}_N(\mathbf x,\omega)dV_x .
\label{eq:app_Eout_full}
\end{multline}
Substituting Eq.~\eqref{eq:app_Eout_full} into Eq.~\eqref{eq:app_b_definition} gives Eq.~\eqref{eq:app_modal_io_start}, with
\begin{align}
S_{mn}(\omega)
&=
-i\int_{S_{\rm out}}\int_{S_{\rm in}}
\mathcal E_m^{{\rm out}\dagger}(\mathbf r)
B_{\rm out}
g(\mathbf r,\mathbf s,\omega)
\nonumber\\
&\quad\times
B_{\rm in}
\mathcal E_n^{\rm in}(\mathbf s)
\,dS_{\rm in}\,dS_{\rm out},
\label{eq:app_S_def_oc}
\end{align}
and
\begin{align}
\hat\xi_m(\omega)
&=
\alpha k_0\int_{S_{\rm out}}\int_V
\mathcal E_m^{{\rm out}\dagger}(\mathbf r)
B_{\rm out}
g(\mathbf r,\mathbf x,\omega)
\nonumber\\
&\quad\times
\hat{\mathcal P}_N(\mathbf x,\omega)
\,dV_x\,dS_{\rm out}.
\label{eq:app_xi_def_oc}
\end{align}
The input field and material reservoir are independent, so
\begin{equation}
[
\hat a_n(\omega),
\hat\xi_m^\dagger(\omega')
]
=0.
\label{eq:app_cross_zero}
\end{equation}
Therefore
\begin{multline}
[
\hat b_m(\omega),
\hat b_{m'}^\dagger(\omega')
]
=
\sum_n S_{mn}(\omega)S_{m'n}^*(\omega)\delta(\omega-\omega')
\\
+
[
\hat\xi_m(\omega),
\hat\xi_{m'}^\dagger(\omega')
].
\label{eq:app_b_comm_split}
\end{multline}
We now evaluate the two terms on the right-hand side directly.

First, inserting Eq.~\eqref{eq:app_S_def_oc} and using the incoming-channel closure relation from Appendix~\ref{app:boundary_commutator} gives
\begin{equation}
\sum_n S_{mn}S_{m'n}^*
=
-
\langle m_{\rm out}|
g B_{\rm in}g^\dagger
|m'_{\rm out}\rangle .
\label{eq:app_SS_overlap}
\end{equation}
Here the projected overlap means
\begin{align}
\langle m_{\rm out}|\mathcal O|m'_{\rm out}\rangle
&\equiv
\int_{S_{\rm out}}\int_{S_{\rm out}}
\mathcal E_m^{{\rm out}\dagger}(\mathbf r)
B_{\rm out}^\dagger
\mathcal O(\mathbf r,\mathbf r')
\nonumber\\
&\quad\times
B_{\rm out}
\mathcal E_{m'}^{\rm out}(\mathbf r')
dS\,dS'.
\label{eq:app_projected_overlap}
\end{align}
The minus sign in Eq.~\eqref{eq:app_SS_overlap} is the incoming-flux sign associated with the outward normal on $S_{\rm in}$.

Second, using the Langevin polarization-noise commutator
\begin{multline}
[
\hat{\mathcal P}_{N,i}(\mathbf x,\omega),
\hat{\mathcal P}_{N,j}^\dagger(\mathbf y,\omega')
]
=
\frac{\hbar}{\pi\varepsilon_0}
(\bar\varepsilon_I)_{ij}(\mathbf x,\omega)
\\
\times
\delta^{(3)}(\mathbf x-\mathbf y)
\delta(\omega-\omega')
\label{eq:app_PN_comm_oc}
\end{multline}
in Eq.~\eqref{eq:app_xi_def_oc} gives
\begin{equation}
[
\hat\xi_m(\omega),
\hat\xi_{m'}^\dagger(\omega')
]
=
2k_0
\langle m_{\rm out}|
g\bar\varepsilon_I g^\dagger
|m'_{\rm out}\rangle
\delta(\omega-\omega').
\label{eq:app_volume_comm}
\end{equation}
The factor $2k_0$ follows from $\alpha^2 k_0^2\hbar/(\pi\varepsilon_0)=2k_0$.

Combining Eqs.~\eqref{eq:app_b_comm_split}, \eqref{eq:app_SS_overlap}, and~\eqref{eq:app_volume_comm}, we obtain
\begin{multline}
[
\hat b_m(\omega),
\hat b_{m'}^\dagger(\omega')
]
=
\Big[
2k_0
\langle m_{\rm out}|
g\bar\varepsilon_I g^\dagger
|m'_{\rm out}\rangle
\\
-
\langle m_{\rm out}|
gB_{\rm in}g^\dagger
|m'_{\rm out}\rangle
\Big]
\delta(\omega-\omega').
\label{eq:app_comm_before_OT}
\end{multline}
The bracketed expression is exactly the projected generalized optical theorem.  With the present boundary orientation, the relevant projected form is
\begin{multline}
2\langle m_{\rm out}|\operatorname{Im}g|m'_{\rm out}\rangle
=
2k_0
\langle m_{\rm out}|
g\bar\varepsilon_I g^\dagger
|m'_{\rm out}\rangle
\\
-
\langle m_{\rm out}|
gB_{\rm in}g^\dagger
|m'_{\rm out}\rangle .
\label{eq:app_projected_OT}
\end{multline}
Thus
\begin{equation}
[
\hat b_m(\omega),
\hat b_{m'}^\dagger(\omega')
]
=
2\langle m_{\rm out}|\operatorname{Im}g|m'_{\rm out}\rangle
\delta(\omega-\omega').
\label{eq:app_b_comm_Img}
\end{equation}
Finally, the outgoing modes are flux-normalized with the same continuum-field normalization as the input modes, so
\begin{equation}
2\langle m_{\rm out}|\operatorname{Im}g|m'_{\rm out}\rangle
=
\delta_{mm'}.
\label{eq:app_projected_Img_delta}
\end{equation}
Substitution into Eq.~\eqref{eq:app_b_comm_Img} proves Eq.~\eqref{eq:app_b_canonical}.

Equivalently, solving Eq.~\eqref{eq:app_b_comm_split} for the Langevin-noise commutator gives the familiar unitarity-deficit form
\begin{equation}
[
\hat\xi_m(\omega),
\hat\xi_{m'}^\dagger(\omega')
]
=
\left[
\delta_{mm'}-
\sum_n S_{mn}(\omega)S_{m'n}^*(\omega)
\right]
\delta(\omega-\omega').
\label{eq:app_xi_comm_deficit}
\end{equation}
This equation is a consequence of the canonical output commutator, not an additional postulate.  The Langevin noise supplies exactly the part of the output commutator carried by material absorption, while the coherent scattering term supplies the boundary-channel contribution.

\section{Spectral Green functions for cavity and waveguide}
\label{app:spectral_gf}
%%%%%%%%%%%%%%%%%%%%%%%%%%%%%%%%%

\subsection{Cavity spectral Green function}

We derive the spectral representation of the cavity Green kernel used in Sec.~\ref{sec:applications}. The starting point is the general retarded Green kernel~\eqref{eq:cav_green_def}.

Let $V$ be a finite cavity volume bounded by a surface $\partial V$ on which the boundary flux vanishes (e.g., perfect electric or magnetic walls), with a lossless material tensor $\bar{\varepsilon}^\dagger = \bar{\varepsilon}$.  For a lossless medium $\mathcal{H}$ is self-adjoint on the cavity domain (the boundary flux vanishes by assumption), and therefore so is $\mathcal{M}$.  The source-free equation $\mathcal{M}\mathcal{E} = 0$ becomes the generalized frequency eigenproblem~\cite{sakoda2004optical,Flow_of_light_Joannopoulos}
\begin{equation}
\mathcal{H}\,\mathcal{E}_n = k_{0,n}\,\bar{\varepsilon}\,\mathcal{E}_n,
\label{eq:cav_eigenproblem}
\end{equation}
where $k_{0,n} = \omega_n/c$.  This is the closed-system counterpart of the waveguide propagation eigenproblem~\eqref{eq:wg_eigenproblem}: the eigenvalue is now the resonance frequency rather than the propagation constant, and the weight operator is the material tensor $\bar{\varepsilon}$ rather than the flux operator $\bar{\mathbf{z}}\times$.  The natural bilinear form is the energy pairing
\begin{equation}
\begin{aligned}
\langle\mathcal{E}_m|\mathcal{E}_n\rangle_{\bar{\varepsilon}}
&=
\int_V
\mathcal{E}_m^\dagger(\mathbf{r})\,
\bar{\varepsilon}(\mathbf{r})\,
\mathcal{E}_n(\mathbf{r})\,dV,
\end{aligned}
\label{eq:cav_energy_pairing}
\end{equation}
which is Hermitian and positive definite for a lossless medium.  Evaluating $\langle\mathcal{E}_m|\mathcal{H}\mathcal{E}_n\rangle$ with the eigenvalue equation for each mode in turn and subtracting---the same self-adjointness argument used for the waveguide in Eq.~\eqref{eq:flux_orthogonality}---yields
\begin{equation}
(k_{0,n} - k_{0,m})\,\langle\mathcal{E}_m|\mathcal{E}_n\rangle_{\bar{\varepsilon}} = 0,
\label{eq:cav_orthogonality}
\end{equation}
implying real eigenfrequencies and orthogonality of modes with distinct $\omega_n$.  We normalize by $\langle\mathcal{E}_m|\mathcal{E}_n\rangle_{\bar{\varepsilon}} = \delta_{mn}$.

The energy-orthonormal eigenmodes satisfy the closure relation
\begin{equation}
\begin{aligned}
\sum_n
\mathcal{E}_n(\mathbf{r})\,
\mathcal{E}_n^\dagger(\mathbf{r}')\,
\bar{\varepsilon}(\mathbf{r}')
&=
\mathbb{I}_6\,\delta^{(3)}(\mathbf{r} - \mathbf{r}'),
\end{aligned}
\label{eq:cav_closure}
\end{equation}
which resolves the identity in the cavity field space.  Expanding the Green kernel~\eqref{eq:cav_green_def} in this basis gives the spectral representation
\begin{equation}
\begin{aligned}
g(\mathbf{r},\mathbf{r}',\omega)
&=
\sum_n
\frac{
\mathcal{E}_n(\mathbf{r})\,
\mathcal{E}_n^\dagger(\mathbf{r}')
}{
k_{0,n} - k_0 - i0^+
},
\end{aligned}
\label{eq:cav_green_spectral}
\end{equation}
with poles at the cavity resonance frequencies~\cite{novotny2006principles}.  The infinitesimal shift $-i0^+$ in the denominator selects the retarded Green kernel, corresponding to the causal (outgoing) boundary conditions in Eq.~\eqref{eq:cav_green_def}; replacing $-i0^+$ with $+i0^+$ would yield the advanced kernel, which propagates signals backward in time.  One can verify Eq.~\eqref{eq:cav_green_spectral} by acting with $\mathcal{M}$ on the observation coordinate: each eigenvalue factor $k_{0,n} - k_0$ cancels the denominator, leaving $\bar{\varepsilon}\sum_n\mathcal{E}_n\mathcal{E}_n^\dagger$, which reduces to $\mathbb{I}_6\,\delta^{(3)}(\mathbf{r}-\mathbf{r}')$ via the closure relation~\eqref{eq:cav_closure}.

Equation~\eqref{eq:cav_green_spectral} is the cavity analog of the waveguide transverse resolvent derived in Sec.~\ref{sec:wg_green}: both are spectral sums over the eigenmodes of the respective generalized eigenproblem, with the retarded prescription selecting the causal response.

\subsection{Incorporating loss}
The spectral representation~\eqref{eq:cav_green_spectral} was derived for a lossless, closed cavity in which $\mathcal{M}$ is self-adjoint.  Any real cavity, however, is subject to two sources of loss: material absorption ($\bar{\varepsilon}_I \neq 0$), which makes the material tensor non-Hermitian, and radiative decay through open boundaries, which replaces the self-adjoint perfect-wall condition with an outgoing (Sommerfeld) radiation condition.  Either mechanism renders $\mathcal{M}$ non-self-adjoint, so the eigenvalues become complex and the left and right eigenvectors are no longer identical.

In the quasinormal mode (QNM) formalism~\cite{kristensen2014quasinormal,lalanne2018light,franke2020fluctuation, lalanne2019QNM}, one solves the non-Hermitian eigenproblem directly, obtaining complex eigenfrequencies $\tilde{\omega}_n = \omega_n - i\kappa_n/2$ and distinct right and left eigenvectors $\mathcal{E}_n^R$ and $\tilde{\mathcal{E}}_n^L$.  The spectral representation of $g$ is then a biorthogonal expansion,
\begin{equation}
\begin{aligned}
g(\mathbf{r},\mathbf{r}',\omega)
&=
\sum_n
\frac{
\mathcal{E}_n^R(\mathbf{r})\,
(\tilde{\mathcal{E}}_n^L(\mathbf{r}'))^\dagger
}{
\omega - \tilde{\omega}_n
},
\end{aligned}
\label{eq:qnm_green}
\end{equation}
with a regularized normalization that replaces the energy pairing~\eqref{eq:cav_energy_pairing}~\cite{kristensen2014quasinormal,lalanne2018light}.

When the loss is small compared to the mode frequency---the high-$Q$ regime $\kappa_n \ll \omega_n$---the non-Hermitian perturbation can be treated to first order.  The eigenvalue acquires an imaginary part, $k_{0,n} \to k_{0,n} - i\kappa_n/(2c)$, but the eigenvectors are modified only at $O(\kappa/\omega)$ and can be replaced by their lossless counterparts to leading order.  The biorthogonal expansion~\eqref{eq:qnm_green} then collapses to the lossless form~\eqref{eq:cav_green_spectral} with complex poles:
\begin{equation}
\begin{aligned}
g(\mathbf{r},\mathbf{r}',\omega)
&\approx
\sum_n
\frac{
\mathcal{E}_n(\mathbf{r})\,
\mathcal{E}_n^\dagger(\mathbf{r}')
}{
k_{0,n} - k_0 - i\kappa_n/(2c)
}.
\end{aligned}
\label{eq:cav_green_lossy}
\end{equation}
This approximation breaks down when the linewidths become comparable to the mode spacing, $\kappa_n \gtrsim |\omega_n - \omega_{n+1}|$, so that adjacent resonances overlap spectrally and can no longer be treated independently.  It also fails near exceptional points, where two complex eigenvalues and their eigenvectors coalesce, rendering the operator non-diagonalizable~\cite{miri2019exceptional}. In those regimes, either the full biorthogonal QNM expansion~\eqref{eq:qnm_green} or the multi-mode matrix resolvent of Appendix~\ref{sec:coupled_cavities} is required.

\subsection{Uniform lossless waveguide spectral Green function}

We now turn to the second canonical geometry.  The starting point is again the general Green equation~\eqref{eq:cav_green_def},
\begin{equation}
\begin{aligned}
\mathcal{M}_{\mathbf{r}}\,
g(\mathbf{r},\mathbf{r}',\omega)
&=
\mathbb{I}_6\,\delta^{(3)}(\mathbf{r} - \mathbf{r}'),
\end{aligned}
\end{equation}
but now the medium is lossless and translationally invariant along $\hat{\mathbf{z}}$.  Translational invariance allows a Fourier decomposition in $z$,
\begin{equation}
\begin{aligned}
g(\mathbf{r},\mathbf{r}',\omega)
&=
\int \frac{d\beta}{2\pi}\,
g_t(\mathbf{r}_\perp,\mathbf{r}'_\perp;\beta)\,
e^{i\beta(z-z')},
\end{aligned}
\label{eq:wg_green_fourier}
\end{equation}
which reduces the three-dimensional problem to a two-dimensional one at each $\beta$.  Substituting into the Green equation and using $\partial_z \to i\beta$ yields the transverse resolvent equation
\label{sec:wg_green}
\begin{equation}
\begin{aligned}
(\mathcal{M}_t - \beta\,\bar{\mathbf{z}}\times)\,
g_t(\mathbf{r}_\perp,\mathbf{r}'_\perp;\beta)
&=
\mathbb{I}_6\,\delta^{(2)}(\mathbf{r}_\perp - \mathbf{r}'_\perp),
\end{aligned}
\label{eq:transverse_resolvent_eq}
\end{equation}
where $\mathcal{M}_t = \mathcal{H}_t - k_0\bar{\varepsilon}$ is the transverse Maxwell operator of Sec.~\ref{sec:waveguide_formalism}.  This is the waveguide counterpart of the cavity Green equation: both invert the Maxwell operator, but here the eigenvalue parameter is the propagation constant $\beta$ rather than the frequency.

Expanding $g_t$ in the flux-orthonormal eigenmodes of the transverse eigenproblem~\eqref{eq:wg_eigenproblem}---the same modes derived in Sec.~\ref{sec:waveguide_formalism}---gives the spectral representation~\cite{Arfken, sakoda2004optical}
\begin{equation}
\begin{aligned}
g_t(\mathbf{r}_\perp,\mathbf{r}'_\perp;\beta)
&=
\sum_n
\frac{
s_n\,\mathcal{E}_n(\mathbf{r}_\perp)\,
\mathcal{E}_n^\dagger(\mathbf{r}'_\perp)
}{
\beta_n - \beta
}\,(\bar{\mathbf{z}}\times)
\\
&\quad+
\int
\frac{
s(\beta')\,\mathcal{E}_{\beta'}(\mathbf{r}_\perp)\,
\mathcal{E}_{\beta'}^\dagger(\mathbf{r}'_\perp)
}{
\beta' - \beta
}\,(\bar{\mathbf{z}}\times)\,d\beta',
\end{aligned}
\label{eq:transverse_resolvent}
\end{equation}
where the first sum runs over the discrete guided modes and the second integral over the radiation-continuum contribution~\cite{chew1995waves1,felsen1994radiation}.  This is the direct analog of the cavity spectral Green function~\eqref{eq:cav_green_spectral}: both are spectral sums over the eigenmodes of their respective generalized eigenproblems, with the eigenvalue ($\beta_n$ or $k_{0,n}$) appearing in the denominator and the appropriate bilinear form ($(\bar{\mathbf{z}}\times)$ or $\bar{\varepsilon}$) providing the weight.

As in the cavity case, the causal boundary condition is enforced by an infinitesimal pole shift.  For the waveguide, the prescription is $1/(\beta_n - \beta) \to 1/(\beta_n - \beta - i0^+s_n)$, which displaces forward-mode poles ($s_n = +1$) into the upper half of the complex $\beta$-plane and backward-mode poles ($s_n = -1$) into the lower half-plane, ensuring that each mode propagates away from the source.  This is the waveguide analog of the retarded $-i0^+$ shift in Eq.~\eqref{eq:cav_green_spectral}: both enforce causality, but the cavity prescription acts in the frequency plane while the waveguide prescription acts in the propagation-constant plane.

To recover the real-space Green kernel we perform the inverse Fourier transform in $\beta$, closing the contour in the upper half-plane for $z > z'$ and in the lower half-plane for $z < z'$.  Each guided-mode pole contributes a residue only when it lies inside the chosen contour: the forward pole ($s_n = +1$, upper half-plane) contributes only for $z > z'$, and the backward pole ($s_n = -1$, lower half-plane) only for $z < z'$.  The result is the guided-mode Green kernel
\begin{multline}
g_\mathrm{guided}(\mathbf{r},\mathbf{r}')
=
\sum_n s_n\,\Theta\!\bigl(s_n(z\!-\!z')\bigr)
\\
\times
\mathcal{E}_n(\mathbf{r}_\perp)\,
\mathcal{E}_n^\dagger(\mathbf{r}'_\perp)\,
(\bar{\mathbf{z}}\times)\,
e^{i\beta_n(z-z')},
\label{eq:guided_green_app}
\end{multline}
where $\Theta$ is the Heaviside step function.  Each mode contributes only on the side of the source consistent with its propagation direction: a forward mode ($s_n = +1$) propagates the field to the right of the source, while a backward mode ($s_n = -1$) propagates it to the left.

\section{Composite nanophotonic systems}
\label{app:composite_moved}
%%%%%%%%%%%%%%%%%%%%%%%%%%%%%%%%%

% \begin{figure}
%     \centering
%     \includegraphics[width=1.\linewidth]{figures/Coupled cavities and ring resonator WB.pdf}
%     \caption{Composite systems}
%     \label{fig:composite systems}
% \end{figure}
%%%%%%%%%%%%%%%%%%%%%%%%%%%%%%%%%%%%%%%%%%%%%
\subsection{Overview}

The single-mode cavity and uniform waveguide of Sec.~\ref{sec:applications} are the two building blocks of nanophotonic design. Any real device, like coupled microring resonators, photonic-crystal defect pairs, arrays of quantum dots in a waveguide~\cite{asenjo-garcia2017atom,hood2016atom, goban2015superradiance}, are fundamentally a composition of these elements. The Green-function formalism accommodates such systems without modifying the quantization technique. One constructs an approximate $g$ for the composite structure and substitutes it into the same scattering matrix~\eqref{eq:S-matrix} and quantum input--output relation~\eqref{eq:quantum_io}. Here we will explore two regimes, one having a strong coupling between the  discrete modes of N-coupled cavities and the other regime of weak coupling between the discrete mode of cavity and continuum modes of waveguide.

\subsection{Coupled Cavities}
\label{sec:coupled_cavities}
%%%%%%%%%%%%%%%%%%%%%%%%%%%%%%%%%%%%%%%%%%%


% In this section, we treat the important case of $N$ coupled cavity modes. And in the following section, Sec.~\ref{sec:composite_main} we extend the analysis to cavity--waveguide composites, where the waveguide continuum dresses the cavity poles through a Dyson self-energy~\cite{kristensen2014quasinormal}.

Consider two cavity modes $\mathcal{E}_1$ and $\mathcal{E}_2$ with complex resonance frequencies $\tilde{\omega}_j = \omega_j - i\kappa_j/2$. When the two modes interact---whether through direct spatial overlap~\cite{Hartmann2008QuantumManyBody}, photon tunneling~\cite{Knight1997Evanescentcoupling}, or radiative mixing~\cite{Horng2019RadiativeCoupling} via a shared environment---the Green function cannot be written as a sum of independent single-mode poles. The correct low-rank approximation retains the off-diagonal propagation channels by projecting $g$ onto the two-mode subspace:
\begin{equation}
\begin{aligned}
g(\mathbf{r},\mathbf{r}',\omega)
&\approx
\sum_{\mu,\nu=1}^{2}
\mathcal{E}_\mu(\mathbf{r})\,
\bigl[D^{-1}(\omega)\bigr]_{\mu\nu}\,
\mathcal{E}_\nu^\dagger(\mathbf{r}'),
\end{aligned}
\label{eq:two_mode_green}
\end{equation}
where $D(\omega)$ is the $2\times 2$ dynamical matrix
\begin{equation}
D(\omega)
=
\begin{pmatrix}
\omega - \tilde\omega_1 & -V_{12}
\\
-V_{21} & \omega - \tilde\omega_2
\end{pmatrix}.
\label{eq:dynamical_matrix}
\end{equation}
Here $V_{12}$ is the coupling between the two cavity modes. For a reciprocal medium, $V_{12} = V_{21} \equiv J$, and the inverse is
\begin{equation}
D^{-1}(\omega)
=
\frac{1}{\mathcal{D}(\omega)}
\begin{pmatrix}
\omega - \tilde\omega_2 & J
\\
J & \omega - \tilde\omega_1
\end{pmatrix},
\label{eq:D_inverse}
\end{equation}
with $\mathcal{D}(\omega) = (\omega-\tilde\omega_1)(\omega-\tilde\omega_2) - V^2$.  Substituting into~\eqref{eq:two_mode_green}, the Green kernel becomes
\begin{multline}
g(\mathbf{r},\mathbf{r}',\omega)
\approx
\frac{1}{\mathcal{D}(\omega)}
\bigl[
(\omega-\tilde\omega_2)\,\mathcal{E}_1\mathcal{E}_1^\dagger
\\
+(\omega-\tilde\omega_1)\,\mathcal{E}_2\mathcal{E}_2^\dagger
+V\bigl(\mathcal{E}_1\mathcal{E}_2^\dagger
+\mathcal{E}_2\mathcal{E}_1^\dagger\bigr)
\bigr],
\label{eq:two_mode_green_explicit}
\end{multline}
where we abbreviate $\mathcal{E}_\mu \equiv \mathcal{E}_\mu(\mathbf{r})$ and $\mathcal{E}_\nu^\dagger \equiv \mathcal{E}_\nu^\dagger(\mathbf{r}')$.  The off-diagonal terms, proportional to $V$, are the inter-cavity propagation channels: excitation injected into one mode can propagate into the other before returning to the observation point.

The poles of the coupled Green function are the zeros of $\mathcal{D}(\omega)$:
\begin{equation}
\begin{aligned}
\omega_\pm
&=
\frac{\tilde\omega_1 + \tilde\omega_2}{2}
\pm
\sqrt{
V^2
+ \left(
\frac{\tilde\omega_1 - \tilde\omega_2}{2}
\right)^2
}.
\end{aligned}
\label{eq:hybridized_poles}
\end{equation}
The bare complex frequencies $\tilde\omega_1,\tilde\omega_2$ are replaced by the dressed frequencies $\omega_\pm$.  In the hybridized-mode basis, the Green function takes the diagonal form
\begin{equation}
\begin{aligned}
g(\mathbf{r},\mathbf{r}',\omega)
&\approx
\frac{
\mathcal{F}_+(\mathbf{r})\,
\bar{\mathcal{F}}_+^\dagger(\mathbf{r}')
}{
\omega - \omega_+
}
\\
&\quad+
\frac{
\mathcal{F}_-(\mathbf{r})\,
\bar{\mathcal{F}}_-^\dagger(\mathbf{r}')
}{
\omega - \omega_-
},
\end{aligned}
\label{eq:hybridized_green}
\end{equation}
where $\mathcal{F}_\pm$ and $\bar{\mathcal{F}}_\pm$ are the right and left eigenvectors of $D(\omega)$, which differ for a non-Hermitian dynamical matrix.  The bare-basis representation~\eqref{eq:two_mode_green} is more convenient for matching to bare-cavity parameters, while the hybridized form~\eqref{eq:hybridized_green} makes the pole structure manifest.

When the two cavities radiate into a common bath or share a continuum channel, the coupling acquires an imaginary part.  The most general two-mode effective Hamiltonian is
\begin{equation}
H_\mathrm{eff}
=
\begin{pmatrix}
\omega_1 - i\kappa_1/2 & J - i\Gamma_{12}/2
\\
J - i\Gamma_{21}/2 & \omega_2 - i\kappa_2/2
\end{pmatrix},
\label{eq:Heff_coupled}
\end{equation}
so that $D(\omega) = \omega I - H_\mathrm{eff}$.  The real part $J$ represents coherent photon tunneling, while the imaginary part $\Gamma_{12}$ represents dissipative coupling through a shared loss channel.  A consequence of this non-Hermitian structure is that coupling not only splits the real parts of $\omega_\pm$ but can also redistribute the linewidths: one hybridized mode may become broader while the other narrows.

The construction extends immediately to $N$ coupled resonances.  The general $N$-mode projected Green function is
\begin{equation}
\begin{aligned}
g(\mathbf{r},\mathbf{r}',\omega)
&\approx
\sum_{\mu,\nu=1}^{N}
\mathcal{E}_\mu(\mathbf{r})\,
\bigl[(\omega I - H_\mathrm{eff})^{-1}\bigr]_{\mu\nu}\,
\mathcal{E}_\nu^\dagger(\mathbf{r}').
\end{aligned}
\label{eq:N_mode_green}
\end{equation}
with $H_\mathrm{eff} \in \mathbb{C}^{N\times N}$ encoding all coherent and dissipative couplings among the $N$ modes.  For $N=1$ this recovers the single-mode approximation~\eqref{eq:cav_single_mode}; for $N=2$ it reduces to~\eqref{eq:two_mode_green}.  Substituted into the scattering matrix~\eqref{eq:S-matrix} and the quantum input--output relation~\eqref{eq:quantum_io}, Eq.~\eqref{eq:N_mode_green} yields the $N$-mode quantum scattering description of the coupled-cavity system, with the Langevin noise fixed by the optical theorem as before.

\paragraph{General scattering matrix for the coupled cavity system:} For a single input and single output channel connecting the coupled cavity system the general scattering matrix has can be deduced using the equation~\eqref{eq:two_mode_green_explicit} and equation~\eqref{eq:S-matrix},
\begin{equation}
    \begin{split}
    S_{mn}
    &=
    \frac{1}{\mathcal{D}(\omega)}
    \Big(
    \Delta_2 d_{m1} c_{1n}
    + \Delta_1 d_{m2}c_{2n}
    \\
    &\quad
    + V d_{m2}c_{1n}
    + V d_{m2} c_{2n}
    \Big)
\end{split}
    \label{eq: general_coupled_cavity_scattering_matrix}
\end{equation}
where $\Delta_{i} = \omega - \tilde\omega_i$ and $d_{mi}$ is the output-overlap integral for the $i^{\text{th}}$ cavity mode to the $m^{\text{th}}$ waveguide mode and $c_{in}$ is the input-overlap integral for the $i^{\text{th}}$ cavity mode to the $n^{\text{th}}$ waveguide mode.


%%%%%%%%%%%%%%%%%%%%%%%%%%%%%%%%%%%%%%%%%%%%
\subsection{Cavity--Waveguide Composites}
\label{sec:composite_main}
%%%%%%%%%%%%%%%%%%%%%%%%%%%%%%%%%%%%%%%%%%%%

Section~\ref{sec:coupled_cavities} treated coupled discrete resonances. Now we bring our focus to the complementary case of one or more cavity modes interacting with a waveguide continuum; the geometry underlying side-coupled ring resonators~\cite{Zare2024RingResonator}, photonic-crystal defect modes, and cavity QED in a waveguide~\cite{Coles2014dot_waveguide_cavity}.

% \paragraph{Self-energy and Markov limit.}
% \label{sec:cav_wg}

Consider a discrete cavity resonance coupled to a waveguide continuum. Similar to the coupled cavity case, the first-order formalism gives a composite Green function of the form
\begin{multline}
g(\mathbf r, \mathbf r' , \omega)
=
\sum_{k}
\frac{\omega}{\omega_k-\omega}\,
\mathcal{E}_{k}(\mathbf{r})\,
\mathcal{E}^\dagger_k(\mathbf{r}')
\\
+
\sum_{k}
\frac{\omega^2 V_{kc}}{\omega_k-\omega}\,
\frac{
\mathcal{E}_{k}(\mathbf{r})\,
\mathcal{E}^\dagger_c(\mathbf{r}')
}{
(\omega_c-\omega)-\Sigma(\omega)
}
\\
+
\frac{\omega}{
(\omega_c-\omega)-\Sigma(\omega)
}\,
\mathcal{E}_{c}(\mathbf{r})\,
\mathcal{E}^\dagger_c(\mathbf{r}')
\end{multline}
where the subscripts $k$ and $c$ represent the waveguide and cavity modes, respectively. The first term on the RHS is the bare waveguide modal form, the second term represents the cross-coupling between the cavity mode and the waveguide continuum, and the third one is the dressed cavity modes. The dressing due to the waveguide continuum enters through the frequency-dependent self-energy term $\Sigma(\omega)$ defined as,
\begin{equation}
\begin{aligned}
\Sigma(\omega)
&=
\lim_{\eta \to 0^+}
\sum_{k}
\frac{\omega^2|V_{k,c}|^2}{
\omega_k -\omega +i\eta
}
\end{aligned}
\end{equation}
where $V_{k,c} = \bra{\mathcal{E}_k(\mathbf{r})}\Delta\bar{\varepsilon}_c(\mathbf{r})\ket{\mathcal{E}_c(\mathbf r)}$ is the interaction term~\cite{HughesCoupledCavityQED}. 

The self-energy term also gives information on how the waveguide continuum affects the decay of the composite system and the Lamb shift in the cavity resonance. By converting $\sum_{k} \to \frac{L}{2\pi}\int_{-\infty}^{\infty} \dd k$ and $\dd k \to \dd \omega_k/v_g$ yields,
\begin{equation}
    \begin{split}
    \Sigma(\omega)
    &=
    \lim_{\eta \to 0^+}
    \int_{0}^\infty
    \frac{\omega^2 J(\omega_k)}{
    \omega_k - \omega + i\eta
    }\,
    \dd \omega_k
    \end{split}
\end{equation}
where $\rho(\omega_k) = L/(\pi v_g)$ is the one dimensional spectral density, and $J(\omega) = |V_{k,c}|^2 \rho(\omega_k)$ . Now, applying the Sokhotski-Plemelj theorem,
\begin{equation}
    \begin{split}
    \Sigma(\omega)
    &=
    i\pi\omega^2 J(\omega)
    \\
    &\quad
    + \text{P.V}
    \int_{0}^\infty
    \frac{\omega^2 J(\omega_k)}{
    \omega_k-\omega
    }\,
    \dd \omega_k
    \end{split}
\end{equation}
% To extract that, one can convert the summation to an integral of the modes, for waveguide of length $L$, $\sum_{k} \to \frac{L}{2\pi}\int_{-\infty}^{\infty} \dd k$ and $\dd k \to \dd \omega_k/v_g$
% \begin{equation}
%     \begin{split}
%     \Sigma(\omega) = \lim_{\eta \to 0^+} \int_{-\infty}^\infty \frac{\omega^2|V_{k,c}|^2}{\omega_k - \omega + i\eta}\frac{L}{2\pi v_g} \dd \omega_k\\
%     =\lim_{\eta \to 0^+} \int_{0}^\infty \frac{\omega^2|V_{k,c}|^2}{\omega_k - \omega + i\eta}\rho(\omega_k) \dd \omega_k\\
%     =\lim_{\eta \to 0^+} \int_{0}^\infty \frac{\omega^2 J(\omega_k)}{\omega_k - \omega + i\eta} \dd \omega_k
%     \end{split}
% \end{equation}
% where $\rho(\omega_k) = L/(\pi v_g)$ is the one dimensional spectral density. Now, applying Sokhotski-Plemelj theorem, 
% \begin{equation}
%     \begin{split}
%     \Sigma(\omega) =  \int_{0}^\infty \omega^2 J(\omega_k)i\pi\delta(\omega_k -\omega) \dd \omega_k\\
%     +\text{P.V} \int_{0}^\infty \frac{\omega^2 J(\omega_k)}{(\omega_k-\omega)} \dd \omega_k\\
%     =i\pi\omega^2 J(\omega)  + \text{P.V} \int_{0}^\infty  \frac{\omega^2 J(\omega_k)}{(\omega_k-\omega)} \dd \omega_k
%     \end{split}
% \end{equation}
we get the decay rate as $\Gamma = \omega^2 J(\omega)$ and the principal value denoting the Lamb shift~\cite{scully1997quantum}. 

\paragraph{Scattering matrix for cavity-waveguide composite:} Typically, the waveguide's effect on the cavity is such that the cavity linewidth is very small compared to the self-energy term, rendering the interaction between the waveguide continuum and cavity mode to be effectively constant, only a function of cavity resonance, also known as the Markov approximation. So, $\Sigma(\omega_c) = i\Gamma + \Delta$ is effectively a constant over the input-output modes of interest, for $n^{\mathrm th}$ input mode, the outcoupling $m^{\mathrm th}$ mode will be defined by the scattering matrix, under projections with $\bar{\varepsilon}_t \mathcal{E}_{m,n}$,
\begin{equation}
\begin{aligned}
S_{mn}
&=
\frac{\omega}{\omega_m - \omega}\delta_{mn}
\\
&\quad+
\frac{
\omega^2 V_{m,c}V_{c,n}\delta_{mn}
}{
(\omega_m-\omega)
(\omega_c -\omega -\Delta-i\Gamma)
}
\end{aligned}
\end{equation}
where $V_{m,c} = \bra{\mathcal{E}_m(\mathbf r)}\Delta\bar{\varepsilon}_c(\mathbf r) \ket{\mathcal{E}_{c}(\mathbf r)}$, $V_{c,n} = \bra{\mathcal{E}_c(\mathbf r)}\Delta\bar{\varepsilon}_c(\mathbf r) \ket{\mathcal{E}_{n}(\mathbf r)}$ and $\bar{\varepsilon}_t = \bar{\varepsilon}_b + \Delta\bar{\varepsilon}_w +\Delta\bar{\varepsilon}_c$.



% Before the two subsystems interact, the Green function decomposes as
% \begin{equation}
% g_0(\mathbf{r},\mathbf{r}',\omega) = g_\mathrm{wg}^{(0)}(\mathbf{r},\mathbf{r}',\omega) + \frac{\mathcal{E}_c(\mathbf{r})\,\mathcal{E}_c^\dagger(\mathbf{r}')}{\omega - \tilde\omega_c},
% \label{eq:bare_decomp}
% \end{equation}
% where $g_\mathrm{wg}^{(0)}$ is the bare waveguide Green function from Sec.~\ref{sec:wg_green} and $\tilde\omega_c = \omega_c - i\kappa_i/2$ is the intrinsic cavity frequency.  The coupling is treated exactly by a Dyson equation~\cite{Ge2014QNM}: letting $W$ denote the coupling operator between the cavity and waveguide subspaces, the full Green function satisfies $g = g_0 + g_0\,W\,g$.  Projecting onto the cavity subspace yields the dressed cavity Green function
% \begin{equation}
% G_c(\omega) = \frac{1}{\omega - \omega_c - \Sigma(\omega)},
% \label{eq:dressed_cavity}
% \end{equation}
% where the self-energy
% \begin{equation}
% \Sigma(\omega) = \sum_n \frac{|V_{cn}|^2}{\omega - \omega_n + i0^+}
% \label{eq:self_energy}
% \end{equation}
% encodes the effect of the waveguide continuum on the cavity, with $V_{cn}$ the coupling amplitude of the cavity to the $n^{\text{th}}$ waveguide mode. The waveguide contributes a branch-cut continuum rather than simple isolated poles, like a cavity; eliminating the branch cut dresses the cavity poles with a frequency-dependent self-energy. The quantum input--output relation~\eqref{eq:quantum_io} remains unchanged, only the representation of the Green function changes. Using the Sokhotski--Plemelj identity, the self-energy separates into a Lamb-shift-like frequency renormalization and a waveguide-induced decay rate,
% \begin{equation}
% \Sigma(\omega) = \Delta_\mathrm{L}(\omega) - i\frac{\Gamma_\mathrm{wg}(\omega)}{2},
% \label{eq:self_energy_split}
% \end{equation}
% where $\Delta_\mathrm{L}(\omega) = \mathcal{P}\sum_n |V_{cn}|^2/(\omega - \omega_n)$ and
% \begin{equation}
% \Gamma_\mathrm{wg}(\omega) = 2\pi \sum_\alpha \frac{|V_{c,k_\alpha}|^2}{|v_g(k_\alpha)|}, \qquad \omega_{k_\alpha} = \omega.
% \label{eq:gamma_wg}
% \end{equation}
% The factor $1/|v_g|$ is the waveguide density of states: a slow-light mode enhances the cavity decay rate, in direct analogy with the Purcell effect.

% Solving the Dyson equation for the full Green function gives the cavity-mediated correction to the bare waveguide propagator,
% \begin{multline}
% g(\omega) \approx g_\mathrm{wg}^{(0)}(\omega) \\
% + g_\mathrm{wg}^{(0)}(\omega)\,W\,G_c(\omega)\,W^\dagger\,g_\mathrm{wg}^{(0)}(\omega),
% \label{eq:full_cav_wg_green}
% \end{multline}
% a rank-one (separable) modification of $g_\mathrm{wg}^{(0)}$ whose pole is the dressed cavity resonance.






%%%%%%%%%%%%%%%%%%%%%%%%%%%%%%%%%

\section{Coincident-point regularization and single-emitter self-energy}
\label{app:single_emitter_regularization}

This appendix records the only extra step required when the Green kernel is evaluated at the position of a point emitter.  The field generated by a point dipole contains the usual singular vacuum self-field, so the coincident-point Green function must be interpreted with the standard principal-value prescription before it is inserted into the single-emitter self-energy~\cite{Yaghjian1980, ChewWavesandFields, Niewenhuizen1992ResonantPointScatterers, Vries1998PointScatterersforClassicalWaves}.

For a two-level emitter at $\mathbf r_A$ with transition dipole six-vector $\mathcal D$, the positive-frequency dipole current is proportional to $\mathcal D\hat\sigma_A$.  In frequency space the emitter-generated field at the emitter position is therefore determined by the coincident Green kernel,
\begin{equation}
\hat{\mathcal E}_{\rm self}(\mathbf r_A,\omega)
=
\frac{\omega}{c}\,
 g(\mathbf r_A,\mathbf r_A,\omega)\mathcal D\,\hat\sigma_A(\omega),
\end{equation}
and the projected self-interaction is
\begin{equation}
\Sigma_A(\omega)
=
\frac{\omega}{\hbar c}\,
\mathcal D^\dagger
 g_{\rm reg}(\mathbf r_A,\mathbf r_A,\omega)
\mathcal D .
\label{eq:app_single_emitter_self_energy}
\end{equation}
Here $g_{\rm reg}$ denotes the coincident-point Green function after the singular electrostatic part has been removed.\ankit{I don't get this point}

\subsection{Principal-value prescription}
\label{appsubsec: decay_dynamics_emitter}

The coincident Green kernel may be separated schematically as
\begin{equation}
 g(\mathbf r,\mathbf r',\omega)
=
 g_{\rm sing}^{\rm vac}(\mathbf r,\mathbf r',\omega)
+
 g_{\rm reg}(\mathbf r,\mathbf r',\omega),
\label{eq:app_g_sing_reg_split}
\end{equation}
where $g_{\rm sing}^{\rm vac}$ contains the divergent local vacuum contribution and $g_{\rm reg}$ is finite at $\mathbf r=\mathbf r'$.  Equivalently, the real part of the singular self-field is understood as a principal value and absorbed into the definition of the physical transition frequency.  With the sign convention used in the main text,
\begin{equation}
\Sigma_A(\omega_A)
=
\Delta_A-i\frac{\Gamma_A}{2},
\label{eq:app_self_energy_split}
\end{equation}
where
\begin{equation}
\Delta_A
=
\operatorname{Re}\Sigma_A(\omega_A),
\label{eq:app_lamb_gamma_from_sigma}
\end{equation}
and $\Gamma_A$ denotes the positive decay rate.  The absorbed principal-value contribution only shifts the bare transition frequency.  The imaginary part is finite and fixes the physical decay rate through the optical theorem.

Using Eq.~\eqref{eq:app_single_emitter_self_energy}, the projected local density of states gives
\begin{equation}
\Gamma_A
=
\frac{2\omega_A}{\hbar c}\,
\operatorname{Im}
\left[
\mathcal D^\dagger
 g(\mathbf r_A,\mathbf r_A,\omega_A)
\mathcal D
\right],
\label{eq:app_gamma_ldos}
\end{equation}
again with the Fourier and Green-function sign convention of the main text.  If the opposite retarded-frequency convention is used, the sign of $\operatorname{Im}g$ and hence the last equality changes, while the positive rate $\Gamma_A$ is unchanged.

The same prescription applies before any Markov or low-saturation approximation.  Regularization is a statement about the local electromagnetic self-field; the subsequent approximations only decide whether $\Sigma_A(\omega)$ is evaluated at a fixed frequency or retained as a frequency-dependent memory kernel.

\section{Pole--zero determinant identity and single-channel simplifications}
\label{app:determinant_pole_zero}

In this appendix we collect the explicit drive vectors and noise operators of the collective response, give the eigenmode expansion of the dressed scattering matrix, and then derive the determinant form and the conditions under which it reduces to a product over collective eigenvalues.  The derivation is purely algebraic up to the final simplification, which requires a special single-channel structure of the Green function.

\subsection{Drive vectors, dressed noise, and eigenmode expansion}
\label{app:collective_drive_eigen}

We first record the explicit single-emitter couplings used in Sec.~\ref{subsec:modal_response_low_saturation}.  The channel normalization is $\alpha=\sqrt{2\pi\varepsilon_0/\hbar k_0}$, converting a flux-projected field amplitude into a dimensionless channel operator.  The emitter-to-output coupling is
\begin{equation}
\begin{aligned}
g_{{\rm out},m}(\omega)
&=
\alpha k_0
\int_{S_{\rm out}}
\mathcal E_m^{{\rm out}\dagger}(\mathbf r,\omega)\,
(\bar n_{\rm out}\times)
\\
&\quad
g(\mathbf r,\mathbf r_A,\omega)\,
\mathcal D \,dS .
\end{aligned}
\label{eq:g_out_single_new}
\end{equation}
The background field driving the emitter is the sum of the boundary-driven field and the Langevin field,
\begin{equation}
\begin{aligned}
\hat{\mathcal E}_0(\mathbf r_A,\omega)
&=
-i\int_{S_{\rm in}}
g(\mathbf r_A,\mathbf s,\omega)\,
(\bar n_{\rm in}\times)
\\
&\quad
\hat{\mathcal E}_{\rm in}(\mathbf s,\omega)\,dS
\\
&\quad
+ k_0\int_V
g(\mathbf r_A,\mathbf r',\omega)\,
\hat{\mathcal P}_N(\mathbf r',\omega)\,dV',
\end{aligned}
\label{eq:background_field_at_emitter_new}
\end{equation}
and its dipole projection $\tfrac{1}{\hbar}\mathcal D^\dagger\hat{\mathcal E}_0=\sum_n g_{{\rm in},n}\hat a_n+\hat F_N$ defines the input-to-emitter coupling
\begin{equation}
\begin{aligned}
g_{{\rm in},n}(\omega)
&=
-\frac{i}{\hbar\alpha}\,
\mathcal D^\dagger
\int_{S_{\rm in}}
g(\mathbf r_A,\mathbf s,\omega)\,
(\bar n_{\rm in}\times)
\\
&\quad
\mathcal E_n^{\rm in}(\mathbf s,\omega) \,dS ,
\end{aligned}
\label{eq:g_in_single_new}
\end{equation}
and the absorption-noise drive
\begin{equation}
\begin{aligned}
\hat F_N(\omega)
&=
\frac{k_0}{\hbar}\,
\mathcal D^\dagger
\int_V
g(\mathbf r_A,\mathbf r',\omega)\,
\hat{\mathcal P}_N(\mathbf r',\omega) \,dV'.
\end{aligned}
\label{eq:FN_single_new}
\end{equation}

The multi-emitter case follows by replacing the scalar couplings with vectors.  The dipole-projected background drive on emitter $i$ separates into a boundary-input part and a material-noise part,
\begin{equation}
[\hat{\mathbf F}_{\rm in}(\omega)]_i + [\hat{\mathbf F}_{N}(\omega)]_i
=
\frac{1}{\hbar}\, \mathcal D_i^\dagger \hat{\mathcal E}_0(\mathbf r_i,\omega).
\label{eq:N_drive_total}
\end{equation}
The boundary-input contribution is $[\hat{\mathbf F}_{\rm in}(\omega)]_i = \sum_n [\mathbf g_{{\rm in},n}(\omega)]_i\, \hat a_n(\omega)$, with the input-to-emitter coupling vector
\begin{equation}
\begin{aligned}
[\mathbf g_{{\rm in},n}(\omega)]_i
&=
-\frac{i}{\hbar\alpha}\,
\mathcal D_i^\dagger
\int_{S_{\rm in}}
g(\mathbf r_i,\mathbf s,\omega)\,
(\bar n_{\rm in}\times)
\\
&\quad
\mathcal E_n^{\rm in}(\mathbf s,\omega) \,dS ,
\end{aligned}
\label{eq:app_g_in_vec_new}
\end{equation}
and the material-noise drive is
\begin{equation}
\begin{aligned}
[\hat{\mathbf F}_{N}(\omega)]_i
&=
\frac{k_0}{\hbar}\,
\mathcal D_i^\dagger
\int_V
g(\mathbf r_i,\mathbf r',\omega)\,
\hat{\mathcal P}_N(\mathbf r',\omega) \,dV'.
\end{aligned}
\label{eq:app_N_FN_vec}
\end{equation}
Solving the collective linear system gives the non-Markovian response
\begin{equation}
\begin{aligned}
\hat{\boldsymbol\sigma}(\omega)
&=
M^{-1}(\omega)
\left[
\sum_n
\mathbf g_{{\rm in},n}(\omega)\hat a_n(\omega)
+ \hat{\mathbf F}_{N}(\omega)
\right],
\end{aligned}
\label{eq:app_N_sigma_solution}
\end{equation}
and substituting into the modal output relation,
\begin{equation}
\begin{aligned}
\hat b_m(\omega)
&=
\sum_n
\left[
S_{mn}(\omega)
+ \mathbf g_{{\rm out},m}^{T}(\omega)
M^{-1}(\omega)
\mathbf g_{{\rm in},n}(\omega)
\right]\hat a_n(\omega)
\\
&\quad
+ \hat\xi_m(\omega)
+ \mathbf g_{{\rm out},m}^{T}(\omega)
M^{-1}(\omega)
\hat{\mathbf F}_{N}(\omega).
\end{aligned}
\label{eq:app_N_output_substituted}
\end{equation}
The dressed noise operator is therefore
\begin{equation}
\begin{aligned}
\hat\xi_m^{(N)}(\omega)
&=
\hat\xi_m(\omega)
+ \mathbf g_{{\rm out},m}^{T}(\omega)
M^{-1}(\omega)
\hat{\mathbf F}_{N}(\omega),
\end{aligned}
\label{eq:app_N_dressed_noise}
\end{equation}
whose two terms are correlated because both are projections of the same Langevin field $\hat{\mathcal P}_N$: the first is material noise propagated directly to the output, the second is material noise that drives the emitters and is then re-radiated into the output channel.

Diagonalizing the collective matrix as $M(\omega) = \sum_\alpha \Lambda_\alpha(\omega)\, \mathbf u_\alpha \mathbf v_\alpha^\dagger$, with right and left eigenvectors $\mathbf u_\alpha$, $\mathbf v_\alpha$, gives $M^{-1}(\omega) = \sum_\alpha \mathbf u_\alpha\mathbf v_\alpha^\dagger / \Lambda_\alpha(\omega)$, so the dressed scattering matrix becomes a sum of one resonance per collective mode,
\begin{equation}
\begin{aligned}
S_{mn}^{(N)}(\omega)
&=
S_{mn}(\omega)
+ \sum_\alpha
\frac{
\left[ \mathbf g_{{\rm out},m}^{T} \mathbf u_\alpha \right]
\left[ \mathbf v_\alpha^\dagger \mathbf g_{{\rm in},n} \right]
}{
\Lambda_\alpha(\omega)
}.
\end{aligned}
\label{eq:dressed_S_N_modal_new}
\end{equation}
Each collective mode contributes a resonance to the measured transmission only if it overlaps both the input-drive vector $\mathbf g_{{\rm in},n}$ and the output-radiation vector $\mathbf g_{{\rm out},m}$; a mode can be long-lived but nearly invisible if it is weakly driven or weakly outcoupled, while a superradiant mode that overlaps strongly with the measured channels produces a broad spectral feature.

\subsection{Determinant identity}
\label{app:determinant_identity}

Consider one selected input channel $n$ and one selected output channel $m$.  The collective emitter input--output result derived in the main text gives
\begin{equation}
\begin{aligned}
S_{mn}^{(N)}(\omega)
&=
S_{mn}(\omega)
+ \mathbf g_{{\rm out},m}^{T}(\omega)
M^{-1}(\omega)
\mathbf g_{{\rm in},n}(\omega).
\end{aligned}
\label{eq:app_SN_scalar}
\end{equation}
Here $S_{mn}$ is the passive photonic transmission amplitude in the absence of the emitters, $M$ is the $N\times N$ inverse collective susceptibility, and $\mathbf g_{{\rm in},n}$, $\mathbf g_{{\rm out},m}$ are $N$-component vectors describing the input-to-emitter and emitter-to-output propagation.  Define
\begin{equation}
T(\omega)\equiv S_{mn}(\omega), \qquad T_N(\omega)\equiv S_{mn}^{(N)}(\omega),
\label{eq:app_T_defs}
\end{equation}
so that
\begin{equation}
T_N
=
T+ \mathbf g_{\rm out}^{T}M^{-1}\mathbf g_{\rm in}.
\label{eq:app_TN}
\end{equation}
We first assume $T(\omega)\neq0$ and $M(\omega)$ invertible.  These restrictions may be relaxed afterward by analytic continuation, except at genuine pole--zero singularities.  Dividing Eq.~\eqref{eq:app_TN} by $T$ gives
\begin{equation}
\begin{aligned}
\frac{T_N}{T}
&=
1+
\frac{1}{T}
\mathbf g_{\rm out}^{T}
M^{-1}
\mathbf g_{\rm in}.
\end{aligned}
\label{eq:app_T_ratio}
\end{equation}
The matrix determinant lemma states that for an invertible matrix $M$,
\begin{equation}
\det(M+\mathbf u\mathbf v^T)
=
\det M \left( 1+\mathbf v^T M^{-1}\mathbf u \right).
\label{eq:app_det_lemma}
\end{equation}
Taking $\mathbf u=\mathbf g_{\rm in}$ and $\mathbf v^T=\mathbf g_{\rm out}^{T}/T$, we obtain
\begin{equation}
\begin{aligned}
\frac{T_N}{T}
&=
\frac{
\det\!\left[
M+
\dfrac{\mathbf g_{\rm in}\mathbf g_{\rm out}^{T}}{T}
\right]
}{
\det M
}.
\end{aligned}
\label{eq:app_det_ratio_M}
\end{equation}
Equivalently, with the sign convention used in the main text, define the rank-one matrix
\begin{equation}
\begin{aligned}
\mathsf s^{(mn)}(\omega)
&\equiv
-\frac{
\mathbf g_{{\rm in},n}(\omega)
\mathbf g_{{\rm out},m}^{T}(\omega)
}{
S_{mn}(\omega)
}.
\end{aligned}
\label{eq:app_s_def}
\end{equation}
Then
\begin{equation}
M-\mathsf s^{(mn)}
=
M+ \frac{ \mathbf g_{{\rm in},n} \mathbf g_{{\rm out},m}^{T} }{ S_{mn} },
\end{equation}
and the determinant identity becomes
\begin{equation}
\begin{aligned}
\frac{S_{mn}^{(N)}(\omega)}{S_{mn}(\omega)}
&=
\frac{
\det\!\left[
M(\omega)-\mathsf s^{(mn)}(\omega)
\right]
}{
\det M(\omega)
}.
\end{aligned}
\label{eq:app_det_ratio_s}
\end{equation}
This identity is exact wherever the quantities are nonsingular.  The denominator gives the collective resonances,
\begin{equation}
\det M(\omega)=0,
\label{eq:app_poles}
\end{equation}
while the numerator gives the transmission zeros associated with destructive interference between the direct photonic path and the emitter-mediated path.  A zero of $\det M$ appears as an observable pole in the measured channel only if the corresponding collective mode has nonzero overlap with both the input-drive vector and the output-radiation vector.

It is often useful to separate the collective matrix into a diagonal detuning matrix and an emitter--emitter Green-function matrix, using the notation introduced in Eq.~\eqref{eq:M_Delta_g},
\begin{equation}
M(\omega)=\Delta(\omega)+\mathsf g(\omega),
\label{eq:app_M_D_g}
\end{equation}
\begin{equation}
\Delta_{ij}(\omega)=(\omega-\omega_i)\delta_{ij},
\qquad
\mathsf g_{ij}(\omega)=-\Sigma_{ij}(\omega).
\label{eq:app_Delta_g_defs}
\end{equation}
The determinant ratio then becomes
\begin{equation}
\begin{aligned}
\frac{S_{mn}^{(N)}}{S_{mn}}
&=
\frac{
\det\!\left[
\Delta+\mathsf g-\mathsf s^{(mn)}
\right]
}{
\det\!\left[
\Delta+\mathsf g
\right]
}.
\end{aligned}
\label{eq:app_D_g_s_ratio}
\end{equation}
Equation~\eqref{eq:app_D_g_s_ratio} is the general pole--zero form.  No one-dimensional approximation has been made.  In a generic multimode or three-dimensional nanophotonic structure, the matrix $\mathsf g-\mathsf s^{(mn)}$ is full, and the numerator contains nontrivial information about both the collective eigenvectors and the measured input--output channel.

For identical emitters, $\Delta(\omega)=D(\omega)I$, with $D(\omega)$ the common single-emitter denominator.  A further simplification occurs when $\mathsf g-\mathsf s^{(mn)}$ is strictly triangular after ordering the emitters.  That is, after labeling the emitters such that $z_1<z_2<\cdots<z_N$, suppose $(\mathsf g-\mathsf s^{(mn)})_{ii}=0$, and either
\begin{equation}
(\mathsf g-\mathsf s^{(mn)})_{ij}=0 \quad \text{for }i>j,
\end{equation}
or
\begin{equation}
(\mathsf g-\mathsf s^{(mn)})_{ij}=0 \quad \text{for }i<j.
\end{equation}
Then $D I+\mathsf g-\mathsf s^{(mn)}$ is triangular with diagonal entries $D$, so
\begin{equation}
\det\!\left[D I+\mathsf g-\mathsf s^{(mn)}\right]
=
D^N.
\label{eq:app_triangular_det}
\end{equation}
If $\lambda_\xi$ are the eigenvalues of $\mathsf g$, then $\det(DI+\mathsf g)=\prod_{\xi=1}^{N}(D+\lambda_\xi)$, and Eq.~\eqref{eq:app_D_g_s_ratio} reduces to
\begin{equation}
\frac{S_{mn}^{(N)}}{S_{mn}}
=
\prod_{\xi=1}^{N} \frac{D}{D+\lambda_\xi}.
\label{eq:app_product_formula}
\end{equation}
This is the product-over-collective-modes formula.  It depends only on the eigenvalues of the emitter Green-function matrix $\mathsf g$, not on the eigenvectors.  The eigenvectors enter only through the condition that makes the numerator determinant trivial.

We now show when this triangular structure appears.  The essential requirement is a single ordered propagation channel.  Consider a uniform single-mode waveguide and let the emitters be located at $\mathbf r_i=(\boldsymbol\rho_i,z_i)$ with $z_1<z_2<\cdots<z_N$.  The atoms may have different transverse positions $\boldsymbol\rho_i$.  For a left-to-right transmission measurement, the right-propagating guided mode gives local dipole-projected coupling amplitudes
\begin{equation}
\eta_i \equiv \mathcal D_i^\dagger \mathcal E_R(\boldsymbol\rho_i),
\label{eq:app_eta_def}
\end{equation}
including the transverse mode profile and dipole orientation.  The guided emitter--emitter Green matrix has the ordered form
\begin{equation}
\mathsf g_{ij}^{\rm wg}
=
C(\omega)\, \eta_i\eta_j^* e^{ik|z_i-z_j|}.
\label{eq:app_uniform_wg_g}
\end{equation}
The input-to-emitter and emitter-to-output amplitudes factorize as
\begin{equation}
[\mathbf g_{\rm in}]_i \propto \eta_i e^{ik(z_i-z_L)}, \qquad
[\mathbf g_{\rm out}]_j \propto \eta_j^* e^{ik(z_R-z_j)},
\end{equation}
while the direct passive transmission is proportional to $S_{mn}\propto e^{ik(z_R-z_L)}$.  Therefore the rank-one input--output matrix has entries
\begin{equation}
\mathsf s_{ij}^{\rm wg}
=
C(\omega)\, \eta_i\eta_j^* e^{ik(z_i-z_j)}
\label{eq:app_uniform_wg_s}
\end{equation}
up to the sign convention already fixed in Eq.~\eqref{eq:app_s_def}.  Comparing Eqs.~\eqref{eq:app_uniform_wg_g} and~\eqref{eq:app_uniform_wg_s}, for $i>j$ we have $z_i-z_j=|z_i-z_j|$, so $\mathsf s_{ij}^{\rm wg}=\mathsf g_{ij}^{\rm wg}$.  With the usual coincident-point prescription, the diagonal also cancels.  Hence $\mathsf g^{\rm wg}-\mathsf s^{\rm wg}$ is strictly triangular.  Thus a uniform single-mode waveguide satisfies the condition for Eq.~\eqref{eq:app_product_formula}, even when the emitters sit at different transverse positions; the transverse dependence simply changes the local coupling factors $\eta_i$.

The same reasoning extends to more general effectively one-dimensional single-channel structures.  If the scalar Green function can be written in terms of left- and right-regular solutions as
\begin{equation}
\begin{aligned}
G(x,x')
&=
\frac{ \phi_L(x_<)\phi_R(x_>) }{W},
\\
x_<
&\equiv \min(x,x'),
\qquad
x_>\equiv \max(x,x'),
\end{aligned}
\label{eq:app_1D_G_factorized}
\end{equation}
then the product $G(x_i,x_L)G(x_R,x_j)/G(x_R,x_L)$ equals one ordered branch of $G(x_i,x_j)$.  Consequently $\mathsf s_{ij}$ cancels $\mathsf g_{ij}$ on one triangular half, and the product formula follows.

A different but related simplification occurs for a single dominant cavity mode.  If the Green function is separable,
\begin{equation}
\begin{aligned}
g(\mathbf r,\mathbf r',\omega)
&\simeq
C(\omega)\,
u(\mathbf r,\omega)
u^*(\mathbf r',\omega),
\end{aligned}
\label{eq:app_cavity_separable_g}
\end{equation}
then the emitter Green matrix is rank one,
\begin{equation}
\mathsf g_{ij}
=
\lambda(\omega)\, u_i u_j^*,
\label{eq:app_cavity_rank_one_g}
\end{equation}
where $u_i$ denotes the dipole-projected cavity mode at emitter $i$.  The input-to-emitter and emitter-to-output vectors are proportional to the same mode profile, $[\mathbf g_{\rm in}]_i\propto u_i$ and $[\mathbf g_{\rm out}]_j\propto u_j^*$.  Since the direct passive transmission carries the same cavity propagator, the matrix $\mathsf s$ is proportional to the same rank-one object as $\mathsf g$.  With the same normalization and sign convention, $\mathsf s=\mathsf g$, so $\mathsf g-\mathsf s=0$.  The numerator determinant is therefore again $D^N$.  Because $\mathsf g$ has only one nonzero eigenvalue $\lambda_B$, the denominator is $\det(DI+\mathsf g)=D^{N-1}(D+\lambda_B)$, and the transmission ratio becomes
\begin{equation}
\frac{S_{mn}^{(N)}}{S_{mn}}
=
\frac{D}{D+\lambda_B}.
\label{eq:app_superatom_result}
\end{equation}
This is the familiar bright-mode or ``superatom'' limit: one collective emitter mode couples to the cavity field, while the $N-1$ orthogonal dark modes do not appear in the transmission.

In a generic nanophotonic structure, these simplifications do not occur.  The emitter--emitter matrix may contain contributions from multiple guided modes, radiation modes, polarization-mixed channels, and near-field interactions,
\begin{equation}
\mathsf g
=
\mathsf g^{(1)} + \mathsf g^{(2)} + \mathsf g^{({\rm rad})} +\cdots .
\end{equation}
The matrix $\mathsf s^{(mn)}$, however, is only the rank-one matrix associated with the selected input--output channel.  It therefore cancels at most the ordered part of the particular propagation channel being measured.  The remaining contributions make $\mathsf g-\mathsf s^{(mn)}$ a full matrix, and the numerator determinant in Eq.~\eqref{eq:app_D_g_s_ratio} must be retained.  Thus the determinant ratio is general, while the eigenvalue-only product formula is a special consequence of single-channel factorization.

\section{Lamb Shift and Spontaneous emission rate}
\label{appsec: Lamb_Shift_and_Spontaneous_emission_rate}

% $$\begin{split}\hat d = q \hat r = q I\hat r I = q (\ket{e}\bra e + \ket g \bra g) \hat r (\ket{e}\bra e + \ket g \bra g) \\
% = q( \ket e r_{eg} \bra g + \ket g r_{ge} \bra e) = q r_{eg} \sigma^+ + qr_{ge}\sigma\\
% = d^* \sigma^+ + d\sigma
% \end{split}$$
% which in the Dual form is $$\hat{\mathbb D} = \mathcal{D}^\dagger \sigma^+(\omega) + \mathcal{D} \sigma(\omega)$$

% For the self field, 
% $$\hat{\mathcal E}_{\text{self}}(\mathbf r_A, \omega) = \omega g(\mathbf r_A, \mathbf r_A, \omega) \mathcal{D} \hat\sigma(\omega)$$
% in time domain, 
% $$\hat{\mathcal E}_{\text{self}}(\mathbf r_A, t) =  i g(\mathbf r_A, \mathbf r_A, t) * \mathcal{D} \frac{\partial}{\partial t} \hat{\sigma}(t)$$under the convention of forward Fourier transform with $e^{i\omega t}$, which is probably correct.
% Lets start with freq. domain of current and check, note that current should increase as the magnitude of dipole change increases so there shouldn't be a negative in j and dipole relation.
% $$
% \begin{split}
% \hat{\mathcal{E}}_{\text{self}}(\mathbf r, \omega) = i \int_V g(\mathbf r, \mathbf r', \omega)\hat{\mathcal{J}}(\mathbf r', \omega) d^3 r'\\
% \implies \hat{\mathcal{E}}_{\text{self}}(\mathbf r,t)= i \int_V g(\mathbf r, \mathbf r', t) *\hat{\mathcal{J}}(\mathbf r', t) d^3 r'\\
% = i\int_V g(\mathbf r, \mathbf r', t) *(\mathcal{D}\frac{\partial }{\partial t}\hat{\sigma}(t)) \delta(\mathbf r - \mathbf r') d^3 r'\\
% \implies \hat{\mathcal{E}}_{\text{self}}(\mathbf r,\omega)= -i g(\mathbf r, \mathbf r, \omega) (i\omega \mathcal{D}\hat{\sigma}(\omega))\\
% \implies \hat{\mathcal{E}}_{\text{self}}(\omega)= \omega g(\mathbf r, \mathbf r, \omega) \mathcal{D} \hat{\sigma}(\omega)
% \end{split}
% $$
% From the Heisenberg-Langevin equation, 
% $$
% \begin{split}
% \dot{\hat \sigma}(t) = i\omega_A \hat{\sigma}(t) + \frac{i}{\hbar}\mathcal{D}^\dagger \hat{\mathcal{E}}_{\text{self}}(\mathbf r_A, t) \hat{\sigma}_z(t)\\
% =i\omega_A \hat{\sigma}(t) + \frac{i^2}{\hbar}\mathcal{D}^\dagger g(\mathbf r_A, \mathbf r_A, t) * \mathcal{D} \frac{\partial}{\partial t} \hat{\sigma}(t) \hat{\sigma}_z(t)\\
% =i\omega_A \hat{\sigma}(t) - \frac{1}{\hbar}\mathcal{D}^\dagger g(\mathbf r_A, \mathbf r_A, t) \mathcal{D} *\dot{\hat{\sigma}}(t) \hat{\sigma}_z(t)
% \end{split}
% $$
% For the atom to behave linearly, we need to work within low-saturation regime, because GF method is valid only for linear systems. Therefore, $\sigma_z(t) \approx -1$, that means initial coherence value $\langle\hat{\sigma}(0)\rangle$ will be very small but not zero.
% $$
% \begin{split}
% \dot{\hat \sigma}(t) =i\omega_A \hat{\sigma}(t) + \frac{1}{\hbar}\mathcal{D}^\dagger g(\mathbf r_A, \mathbf r_A, t) \mathcal{D} *\dot{\hat{\sigma}}(t) \\
% \implies \dot{\hat \sigma}(t)  - \frac{1}{\hbar}\mathcal{D}^\dagger g(\mathbf r_A, \mathbf r_A, t) \mathcal{D} *\dot{\hat{\sigma}}(t)=i\omega_A \hat{\sigma}(t)
% \end{split}$$
% apply the Laplace transform with the forward convention of $e^{-st}$,
% $$
% \begin{split}
% \implies (1 - \frac{1}{\hbar}\mathcal{D}^\dagger g(\mathbf r_A, \mathbf r_A, s) \mathcal{D})(s\hat \Sigma(s)-\hat{\sigma}(0)) =i\omega_A \hat{\Sigma}(s)\\
% \implies \Big((1 - \frac{1}{\hbar}\mathcal{D}^\dagger g(\mathbf r_A, \mathbf r_A, s) \mathcal{D})s-i\omega_A \Big)\hat \Sigma(s) = (1 - \frac{1}{\hbar}\mathcal{D}^\dagger g(\mathbf r_A, \mathbf r_A, s) \mathcal{D})\hat{\sigma}(0)\\
% \implies \hat \Sigma(s) = \frac{(1 - \frac{1}{\hbar}\mathcal{D}^\dagger g(\mathbf r_A, \mathbf r_A, s) \mathcal{D})}{(1 - \frac{1}{\hbar}\mathcal{D}^\dagger g(\mathbf r_A, \mathbf r_A, s) \mathcal{D})s-i\omega_A }\hat{\sigma}(0)\\
% \implies \hat \Sigma(s) = \frac{\hat{\sigma}(0)}{s-\frac{i\omega_A}{(1 - \frac{1}{\hbar}\mathcal{D}^\dagger g(\mathbf r_A, \mathbf r_A, s) \mathcal{D})} }
% \end{split}$$
% For Markovian type reservoir, the Green's function response for the emitter's environment can be approximated to be only a function of the emitter's response, essentially rendering it to be freq. independent.
% $$
% \hat \Sigma(s) = \frac{\hat{\sigma}(0)}{s-\frac{i\omega_A}{(1 - \frac{1}{\hbar}\mathcal{D}^\dagger g(\mathbf r_A, \mathbf r_A, -i\omega_A) \mathcal{D})} }
% $$
% let $(1 - \frac{1}{\hbar}\mathcal{D}^\dagger g(\mathbf r_A, \mathbf r_A, -i\omega_A) \mathcal{D}) = 1-\Omega'/\hbar$ ,
% now, for low saturation regime $\Omega'/\hbar<1$ then one can use the T.S expansion of $1/(1-x) \approx 1 + x + x^2...$.
% Then, 
% $$\frac{i\omega_A}{1-\Omega'/\hbar} = i\omega_A(1+ \Omega'/\hbar)$$neglecting higher terms,
% $$
% \hat \Sigma(s) = \frac{\hat{\sigma}(0)}{s- i\omega_A(1+ \Omega'/\hbar)} = \frac{\hat{\sigma}(0)}{s- i\omega_A -i\omega_A \Omega'/\hbar}
% $$
% Now, since the GF can be decomposed into its real and imaginary parts, 
% $\Omega' = \Omega_R + i\Omega_I$,
% $$
% \hat \Sigma(s)  = \frac{\hat{\sigma}(0)}{s- i\omega_A -i\omega_A \frac{\mathcal{D} g_R(\omega_A) \mathcal{D}}{\hbar} + \omega_A\frac{\mathcal{D} g_I(\omega_A) \mathcal{D}}{\hbar}}
% $$
% performing the inverse Laplace transform, 
% $$
% \hat \sigma(t)  = \hat{\sigma}(0)e^{i(\omega_A + \omega_A \mathcal{D}g_R \mathcal{D}/\hbar)t}e^{-\omega_A \mathcal{D} g_I \mathcal{D} t/\hbar}
% $$

We begin with the equation~\eqref{eq: lowering_operatr_time_DiffEq}, where the interaction is expressed as a time convolution ($*$) involving the Green's tensor,
\begin{equation}
\begin{split}
\dot{\hat{\sigma}}(t) = -i\omega_a \hat{\sigma}(t) 
+ \frac{-1}{\hbar} \mathcal{D}^\dagger g(\mathbf{r}_A, \mathbf{r}_A, t) \mathcal{D} * [\dot{\hat{\sigma}}(t)\sigma_z(t)].
\end{split}
\end{equation}

For notational simplicity, we drop the arguments of $g$ from here on. Under the low-saturation regime of the two-level system $\sigma_z(t) = -1$ resulting in,
\begin{align}\dot{\hat{\sigma}}(t) = -i\omega_a \hat{\sigma}(t) + \frac{1}{\hbar} \mathcal{D}^\dagger g(\mathbf r_A, \mathbf r_A, t) \mathcal{D} * \dot{\hat{\sigma}}(t).\end{align}

\noindent Performing the Laplace transform (under the definition $\hat\Sigma(s) = \int_{-\infty}^\infty \hat\sigma(t)e^{-st} dt$),

\begin{equation}
\begin{split}
   \Big((1 + \frac{1}{\hbar}\mathcal{D}^\dagger g(\mathbf r_A, \mathbf r_A, s) \mathcal{D})s + i\omega_A \Big)\hat \Sigma(s)\\
   = (1 + \frac{1}{\hbar}\mathcal{D}^\dagger g(\mathbf r_A, \mathbf r_A, s) \mathcal{D})\hat{\sigma}(0)
\end{split}
\end{equation}
rearranging, 
\begin{equation}
    \begin{split}
        \hat \Sigma(s) = \frac{\hat{\sigma}(0)}{ s + \frac{i\omega_A}{(1 + \frac{1}{\hbar}\mathcal{D}^\dagger g(\mathbf r_A, \mathbf r_A, s) \mathcal{D})} }
    \end{split}
\end{equation}
For Markovian-type reservoir, the Green's function response for the emitter's environment can be approximated to be only a function of the emitter's frequency, essentially rendering it frequency independent.
\begin{equation}
\hat \Sigma(s) = \frac{\hat{\sigma}(0)}{s + \frac{i\omega_A}{(1  + \frac{1}{\hbar}\mathcal{D}^\dagger g(\mathbf r_A, \mathbf r_A, -i\omega_A) \mathcal{D})} }
\end{equation}
Let $(1  +  \frac{1}{\hbar}\mathcal{D}^\dagger g(\mathbf r_A, \mathbf r_A, -i\omega_A) \mathcal{D}) = 1 + \Omega'/\hbar$ ,
then for the low-saturation regime $\Omega'/\hbar<1$, one can use the Taylor series expansion of $1/(1+x) \approx 1 - x + x^2...$.
Then, 
\begin{equation}\frac{i\omega_A}{1 + \Omega'/\hbar} = i\omega_A(1 -  \Omega'/\hbar)\end{equation}neglecting higher terms,
\begin{equation}
\hat \Sigma(s) = \frac{\hat{\sigma}(0)}{s + i\omega_A(1 - \Omega'/\hbar)} = \frac{\hat{\sigma}(0)}{s + i\omega_A  -i\omega_A \Omega'/\hbar}
\end{equation}
Now, since the Greens' function can be decomposed into its real and imaginary parts, 
$g' = g_R + ig_I$,
\begin{equation}
\hat \Sigma(s)  = \frac{\hat{\sigma}(0)}{s + i\omega_A -i\omega_A \frac{\mathcal{D}^\dagger g_R \mathcal{D}}{\hbar} + \omega_A\frac{\mathcal{D}^\dagger g_I \mathcal{D}}{\hbar}}
\end{equation}
performing the inverse Laplace transform, 
\begin{equation}
\hat \sigma(t)  = \hat{\sigma}(0)e^{i(\omega_A  - \omega_A \mathcal{D}^\dagger g_R \mathcal{D}/\hbar)t}e^{-\omega_A \mathcal{D}^\dagger g_I \mathcal{D} t/\hbar}
\label{appeq: Lamb_decay}
\end{equation}
