# Supplementary material for: Modal input-output theory for quantum nanophotonics from the first-order Maxwell operator
Source: arXiv:2610.04043 source file (2026-10-02)
Supplement: Supplementary file 2 [file appendix_cavity_green.tex]

\section{Cavity eigenmode expansion and single-resonance limit}
\label{app:cavity_green_derivation}

This appendix derives the closed-system eigenmode expansion used in Sec.~III and fixes the normalization of its single-resonance approximation. The starting point is the first-order Maxwell operator in Eq.~\eqref{eq:first_order_green_definition}, with $\mathcal M=\mathcal H-k_0\bar\varepsilon$, $\mathcal H=i\bar\nabla\times$, and $\mathcal M G=I$. Here $G$ is the operator with kernel $g$ and $k_0=\omega/c$.

\subsection{Closed, lossless system}

Consider a closed volume $V$ with boundary conditions making the bilinear boundary flux vanish, such as perfectly electric or magnetic conducting walls. The material tensor is nondispersive, Hermitian, and positive definite, $\bar\varepsilon^\dagger=\bar\varepsilon>0$, but may vary arbitrarily in space. These assumptions make $\mathcal H$ self-adjoint on the chosen domain and give a positive material-weighted inner product. The source-free modes obey the generalized eigenproblem~\cite{sakoda2004optical,silveirinha2021modal}
\begin{equation}
\mathcal H\mathcal E_n=k_{0,n}\bar\varepsilon\mathcal E_n,
\qquad k_{0,n}=\omega_n/c.
\label{eq:cgd_eigenproblem}
\end{equation}
Define
\begin{equation}
\langle\mathcal E_m|\mathcal E_n\rangle_{\bar\varepsilon}
=\int_V\mathcal E_m^\dagger(\mathbf r)\bar\varepsilon(\mathbf r)
\mathcal E_n(\mathbf r)\,dV.
\label{eq:cgd_inner_product}
\end{equation}
Applying self-adjointness to two eigenmodes gives
\begin{equation}
(k_{0,n}-k_{0,m}^*)
\langle\mathcal E_m|\mathcal E_n\rangle_{\bar\varepsilon}=0.
\label{eq:cgd_orthogonality}
\end{equation}
Taking $m=n$ establishes real eigenvalues; distinct eigenvalues then give orthogonal modes. Within degenerate subspaces we choose an orthonormal basis, so that
\begin{equation}
\int_V\mathcal E_m^\dagger\bar\varepsilon\mathcal E_n\,dV
=\delta_{mn}.
\label{eq:cgd_normalization}
\end{equation}
This normalization uses the full dual field $\mathcal E_n=[\mathbf E_n,Z_0\mathbf H_n]^T$, not only its electric component.

The transformation $\mathcal F_n=\bar\varepsilon^{1/2}\mathcal E_n$ reduces Eq.~\eqref{eq:cgd_eigenproblem} to an ordinary Hermitian eigenproblem,
\begin{equation}
\begin{gathered}
\mathcal K\mathcal F_n=k_{0,n}\mathcal F_n,\qquad
\mathcal K=\bar\varepsilon^{-1/2}\mathcal H\bar\varepsilon^{-1/2},\\
\langle\mathcal F_m|\mathcal F_n\rangle=\delta_{mn}.
\end{gathered}
\label{eq:cgd_Hermitian_transform}
\end{equation}
Completeness therefore gives
\begin{equation}
\sum_n|\mathcal E_n\rangle\langle\mathcal E_n|\bar\varepsilon=I.
\label{eq:cgd_closure}
\end{equation}
The sum and identity refer to the same field space. A full first-order inverse includes the complete spectrum, including negative-frequency and any required static sectors; if a constrained subspace is used, the identity and inverse are restricted consistently to that subspace.

\subsection{Retarded Green function}

Since $\mathcal M=\bar\varepsilon^{1/2}(\mathcal K-k_0)\bar\varepsilon^{1/2}$, its retarded inverse is
\begin{equation}
\begin{aligned}
G
&=\bar\varepsilon^{-1/2}
(\mathcal K-k_0-i0^+)^{-1}\bar\varepsilon^{-1/2}\\
&=\sum_n\frac{|\mathcal E_n\rangle\langle\mathcal E_n|}
{k_{0,n}-k_0-i0^+}.
\end{aligned}
\label{eq:cgd_resolvent}
\end{equation}
In position space this is
\begin{equation}
g(\mathbf r,\mathbf r',\omega)
=\sum_n\frac{\mathcal E_n(\mathbf r)\mathcal E_n^\dagger(\mathbf r')}
{k_{0,n}-k_0-i0^+},
\label{eq:cgd_kernel}
\end{equation}
which reproduces Eq.~\eqref{eq:cav_green_spectral}. The minus infinitesimal follows from approaching real frequency as $\omega+i0^+$ with the $e^{-i\omega t}$ convention. The transformed resolvent also shows why no additional material tensor appears in the numerator: the energy weight has already been included in the mode normalization. Material dispersion would require a generalized energy normalization or an enlarged field--material eigenproblem; Eqs.~\eqref{eq:cgd_normalization}--\eqref{eq:cgd_resolvent} use the nondispersive assumption explicitly.

\subsection{Weak loss and a single cavity resonance}

For a weakly perturbed, high-$Q$ cavity with a well-isolated resonance, retain the corresponding closed-system mode profile to leading order and replace its real resonance by the complex frequency~\cite{kristensen2014quasinormal}
\begin{equation}
\tilde\omega_c=\omega_c-i\kappa/2,
\qquad
\tilde k_{0,c}=\frac{\omega_c}{c}-\frac{i\kappa}{2c}.
\label{eq:cgd_complex_pole}
\end{equation}
Here $\omega_c$ may include the small real resonance shift, and $\kappa$ is the total energy-decay rate from radiative leakage and material absorption; the field amplitude decays at rate $\kappa/2$. The mode-profile approximation requires perturbatively small changes to the residue and negligible mixing with neighboring modes, not merely a small linewidth compared with the optical frequency. It is not intended for overlapping resonances or exceptional points.

The resonant contribution inherited from Eq.~\eqref{eq:cgd_kernel} is
\begin{equation}
g_{\rm res}(\mathbf r,\mathbf r',\omega)
\simeq\frac{\mathcal E_c(\mathbf r)\mathcal E_c^\dagger(\mathbf r')}
{k_{0,c}-k_0-i\kappa/(2c)}.
\label{eq:cgd_single_k}
\end{equation}
To express the denominator in frequency units, use
\begin{equation}
\begin{aligned}
k_{0,c}-k_0-\frac{i\kappa}{2c}
&=\frac{\omega_c-\omega-i\kappa/2}{c}\\
&=-\frac{\Delta(\omega)+i\kappa/2}{c},
\end{aligned}
\label{eq:cgd_conversion}
\end{equation}
where $\Delta(\omega)=\omega-\omega_c$. Consequently,
\begin{equation}
g_{\rm res}(\mathbf r,\mathbf r',\omega)
\simeq-\frac{c\,\mathcal E_c(\mathbf r)\mathcal E_c^\dagger(\mathbf r')}
{\Delta(\omega)+i\kappa/2}.
\label{eq:cgd_single_omega}
\end{equation}
Thus the factor $-c$ is fixed by the conversion from wavenumber to frequency while retaining the normalization in Eq.~\eqref{eq:cgd_normalization}. It is not an additional coupling coefficient. In particular, changing the phase of $\mathcal E_c$ cannot absorb the minus sign because the outer product $\mathcal E_c\mathcal E_c^\dagger$ is phase invariant. As a sign check, at resonance Eq.~\eqref{eq:cgd_single_omega} gives $g_{\rm res}=2ic\,\mathcal E_c\mathcal E_c^\dagger/\kappa$, with a positive semidefinite imaginary part.

The full Green function may also contain a smooth nonresonant background, $g=g_{\rm bg}+g_{\rm res}$. The single-mode approximation $g\simeq g_{\rm res}$ applies when that background is negligible for the observable under consideration; a direct transmission or reflection path must otherwise be retained. A general open or strongly dispersive cavity requires its properly normalized left and right mode residues rather than the unmodified closed-system outer product used here.
