# Supplementary material for: Modal input-output theory for quantum nanophotonics from the first-order Maxwell operator
Source: arXiv:2610.04043 source file (2026-10-02)
Supplement: Supplementary file 3 [file appendix_collective_transmission.tex]

\section{Collective modes and transmission zeros}
\label{app:collective_transmission}

This appendix gives two interpretations of the stationary, low-saturation scattering result in Eq.~\eqref{eq:dressed_S_N_new}. All Green functions and couplings retain their frequency dependence, and the emitter self-energy uses the convention of Appendix~\ref{app:emitter_details}.

\subsection{Which collective modes appear in transmission?}

At frequencies where the inverse collective susceptibility $\mathbf M(\omega)$ is diagonalizable, choose right and left eigenvectors satisfying
\begin{equation}
\begin{aligned}
\mathbf M\mathbf u_\alpha&=\Lambda_\alpha\mathbf u_\alpha,\qquad
\mathbf v_\alpha^\dagger\mathbf M=\Lambda_\alpha\mathbf v_\alpha^\dagger,\\
\mathbf v_\alpha^\dagger\mathbf u_\beta&=\delta_{\alpha\beta},
\qquad
\mathbf M^{-1}=\sum_\alpha
\frac{\mathbf u_\alpha\mathbf v_\alpha^\dagger}{\Lambda_\alpha}.
\end{aligned}
\label{eq:ct_modes}
\end{equation}
Substitution into the scattering expression gives
\begin{equation}
S_{mn}^{(N)}
=S_{mn}
+\sum_\alpha
\frac{(\mathbf g_{{\rm out},m}^{T}\mathbf u_\alpha)
(\mathbf v_\alpha^\dagger\mathbf g_{{\rm in},n})}
{\Lambda_\alpha}.
\label{eq:ct_modal_scattering}
\end{equation}
The two numerator factors describe excitation of a collective mode by the input and its radiation into the selected output. A mode contributes only when both overlaps are nonzero. A long-lived mode can therefore be nearly invisible in transmission, while a strongly coupled mode can dominate the measured spectrum~\cite{asenjo-garcia2017atom,asenjo-garcia2017exponential}. The contributions add as amplitudes and can interfere.

Equation~\eqref{eq:ct_modal_scattering} is a frequency-dependent spectral decomposition, not an assumption of one Lorentzian per collective mode. For an isolated simple zero $\Lambda_\alpha(\omega_p)=0$, the pole residue also contains the factor $1/\partial_\omega\Lambda_\alpha(\omega_p)$. At a defective eigenvalue, the diagonal expansion must be replaced by the appropriate generalized-eigenvector form; the original matrix inverse remains the starting point wherever it exists.

\subsection{General determinant identity}

For one selected input--output pair, write $t=S_{mn}$ and $t_N=S_{mn}^{(N)}$, so that
\begin{equation}
t_N=t+\mathbf g_{\rm out}^{T}\mathbf M^{-1}\mathbf g_{\rm in}.
\label{eq:ct_transmission}
\end{equation}
For invertible $\mathbf M$ and nonzero $t$, the matrix determinant lemma gives
\begin{equation}
\frac{t_N}{t}
=\frac{\det\!\left[
\mathbf M+\mathbf g_{\rm in}\mathbf g_{\rm out}^{T}/t
\right]}{\det\mathbf M}.
\label{eq:ct_determinant_ratio}
\end{equation}
No one-dimensional or single-mode assumption is needed: selecting a scalar scattering element makes the update rank one. The identity also holds without dividing by the background transmission, in the form
\begin{equation}
t_N
=\frac{
\det\begin{pmatrix}
\mathbf M&\mathbf g_{\rm in}\\
-\mathbf g_{\rm out}^{T}&t
\end{pmatrix}}
{\det\mathbf M}.
\label{eq:ct_block_determinant}
\end{equation}
This form remains useful when $t=0$, provided $\mathbf M$ is invertible.

Where the background and couplings are regular, zeros of $\det\mathbf M$ locate candidate collective poles, while zeros of the numerator in Eq.~\eqref{eq:ct_block_determinant} give transmission zeros. Common factors can cancel: a collective pole need not appear in a particular measured channel, and transmission can vanish through interference between the background and emitter-mediated amplitudes. The determinant representation does not remove any frequency dependence or branch cuts inherited from the photonic environment. A further reduction to a product involving only collective eigenvalues requires additional factorization of the channel couplings and is not assumed here.
