# Supplementary material for: Modal input-output theory for quantum nanophotonics from the first-order Maxwell operator
Source: arXiv:2610.04043 source file (2026-10-02)
Supplement: Supplementary file 4 [file appendix_composite.tex]

\section{Composite nanophotonic systems}
\label{app:composite_moved}

This appendix extends the cavity and waveguide examples of Sec.~\ref{sec:applications} to coupled structures. The procedure is the same: construct an approximate Green function for the composite system and insert it into the boundary scattering expression, Eq.~\eqref{eq:S_matrix_braket}. We consider coupled cavity modes first, then a cavity coupled to a waveguide continuum.

We use a reduced basis with the common energy normalization of Eq.~\eqref{eq:cgd_normalization}. Modes calculated for separate dielectric structures are not automatically orthogonal under this common inner product; they must be orthogonalized, or their overlap matrix must be retained in the projected equations. The following expressions describe the retained modal subspace over the frequency range where this reduction is accurate, rather than a complete expansion for an arbitrary open structure.

\subsection{Coupled cavities}
\label{sec:coupled_cavities}

For $N$ coupled cavity modes, collect their spatial profiles into $\mathsf E(\mathbf r)=(\mathcal E_1(\mathbf r),\ldots,\mathcal E_N(\mathbf r))$. Their frequency-domain response and the corresponding resonant Green function are
\begin{equation}
\begin{aligned}
R(\omega)&=[\omega I-H_{\rm eff}]^{-1},\\
g_{\rm cav}(\mathbf r,\mathbf r',\omega)
&\simeq-c\,\mathsf E(\mathbf r)R(\omega)\mathsf E^\dagger(\mathbf r').
\end{aligned}
\label{eq:N_mode_green}
\end{equation}
Here $c$ is the speed of light, and the factor $-c$ follows from the conversion to frequency units in Eq.~\eqref{eq:cgd_single_omega}. The matrix element $R_{\mu\nu}$ describes excitation of cavity mode $\mu$ by a drive on mode $\nu$. The effective matrix includes the resonance frequencies, coupling between cavities, and decay into channels not retained explicitly~\cite{Hartmann2008QuantumManyBody,suh2004temporal}.

For two cavities, write $\tilde\omega_j=\omega_j-i\kappa_j/2$ and $\Delta_j=\omega-\tilde\omega_j$. The response is the inverse of
\begin{equation}
D=\omega I-H_{\rm eff}
=\begin{pmatrix}
\Delta_1&-J_{12}\\
-J_{21}&\Delta_2
\end{pmatrix},
\label{eq:dynamical_matrix}
\end{equation}
giving
\begin{equation}
R=D^{-1}
=\frac{1}{\mathcal D}
\begin{pmatrix}
\Delta_2&J_{12}\\
J_{21}&\Delta_1
\end{pmatrix},
\qquad
\mathcal D=\Delta_1\Delta_2-J_{12}J_{21}.
\label{eq:D_inverse}
\end{equation}
The diagonal terms describe the response within each cavity, while the off-diagonal terms describe transfer between them. For a frequency-independent $H_{\rm eff}$, the coupled resonances are the zeros of $\mathcal D$,
\begin{equation}
\omega_\pm=\frac{\tilde\omega_1+\tilde\omega_2}{2}
\pm\sqrt{J_{12}J_{21}
+\left(\frac{\tilde\omega_1-\tilde\omega_2}{2}\right)^2}.
\label{eq:hybridized_poles}
\end{equation}
Coupling can therefore change both the resonance frequencies and the linewidths. A symmetric coupling $J_{12}=J_{21}=J$ is a useful special case, but is not required in Eq.~\eqref{eq:D_inverse}.

For a passive reduced model, coherent and dissipative coupling can be separated as $H_{\rm eff}=\Omega-i\Gamma/2$, with $\Omega=\Omega^\dagger$ and $\Gamma=\Gamma^\dagger\geq0$. Off-diagonal entries of $\Gamma$ describe decay through shared channels; they are constrained by passivity, rather than independent complex parameters. In particular, $|\Gamma_{12}|^2\leq\kappa_1\kappa_2$. This allows one coupled resonance to broaden while the other narrows.

To connect the cavity response to the external channels, define $B_{\rm in,out}=(\bar n_{\rm in,out}\times)$ and the boundary overlaps
\begin{equation}
\begin{aligned}
(\mathbf c_n)_\nu
&=\sqrt c\,\langle\mathcal E_\nu|B_{\rm in}
|\mathcal E_n^{\rm in}\rangle_{S_{\rm in}},\\
(\mathbf d_m)_\mu
&=i\sqrt c\,\langle\mathcal E_m^{\rm out}|B_{\rm out}
|\mathcal E_\mu\rangle_{S_{\rm out}}.
\end{aligned}
\label{eq:composite_channel_overlaps}
\end{equation}
Here $\mathbf c_n$ is a column vector that drives the cavity modes, and $\mathbf d_m$ is a row vector that projects their response onto output mode $m$. The factors of $\sqrt c$ and $i$ include the Green-function normalization and the phase convention of Eq.~\eqref{eq:S_matrix_braket}. At external reference planes, the cavity profiles must represent the consistently continued port fields of the reduced model, not unmodified closed-cavity modes evaluated outside their domain.

Substituting Eq.~\eqref{eq:N_mode_green} into the boundary scattering expression gives
\begin{equation}
S_{mn}=S_{mn}^{(0)}+\mathbf d_m R\,\mathbf c_n.
\label{eq: general_coupled_cavity_scattering_matrix}
\end{equation}
The background $S_{mn}^{(0)}$ accounts for paths not mediated by the retained cavity modes~\cite{fan2003temporal,suh2004temporal}. Reading the second term from right to left, the input drives the cavities, the matrix $R$ propagates the excitation between them, and the output overlap selects the detected channel. For a single cavity with no direct transmission path, expressing the channel couplings in terms of the port decay rates gives Eq.~\eqref{eq:cavity_io}. In a quantum description, the decay, channel couplings, and material-noise couplings must be obtained consistently so that the scattering and noise terms together preserve the output commutators.

\subsection{Cavity coupled to a waveguide}
\label{sec:composite_main}

A waveguide continuum can be included in the same projected description. We take one cavity mode coupled to lossless waveguide modes, with $H_{\rm w}|k\rangle=\omega_k|k\rangle$ and coupling amplitudes $h_k$ in frequency units. Let $z=\omega+i0^+$ and $R_{\rm w}=(zI-H_{\rm w})^{-1}$. The cavity frequency $\tilde\omega_c=\omega_c-i\kappa_{\rm int}/2$ includes only decay channels other than the explicitly retained waveguide, avoiding double counting of its leakage.

For cavity and waveguide amplitudes $x_c$ and $\mathbf x_{\rm w}$ driven by $f_c$ and $\mathbf f_{\rm w}$, the projected equations are
\begin{equation}
\begin{aligned}
(z-\tilde\omega_c)x_c-\mathbf h^\dagger\mathbf x_{\rm w}&=f_c,\\
(zI-H_{\rm w})\mathbf x_{\rm w}-\mathbf h x_c&=\mathbf f_{\rm w}.
\end{aligned}
\label{eq:composite_block_equations}
\end{equation}
The second equation gives $\mathbf x_{\rm w}=R_{\rm w}(\mathbf f_{\rm w}+\mathbf h x_c)$. Substituting it into the first eliminates the waveguide amplitudes and gives the dressed cavity response,
\begin{equation}
\begin{aligned}
x_c&=R_c\bigl(f_c+\mathbf h^\dagger R_{\rm w}\mathbf f_{\rm w}\bigr),\\
R_c(\omega)&=\frac{1}{z-\tilde\omega_c-\Sigma(\omega)},\\
\Sigma(\omega)&=\mathbf h^\dagger R_{\rm w}\mathbf h
=\sum_k\frac{|h_k|^2}{\omega-\omega_k+i0^+}.
\end{aligned}
\label{eq:composite_self_energy}
\end{equation}
The self-energy is the amplitude for an excitation to leave the cavity, propagate through the waveguide, and return. This elimination does not require weak coupling or a Markov approximation within the chosen projected model.

The same substitution gives all four blocks of the composite response,
\begin{equation}
R_{\rm full}=
\begin{pmatrix}
R_c&R_c\mathbf h^\dagger R_{\rm w}\\
R_{\rm w}\mathbf h R_c&
R_{\rm w}+R_{\rm w}\mathbf h R_c\mathbf h^\dagger R_{\rm w}
\end{pmatrix}.
\label{eq:composite_full_response}
\end{equation}
The off-diagonal blocks describe cavity-to-waveguide and waveguide-to-cavity propagation. The lower-right block includes both direct waveguide propagation and the path through the cavity. With $\mathsf E=(\mathcal E_c,\mathsf E_{\rm w})$, the corresponding projected Green function is $g_{\rm comp}\simeq-c\,\mathsf E R_{\rm full}\mathsf E^\dagger$, as in Eq.~\eqref{eq:N_mode_green}.

In the continuum limit, define the coupling-weighted spectral density $\mathcal J(\nu)=\sum_k|h_k|^2\delta(\nu-\omega_k)$. The retarded prescription in Eq.~\eqref{eq:composite_self_energy} gives
\begin{equation}
\begin{aligned}
\Sigma(\omega)&=\Delta_{\rm w}(\omega)-i\kappa_{\rm w}(\omega)/2,\\
\Delta_{\rm w}(\omega)&=\mathcal P\int
\frac{\mathcal J(\nu)}{\omega-\nu}\,d\nu,\\
\kappa_{\rm w}(\omega)&=2\pi\mathcal J(\omega).
\end{aligned}
\label{eq:composite_shift_decay}
\end{equation}
The integral covers the retained waveguide spectrum. The real part shifts the cavity resonance, and the imaginary part gives its decay into the waveguide~\cite{scully1997quantum}. For modes box-normalized over length $L$, the spectral density is
\begin{equation}
\mathcal J(\omega)=\frac{L}{2\pi}
\sum_{\alpha:\,\omega_{k_\alpha}=\omega}
\frac{|h_{k_\alpha}|^2}{|v_g(k_\alpha)|},
\label{eq:composite_spectral_density}
\end{equation}
where the sum includes all propagation directions and bands at that frequency.

Finally, partition the input and output overlaps of Eq.~\eqref{eq:composite_channel_overlaps} into cavity and waveguide components, $\mathbf c_n=(c_{cn},\mathbf c_{{\rm w}n})^T$ and $\mathbf d_m=(d_{mc},\mathbf d_{m{\rm w}})$. Contracting Eq.~\eqref{eq:composite_full_response} gives the effective couplings
\begin{equation}
\begin{aligned}
c_n^{\rm eff}&=c_{cn}+\mathbf h^\dagger R_{\rm w}\mathbf c_{{\rm w}n},\\
d_m^{\rm eff}&=d_{mc}+\mathbf d_{m{\rm w}}R_{\rm w}\mathbf h,
\end{aligned}
\label{eq:composite_effective_couplings}
\end{equation}
and hence
\begin{equation}
S_{mn}(\omega)=S_{mn}^{(0)}(\omega)
+\frac{d_m^{\rm eff}(\omega)c_n^{\rm eff}(\omega)}
{\omega-\omega_c-\Delta_{\rm w}(\omega)
+i[\kappa_{\rm int}+\kappa_{\rm w}(\omega)]/2}.
\label{eq:composite_scattering}
\end{equation}
Here $S_{mn}^{(0)}$ contains $\mathbf d_{m{\rm w}}R_{\rm w}\mathbf c_{{\rm w}n}$ and any background outside the retained subspace. The continuum boundary projections are taken with the retarded prescription before its limiting value; individual on-shell mode denominators are not scattering amplitudes. For a uniform guide without the cavity, the background reduces to the propagation result in Eq.~\eqref{eq:S_waveguide}. The resonant term need not be diagonal in the channel indices: the cavity can transfer light between different waveguide channels.

If the self-energy varies little over the frequency window of interest, typically the dressed cavity linewidth, it may be evaluated at a representative resonance frequency. This is the Markov approximation and recovers a cavity response with a constant frequency shift and linewidth. Otherwise Eq.~\eqref{eq:composite_scattering} retains the frequency dependence of the waveguide environment.
