# Supplementary material for: Modal input-output theory for quantum nanophotonics from the first-order Maxwell operator
Source: arXiv:2610.04043 source file (2026-10-02)
Supplement: Supplementary file 5 [file appendix_emitter_details.tex]

\section{Emitter self-energy convention and noise drive}
\label{app:emitter_details}

\subsection{Coincident-point self-interaction}

The diagonal Green function in Eq.~\eqref{eq:emitter_self_energy} is a regularized local-field quantity, not the unmodified point-source kernel. A source-region prescription removes the singular self-field while retaining the finite radiative contribution~\cite{Yaghjian1980}. Let $g_{\rm reg}$ denote the Green function evaluated with the chosen local-field or finite-size prescription, and define
\begin{equation}
\Sigma_i^{\rm reg}(\omega)
=-\frac{\omega Z_0}{\hbar}\mathcal D_i^\dagger g_{\rm reg}(\mathbf r_i,\mathbf r_i,\omega)\mathcal D_i.
\label{eq:emitter_details_raw_self_energy}
\end{equation}
We take $\omega_i$ to be the transition frequency in a specified reference environment, including its reference Lamb shift. To avoid counting that shift twice, the diagonal element used in $\mathbf M$ is
\begin{equation}
\begin{aligned}
\Sigma_{ii}(\omega)&=\Sigma_i^{\rm reg}(\omega)-\delta\omega_i^{\rm ref},\\
\delta\omega_i^{\rm ref}&=\operatorname{Re}\Sigma_i^{{\rm reg},{\rm ref}}(\omega_i).
\end{aligned}
\label{eq:emitter_details_reference_subtraction}
\end{equation}
Both self-energies use the same regularization prescription. The subtraction is a real, frequency-independent reference counterterm within the effective transition model; it does not remove the reference radiative decay or discard the remaining frequency dependence. For an isolated atom, the reference is vacuum. A measured host-medium transition can instead be used with the corresponding host reference. For $i\ne j$, Eq.~\eqref{eq:emitter_self_energy} needs no reference-frequency subtraction.

For a passive environment, the electromagnetic decay rate at a real evaluation frequency is
\begin{equation}
\Gamma_i(\omega)=-2\operatorname{Im}\Sigma_{ii}(\omega)
=\frac{2\omega Z_0}{\hbar}\mathcal D_i^\dagger\operatorname{Im}g_{\rm reg}(\mathbf r_i,\mathbf r_i,\omega)\mathcal D_i.
\label{eq:emitter_details_decay}
\end{equation}
Here $\operatorname{Im}g=(g-g^\dagger)/(2i)$. The total electromagnetic Green function is retained in this expression: using only its scattering part would omit the reference decay. Additional non-electromagnetic relaxation or dephasing is not included in this model.

The regularization is physical input to the point-emitter approximation. In particular, an emitter embedded in a material requires a consistent microscopic local-field or finite-size model~\cite{BuhmannDispForcesI}; subtracting a real vacuum singularity alone does not resolve all coincident-point problems in an absorbing host. The same local-field prescription must be used for the driving field, emitter radiation, and noise projections. The stationary solution assumes that initial emitter transients decay; a populated nondecaying bound mode would require a separate initial-state contribution.

\subsection{Material-noise drive}

The noise part of the background field is $\hat{\mathcal E}_{0,N}(\mathbf r,\omega)=k_0\int_V g(\mathbf r,\mathbf r',\omega)\hat{\mathcal P}_N(\mathbf r',\omega)\,dV'$. Projecting this field onto the emitter dipole gives the noise drive used in Eqs.~\eqref{eq:background_emitter_drive} and~\eqref{eq:N_sigma_solution},
\begin{multline}
[\hat{\mathbf F}_N(\omega)]_i
=-\frac{k_0}{\hbar}\mathcal D_i^\dagger
\int_V g(\mathbf r_i,\mathbf r',\omega)\hat{\mathcal P}_N(\mathbf r',\omega)\,dV'.
\label{eq:emitter_details_noise_drive}
\end{multline}
Since $\hat{\mathbf F}_N$ and $\hat\xi_m$ depend on the same material polarization noise, their cross correlations must be retained when evaluating the dressed noise in Eq.~\eqref{eq:N_dressed_noise}. This definition introduces no independent emitter bath; vacuum fluctuations also enter through the incoming channel operators.
