# Supplementary material for: Modal input-output theory for quantum nanophotonics from the first-order Maxwell operator
Source: arXiv:2610.04043 source file (2026-10-02)
Supplement: Supplementary file 6 [file appendix_old.tex]

\section{Coupled cavity Green's function}
\label{app: coupled_cavities}

We assume the total system consists of two single-mode cavities ($1$ and $2$). When they are far apart (uncoupled), the total Green's function is simply the sum of the individual responses:
\begin{equation}
G_0(\mathbf{r}, \mathbf{r}', \omega) = g_1 + g_2 \approx \sum_{\mu =1}^2\frac{\ket{\mathcal{E}_\mu}\bra{\mathcal{E}_\mu}}{\omega - \omega_\mu}
\end{equation}
where $\ket{\mathcal{E}_\mu}$ is the spatial mode profile of cavity $\mu$, and $\omega_\mu$ is the complex eigenfrequency (including material loss and radiation).

In first order six-vector form, the total wave operator for the coupled system is $\mathcal{M} = \mathcal{M}_0 - \mathcal{V}$, where $\mathcal{M} = \mathcal{H} - k_o\bar{\varepsilon}$ and $\mathcal{V}$ is the interaction parameter for the two cavities. Then with QNM form for permittivity~\cite{Wu2025Dissipative}, $\bar{\varepsilon}_{t}(\mathbf{r}) = \bar{\varepsilon}_{b}(\mathbf{r}) + \Delta\bar{\varepsilon}(\mathbf{r})$, where $\Delta\bar{\varepsilon}$ is the perturbation from the second cavity onto the first cavity. This decomposition defines the interaction term $\mathcal{V}$ as,
$\mathcal{M} = \mathcal{H} - k_o \epsilon_{ref}(\mathbf{r}) -k_o \Delta\epsilon(\mathbf{r})$ that is $\mathcal{V} = k_o\Delta\epsilon(\mathbf{r})$.
The collective Green's function $g$ must satisfy the Dyson Equation (provided $\mathcal{M}g=g\mathcal{M}=\mathbb{I}$), originating from,
\begin{equation}
\begin{split}(\mathcal{M}_o - k_o\Delta\bar{\epsilon})g = \mathbb{I}\\
\implies G_o\mathcal{M}_og - G_o\mathcal{V}G = G_o \mathbb{I}\\
\implies g = G_o +G_o\mathcal{V}g
\end{split}
\label{Dyson_equation}
\end{equation}
Rearranging this to solve for $g$,
\begin{equation}
g = (1 - G_0 \mathcal{V})^{-1} G_0
\label{eq:Dyson_equation}
\end{equation}
We assume the field is entirely contained in the subspace spanned by $\{\ket{\mathcal{E}_1}, \ket{\mathcal{E}_2}\}$. We can write the identity operator in this subspace as $\mathcal{I} = \sum_{\mu=1,2} \ket{\mathcal{E}_\mu}\bra{\mathcal{E}_\mu}$.
% Now note that $$G_o\mathcal{V} =(\frac{\ket{\mathcal{E}_1}\bra{\mathcal{E}_1}}{\omega - \tilde{\omega}_1} + \frac{\ket{\mathcal{E}_2}\bra{\mathcal{E}_2}}{\omega - \tilde{\omega}_2}) k_o\Delta\bar{\epsilon}$$

% it is confusing perhaps better is $G =G_o  - \mathcal{V}$ then all we need is to add the $\mathcal{V}$ in the right basis with $G_o$. In the collective basis of the two cavities, $G_o$ is block diagonal,

% $$G_o = \begin{bmatrix}
% \frac{1}{\omega - \omega_1} & 0\\
% 0& \frac{1}{\omega - \omega_2}
% \end{bmatrix}$$
% whereas the role of perturbation from change in permittivity,
% $$\mathcal{V} = \begin{bmatrix}
% V_{11} & V_{12}\\
% V_{21} & V_{22}
% \end{bmatrix}$$
% where $V_{ij} = k_o\bra{\mathcal{E}_i}\Delta\bar{\epsilon}\ket{\mathcal{E}_j}$
% Therefore, the net is $$G = \begin{bmatrix}
% \frac{1}{\omega - \omega_1} -V_{11} & -V_{12}\\
% -V_{21} & \frac{1}{\omega - \omega_2} -V_{22}
% \end{bmatrix}$$

Now, rearrange the Dyson equation in the form, 
\begin{equation}\underbrace{G_o^{-1}(1 - G_0 \mathcal{V})}_{D(\omega)} g = \mathbb{I}
\end{equation}
then 
\begin{equation}
g = D^{-1}(\omega)
\end{equation}
which in the spectral form is
\begin{equation}
    g(\mathbf{r}, \mathbf{r}') = \sum_{\{\mu, \nu\} =1,2} \ket{\mathcal{E}_\mu (\mathbf{r})} [D^{-1}(\omega)]_{\mu\nu} \bra{\mathcal{E}_\nu(\mathbf{r}')}
\end{equation}
with the dynamical matrix being defined as, $$D(\omega) = G_o^{-1} - \mathcal{V} = \begin{bmatrix}
{\omega - \omega_1} -V_{11} & -V_{12}\\
-V_{21} & {\omega - \omega_2} -V_{22}
\end{bmatrix}$$
Let the rescaled frequency for the two cavities be
$\omega_i + V_{ii} \to \tilde{\omega}_i$, making,
$$D(\omega) = \begin{bmatrix}
{\omega - \tilde{\omega}_1} & -V_{12}\\
-V_{21} & {\omega - \tilde{\omega}_2} 
\end{bmatrix}$$
and the interaction term components are $V_{\mu, \nu} = \bra{\mathcal{E}_{\mu}(\mathbf{r})}\ket{\Delta \bar\varepsilon(\mathbf{r}) \mathcal{E}_\nu(\mathbf{r}')}$.

%%%%%%%%%%%%%%%%%%%%%%%%%%%%%%%%%%%%%%%%%%%%%%%%%
\section{Cavity-Waveguide Greens Function}
\label{app: cavity-waveguide}


For the composite system, the Green's function should satisfy,
\begin{equation}
\Big(i\bar{\nabla}\times\ -\frac{\omega}{c}\bar{\varepsilon}_t
(\mathbf{r})\Big) g(\mathbf{r}, \mathbf{r}', \omega) = \frac{\omega}{c}\mathbb{I}_6\delta(\mathbf{r}-\mathbf{r}')
\end{equation}
where the total permittivity can be defined in accordance to Lippmann-Schwinger formulation~\cite{Hughes2004SingleQD, Chen2019GENOME}, 
\begin{equation}
\bar\varepsilon_t(\mathbf r) = \bar{\varepsilon}_b(\mathbf{r}) + \Delta\bar{\varepsilon}_w(\mathbf{r}) + \Delta\bar{\varepsilon}_c(\mathbf r)
\end{equation}
with the waveguide, $\Delta\bar{\varepsilon}_w$, and cavity, $\Delta\bar{\varepsilon}_c$, permittivities being a perturbation in each other's dielectric environment, and $\bar{\varepsilon}_b$ is the background permittivity in the absence of waveguide and cavity.

Under quasi-normal approximation with no cross-coupling between the waveguide modes, one can decompose the GF into the spectral representation as, 

\begin{align}
g(\mathbf r, \mathbf r' , \omega) = \sum_{\{\alpha, \beta\} = \{k, c\}} A_{\alpha, \beta}(\omega)\  \mathcal{E}_{\alpha}(\mathbf{r})\ \mathcal{E}^\dagger_\beta (\mathbf{r}')
\label{appeq: gf_spectral_form}
\end{align} 
where $k$ values represent the distinct propagating waveguide modes of the waveguide, and $c$ represents the stationary cavity mode.

Note that the eigen equation satisfies the two sets of orthogonal modes, i.e., the propagating and stationary ones are different eigen equations~\cite{Cowan2003OpticalBistability}. After all, they are not in a strong coupling regime to share a common mode like the N coupled cavities.
For propagating modes
\begin{equation}
i\bar{\nabla}\times \mathcal{E}_k(\mathbf{r}) =\frac{\omega_k}{c}\underbrace{(\bar{\varepsilon}_b(\mathbf r)+\Delta\bar{\varepsilon}_w
(\mathbf{r}))}_{\bar{\varepsilon}_k} \mathcal{E}_k(\mathbf{r})
\end{equation}
whereas for the stationary modes
\begin{equation}
i\bar{\nabla}\times \mathcal{E}_c(\mathbf{r}) =\frac{\omega_c}{c}\underbrace{(\bar{\varepsilon}_b(\mathbf r)+\Delta\bar{\varepsilon}_c
(\mathbf{r}))}_{\bar{\varepsilon}_c} \mathcal{E}_c(\mathbf{r})
\end{equation}
The normalisation condition for each of them is defined with respect to the permittivity-weighted inner product
\begin{equation}
    \int \mathcal{E}^\dagger_\alpha (\mathbf r) \bar{\varepsilon}_{\alpha}(\mathbf r )\mathcal{E}_{\alpha}(\mathbf r)\ \dd^3 \mathbf r = \mathbb I .
\end{equation}Hence, in general, the Maxwell equation in eigenvalue form is
\begin{equation}i\bar{\nabla}\times \mathcal{E}_\alpha(\mathbf{r}) =\frac{\omega_\alpha}{c}\bar{\varepsilon}_\alpha(\mathbf r) \mathcal{E}_\alpha(\mathbf{r})
\label{appeq:cavity_waveguide_eigenval_eq}
\end{equation}
where $\alpha = \{k,c\}$ and $\bar\varepsilon_k$ is indepedent of the propagting mode wavevector. The Dirac-Delta function is decomposed as, 
\begin{equation}\mathbb{I}_6 \delta(r-r') = \sum_{\alpha = \{k,c\}}\bar{\varepsilon}_\alpha(\mathbf{r})\ \mathcal{E}_\alpha(\mathbf r)\ \mathcal{E}^\dagger_\alpha (\mathbf{r})
\label{appeq: Identity_spectral_form}
\end{equation}

\noindent Plugging the relations~\eqref{appeq: gf_spectral_form} and ~\eqref{appeq: Identity_spectral_form} in the Green's function identity relation,

\begin{widetext}
\begin{equation}
\begin{split}\Big(i\bar{\nabla}\times\ -\frac{\omega}{c}\bar{\varepsilon}_t
(\mathbf{r})\Big) \sum_{\{\alpha, \beta \} = \{k, c\}} A_{\alpha, \beta}(\omega)\  \mathcal{E}_{\alpha}(\mathbf{r})\ \mathcal{E}^\dagger_\beta (\mathbf{r}') = \frac{\omega}{c}\sum_{\alpha =\{k,c\}}\bar{\varepsilon}_\alpha(\mathbf{r})\ \mathcal{E}_\alpha(\mathbf r)\ \mathcal{E}^\dagger_\alpha (\mathbf{r})
\end{split}
\end{equation}
\end{widetext}

\noindent and applying the eigenvalue equation~\eqref{appeq:cavity_waveguide_eigenval_eq},
\begin{widetext}
\begin{equation}\begin{split}
\sum_{\{\alpha, \beta \} = \{k, c\}}\Big(A_{\alpha, \beta}(\omega) \frac{\omega_\alpha}{c}\bar{\varepsilon}_\alpha(\mathbf r) \mathcal{E}_\alpha(\mathbf{r})\ \mathcal{E}^\dagger_\beta (\mathbf{r}') -\frac{\omega}{c}\bar{\varepsilon}_t
(\mathbf{r})  A_{\alpha, \beta}(\omega)\  \mathcal{E}_{\alpha}(\mathbf{r})\ \mathcal{E}^\dagger_\beta (\mathbf{r}')\Big) = \frac{\omega}{c}\sum_{\alpha =\{k,c\}}\bar{\varepsilon}_\alpha(\mathbf{r})\ \mathcal{E}_\alpha(\mathbf r)\ \mathcal{E}^\dagger_\alpha (\mathbf{r})
\end{split}
\end{equation}
\end{widetext}

Now to extract the coefficents, project from left with $\mathcal{E}^\dagger_\mu (\mathbf{r})$ and also, project from right with the permittivity weighing $\bar\varepsilon_{\nu} (\mathbf r')\mathcal{E}_\nu(\mathbf{r}')$,
\begin{widetext}
\begin{equation}
\begin{split}
\sum_{\{\alpha, \beta \} = \{k, c\}}\Big( \underbrace{A_{\alpha, \beta}(\omega) \frac{\omega_\alpha}{c}\mathcal{E}^\dagger_\mu (\mathbf{r})\bar{\varepsilon}_\alpha(\mathbf r) \mathcal{E}_\alpha(\mathbf{r})\ \mathcal{E}^\dagger_\beta (\mathbf{r}') \bar{\varepsilon}_\nu(\mathbf r') \mathcal{E}_\nu(\mathbf{r}')}_{\text{1st}}\\ -\underbrace{\frac{\omega}{c}\mathcal{E}^\dagger_\mu (\mathbf{r})\bar{\varepsilon}_t
(\mathbf{r})  A_{\alpha, \beta}(\omega)\  \mathcal{E}_{\alpha}(\mathbf{r})\ \mathcal{E}^\dagger_\beta (\mathbf{r}')\bar{\varepsilon}_\nu(\mathbf r')\mathcal{E}_\nu(\mathbf{r}')}_{\text{2nd}}\Big) =\\
\frac{\omega}{c}\sum_{\alpha =\{k,c\}}\mathcal{E}^\dagger_\mu (\mathbf{r})\bar{\varepsilon}_\alpha(\mathbf{r})\ \mathcal{E}_\alpha(\mathbf r)\ \mathcal{E}^\dagger_\alpha (\mathbf{r'}) \bar{\varepsilon}_\nu(\mathbf r') \mathcal{E}_\nu(\mathbf{r}')
\end{split}
\label{appeq: mode projection relation}
\end{equation}
\end{widetext}
 \paragraph{Cross-coupling between cavity-waveguide modes: }
For $\mu$ representing all the waveguide modes, $\mu = k$ and $\nu = c$ representing the cavity modes, we can deduce the coefficient responsible for the cross-coupling, $A_{k,c}$. The first term on the LHS has a non-zero value for $\alpha = k$ (by orthogonality condition), under an integral over $r$ and $r'$ it gives,
\begin{widetext}
\begin{equation}\begin{split}\int \int \sum_{\{\alpha, \beta \} = \{k, c\}} A_{\alpha, \beta}(\omega) \frac{\omega_\alpha}{c}\mathcal{E}^\dagger_{\mu=k} (\mathbf{r})\bar{\varepsilon}_\alpha(\mathbf r) \mathcal{E}_\alpha(\mathbf{r})\ \mathcal{E}^\dagger_\beta (\mathbf{r}') \bar{\varepsilon}_{\nu=c}(\mathbf r') \mathcal{E}_{\nu=c}(\mathbf{r}')\ \dd \mathbf r\ \dd \mathbf r' 
% = \sum_{\{ \beta \} = \{k, c\}} A_{k,\beta}(\omega) \frac{\omega_k}{c}\mathcal{E}^\dagger_\mu (\mathbf{r})\bar{\varepsilon}_k(\mathbf r) \mathcal{E}_k(\mathbf{r})\ \mathcal{E}^\dagger_\beta (\mathbf{r}') \mathcal{E}_{\nu=c}(\mathbf{r}')\\
% =\sum_{\{ \beta \} = \{k\}} A_{k,\beta}(\omega) \frac{\omega_k}{c}\mathcal{E}^\dagger_\mu (\mathbf{r})\bar{\varepsilon}_k(\mathbf r) \mathcal{E}_k(\mathbf{r})\ \underbrace{\mathcal{E}^\dagger_\beta (\mathbf{r}') \mathcal{E}_\nu(\mathbf{r}')}_{0} + A_{k,c}(\omega) \frac{\omega_k}{c}\mathcal{E}^\dagger_\mu (\mathbf{r})\bar{\varepsilon}_k(\mathbf r) \mathcal{E}_k(\mathbf{r})\ \mathcal{E}^\dagger_c (\mathbf{r}') \mathcal{E}_c(\mathbf{r}')\\
=A_{k,c}(\omega) \frac{\omega_k}{c}
\end{split}\end{equation}
\end{widetext}
similarly for the same $\mu=k, \nu=c$ condition, the second term gives,
\begin{widetext}
\begin{equation}\begin{split}
\sum_{\{\alpha, \beta \} = \{k, c\}}\frac{\omega}{c}\mathcal{E}^\dagger_{\mu=k} (\mathbf{r})(\bar{\varepsilon}_b(\mathbf{r}) + \Delta\bar{\varepsilon}_w(\mathbf{r}) + \Delta\bar{\varepsilon}_c(\mathbf r))
  A_{\alpha, \beta}(\omega)\  \mathcal{E}_{\alpha}(\mathbf{r})\ \mathcal{E}^\dagger_\beta(\mathbf r') \bar{\varepsilon}_{\nu = c}(\mathbf r') \mathcal{E}_{\nu=c}(\mathbf{r}')
% =\frac{\omega}{c}A_{k, c}(\omega) + \sum_{\{\alpha, \beta \} = \{k, c\}} A_{\alpha, \beta}(\omega)\frac{\omega}{c}\mathcal{E}^\dagger_k (\mathbf{r})(\Delta\bar{\varepsilon}_c(\mathbf r))
%  \  \mathcal{E}_{\alpha}(\mathbf{r})\ \mathcal{E}^\dagger_\beta (\mathbf{r}')\mathcal{E}_c(\mathbf{r}')\\
%   =\frac{\omega}{c}A_{k, c}(\omega) + \sum_{\{\alpha, \beta \} = \{k\}} A_{\alpha, \beta}(\omega)\frac{\omega}{c} \int\mathcal{E}^\dagger_k (\mathbf{r})(\Delta\bar{\varepsilon}_c(\mathbf r))
%  \  \mathcal{E}_{\alpha}(\mathbf{r})d\mathbf{r}\ \mathcal{E}^\dagger_\beta (\mathbf{r}')\mathcal{E}_c(\mathbf{r}') + \sum_{\{\alpha, \beta \} = \{c\}} A_{\alpha, \beta}(\omega)\frac{\omega}{c} \int\mathcal{E}^\dagger_k (\mathbf{r})(\Delta\bar{\varepsilon}_c(\mathbf r))
%  \  \mathcal{E}_{\alpha}(\mathbf{r})d\mathbf{r}\ \mathcal{E}^\dagger_\beta (\mathbf{r}')\mathcal{E}_c(\mathbf{r}')\\
 =\frac{\omega}{c}A_{k, c}(\omega) + A_{cc}(\omega)\frac{\omega}{c} V_{kc}
\end{split}\end{equation}
\end{widetext}
Combining the two, and with the RHS being zero, the first equation is 

\begin{equation}
A_{k,c}(\omega) (\frac{\omega_k-\omega}{c}) - A_{c,c}(\omega)\frac{\omega}{c} \sum_{k} V_{kc} = 0
\label{appeq: kc_cc_relation_1}
\end{equation}
where the interaction term is given by,
\begin{align}
    V_{k,c} = \int \mathcal{E}^\dagger_{k}(\mathbf{r}) \Delta \bar{\varepsilon}_c(\mathbf{r}) \mathcal{E}_c(\mathbf{r})\dd \mathbf r
\end{align}

\paragraph{Intra-cavity mode coupling:} For representing the effect on cavity modes,  $\mu = c$ and $\nu = c$, will define $A_{c,c}$, the first term from~\eqref{appeq: mode projection relation} gives,
\begin{widetext}
\begin{equation}
\begin{split}
\int \int \sum_{\{\alpha, \beta \} = \{k, c\}} A_{\alpha, \beta}(\omega) \frac{\omega_c}{c}\mathcal{E}^\dagger_{\mu=c} (\mathbf{r})\bar{\varepsilon}_c(\mathbf r) \mathcal{E}_\alpha(\mathbf{r})\ \mathcal{E}^\dagger_\beta (\mathbf{r}') \bar{\varepsilon}_{\nu = c} \mathcal{E}_{\nu=c}(\mathbf{r}') \ \dd \mathbf r' \dd \mathbf r = 
A_{c,c}(\omega) \frac{\omega_c}{c}
\end{split}\end{equation}
\end{widetext}
and the second term from~\eqref{appeq: mode projection relation} for $\mu=c=\nu$ is,
\begin{widetext}
\begin{equation}\begin{split}
\sum_{\{\alpha, \beta \} = \{k, c\}}\frac{\omega}{c}\mathcal{E}^\dagger_c (\mathbf{r})(\bar{\varepsilon}_b(\mathbf{r}) + \Delta\bar{\varepsilon}_w(\mathbf{r}) + \Delta\bar{\varepsilon}_c(\mathbf r))
  A_{\alpha, \beta}(\omega)\  \mathcal{E}_{\alpha}(\mathbf{r})\ \mathcal{E}^\dagger_\beta (\mathbf{r}')\mathcal{E}_c(\mathbf{r}')
% =\frac{\omega}{c}A_{c, c}(\omega) + \sum_{\alpha = \{k\}} A_{\alpha, c}(\omega)\frac{\omega}{c}\mathcal{E}^\dagger_c (\mathbf{r})(\Delta\bar{\varepsilon}_c(\mathbf r))
%  \  \mathcal{E}_{\alpha}(\mathbf{r})\ \mathcal{E}^\dagger_c (\mathbf{r}')\mathcal{E}_c(\mathbf{r}')\\
 =\frac{\omega}{c}A_{c, c}(\omega) + A_{k,c}(\omega)\frac{\omega}{c} V_{c,k}
\end{split}\end{equation}
\end{widetext}
and on the RHS, this time we are left with $\omega/c$. Thus, the second equation is,
\begin{equation}
\frac{\omega_c-\omega}{c} A_{c,c}(\omega) - \frac{\omega}{c}A_{k,c}(\omega) \sum_{k} V_{c, k} = \frac{\omega}{c}
\label{appeq: kc_cc_relation_2}
\end{equation}
By Lorentz reciprocity, $V_{c,k} = V_{k,c}$ that is, the interaction between the cavity and waveguide mode is the same irrespective of the direction of transfer of energy.

\noindent Substituting $A_{c,c}$, from \eqref{appeq: kc_cc_relation_1} in\eqref{appeq: kc_cc_relation_2}, gives the cavity-waveguide mode coupling coefficient,
% \begin{equation}
% \frac{(\omega_c - \omega)(\omega_k-\omega)}{\omega \sum_{k} V_{kc}}A_{k,c} - \frac{\omega}{c} \sum_{k} V_{c,k}A_{k,c} = \frac{\omega}{c}
% \end{equation}
% \begin{equation}
% A_{k,c} = \frac{\omega^2 \sum_{k} V_{k,c}}{(\omega_c-\omega)(\omega_k-\omega) - \omega^2 \sum_{k}|V_{k,c}|^2}
% \end{equation}
\begin{equation}
A_{k,c} = \frac{\omega^2 \sum_{k} V_{k,c}}{(\omega_k-\omega)}\times\frac{1}{(\omega_c-\omega) - \frac{\omega^2 \sum_{k} |V_{k,c}|^2}{(\omega_k-\omega)}}
\end{equation}
with $\omega^2 \sum_{k} |V_{k,c}|^2/(\omega_k-\omega) = \Sigma(\omega)$ defining the self-energy due to interaction. And the effect of the waveguide continuum on cavity resonance gives the intra-cavity mode coupling coefficient, 
\begin{align}
A_{c,c} = \frac{\omega}{(\omega_c -\omega) -\Sigma(\omega)}.
\end{align} 

\paragraph{Bare waveguide modes:} For $\mu$ representing all the waveguide modes, $\mu = k$ and $\nu = k'$ also representing the waveguide modes, the first term from~\eqref{appeq: mode projection relation}on the LHS has,
\begin{widetext}
\begin{equation}
\begin{split}\sum_{\{\alpha, \beta \} = \{k, c\}} A_{\alpha, \beta}(\omega) \frac{\omega_\alpha}{c}\mathcal{E}^\dagger_{\mu=k} (\mathbf{r})\bar{\varepsilon}_\alpha(\mathbf r) \mathcal{E}_\alpha(\mathbf{r})\ \mathcal{E}^\dagger_\beta (\mathbf{r}') \bar{\varepsilon}_{\nu=k'}(\mathbf r') \mathcal{E}_{\nu=k'}(\mathbf{r}')
=A_{k,k}\frac{\omega_k}{c}
\end{split}
\end{equation}
\end{widetext}
similarly for the same $\mu=k, \nu=k'$ condition, the second term from~\eqref{appeq: mode projection relation} gives,
\begin{widetext}
\begin{equation}
\begin{split}
\sum_{\{\alpha, \beta \} = \{k, c\}}\frac{\omega}{c}\mathcal{E}^\dagger_k (\mathbf{r})(\bar{\varepsilon}_b(\mathbf{r}) + \Delta\bar{\varepsilon}_w(\mathbf{r}) + \Delta\bar{\varepsilon}_c(\mathbf r))
  A_{\alpha, \beta}(\omega)\  \mathcal{E}_{\alpha}(\mathbf{r})\ \mathcal{E}^\dagger_\beta (\mathbf{r}') \bar{\varepsilon}_{k'}(\mathbf r') \mathcal{E}_{k'}(\mathbf{r}')
  =\frac{\omega}{c}A_{k,k}
  \end{split}
\end{equation}
\end{widetext}

\noindent then equating the LHS and RHS from~\eqref{appeq: mode projection relation},
% \begin{equation}
% \begin{split}
% \frac{\omega_k -\omega}{c}A_{k,k} 
% \end{split}
% \end{equation}
% equating to the RHS,
% \begin{equation}
%  \frac{\omega}{c}\sum_{\alpha =\{k,c\}}\mathcal{E}^\dagger_k (\mathbf{r})\bar{\epsilon}_t(\mathbf{r})\ \mathcal{E}_\alpha(\mathbf r)\ \mathcal{E}^\dagger_\alpha (\mathbf{r'})\bar\varepsilon_k(\mathbf r')\mathcal{E}_k(\mathbf{r}') =\frac{\omega}{c}
% \end{equation}
% Therefore, 
\begin{equation}
A_{k,k} = \frac{\omega}{\omega_k - \omega}
\end{equation}

Therefore, the Greens function for the cavity-waveguide system by combining the three coefficients is,
\begin{widetext}
\begin{equation}
g(\mathbf r, \mathbf r' , \omega) = \sum_{k}\frac{\omega}{\omega_k - \omega}\mathcal{E}_{k}(\mathbf{r})\ \mathcal{E}^\dagger_k (\mathbf{r}') + \sum_{k} \frac{\omega^2 V_{kc}}{(\omega_k-\omega)}\times\frac{1}{(\omega_c-\omega) - \Sigma(\omega)}\  \mathcal{E}_{k}(\mathbf{r})\ \mathcal{E}^\dagger_c (\mathbf{r}') +  \frac{\omega}{(\omega_c -\omega) -\Sigma(\omega)}\mathcal{E}_{c}(\mathbf{r})\ \mathcal{E}^\dagger_c (\mathbf{r}')
\end{equation}
\end{widetext}


% \textbf{old handwavy from:}
% The uncoupled Green's function is block-diagonal in the $\{|k\rangle, |c\rangle\}$ basis, with the bare waveguide being defined only w.r.t the transverse component~\cite{HughesCoupledCavityQED}:
% \begin{equation}
% g_0(\omega) = \underbrace{\sum_k \frac{\omega_k}{\omega_k - \omega} | \mathcal{E}_k \rangle \langle \mathcal{E}_k |}_{\hat{g}_{wg}^{(0)}} + \underbrace{\frac{1}{\omega_c - \omega} | \mathcal{E}_c \rangle \langle \mathcal{E}_c |}_{\hat{g}_{c}^{(0)}}
% \end{equation}
% where the transverse modes of waveguide $\mathcal{E}_k$ satisfy the first-order Maxwell form, \begin{equation}
%     \mathcal{M}_t \mathcal{E}_k = \frac{\omega_k}{c}\bar{\epsilon}_t\mathcal{E}_k
% \end{equation}
% We work with the frequency form as in~\cite{HughesCoupledCavityQED} instead of the wavevector modal form described in Sec.~\ref{sec:waveguide} to facilitate ease of integration with the cavity modal form.
% The coupling operator $W$ represents the interaction between the two. Since it is purely an interaction term between a propagating and one stationary mode, it is strictly off-diagonal in this basis:

% \begin{equation}
% W = \sum_k \left( V_{ck} | \mathcal{E}_c \rangle \langle \mathcal{E}_k | + V_{kc} | \mathcal{E}_k \rangle \langle \mathcal{E}_c | \right)
% \end{equation}
% where $V_{ck}$ is the overlap integral describing how the cavity mode drives the $k$-th waveguide mode.
% Then the Dyson Equation in Matrix Form for the full Green's function $g$ as in Eq.\eqref{eq:Dyson_equation} yields a matrix form,
% \begin{equation}
% \begin{bmatrix} I & -\hat{g}_{wg}^{(0)} \hat{V}^\dagger \\ -\hat{g}_{c}^{(0)} \hat{V} & I \end{bmatrix} 
% \begin{bmatrix} G_{ww} & G_{wc} \\ G_{cw} & G_{cc} \end{bmatrix} = \begin{bmatrix} \hat{g}_{wg}^{(0)} & 0 \\ 0 & \hat{g}_{c}^{(0)} \end{bmatrix}
% \end{equation}

% We are interested in $G_c \equiv G_{cc}$, the projection onto the cavity subspace. From the bottom row of the matrix multiplication:

% $$-\hat{g}_{c}^{(0)} \hat{V} G_{wc} + G_{cc} = \hat{g}_{c}^{(0)}$$

% From the top row (looking at the second column):

% $$G_{wc} - \hat{g}_{wg}^{(0)} \hat{V}^\dagger G_{cc} = 0 \implies G_{wc} = \hat{g}_{wg}^{(0)} \hat{V}^\dagger G_{cc}$$
%  Solving for $G_c$

% Substitute the expression for $G_{wc}$ back into the first equation:

% $$-\hat{g}_{c}^{(0)} \hat{V} \left( \hat{g}_{wg}^{(0)} \hat{V}^\dagger G_{cc} \right) + G_{cc} = \hat{g}_{c}^{(0)}$$

% Factor out $G_{cc}$:

% $$\left( I - \hat{g}_{c}^{(0)} \hat{V} \hat{g}_{wg}^{(0)} \hat{V}^\dagger \right) G_{cc} = \hat{g}_{c}^{(0)}$$

% $$G_{cc} = \left( I - \hat{g}_{c}^{(0)} \hat{V} \hat{g}_{wg}^{(0)} \hat{V}^\dagger \right)^{-1} \hat{g}_{c}^{(0)}$$

% Recovering the Self-Energy Form,

% Since $\hat{g}_{c}^{(0)} = \frac{1}{\omega_c - \omega}$, we can multiply through by the inverse of $\hat{g}_{c}^{(0)}$ (which is just the scalar $\omega_c - \omega$):

% $$G_c(\omega) = \frac{1}{(\omega_c - \omega) - \hat{V} \hat{g}_{wg}^{(0)} \hat{V}^\dagger}$$

% Now, substitute your explicit form for $\hat{g}_{wg}^{(0)}$ into the denominator:

% $$\Sigma(\omega) = \hat{V} \hat{g}_{wg}^{(0)} \hat{V}^\dagger = \sum_k \langle \mathcal{E}_c | W | \mathcal{E}_k \rangle \left( \frac{\omega_k}{\omega_k - \omega} \right) \langle \mathcal{E}_k | W | \mathcal{E}_c \rangle$$

% $$\Sigma(\omega) = \sum_k \frac{\omega_k |V_{ck}|^2}{\omega_k - \omega}$$

% Therefore, the final Dressed Green's Function,

% Combining the terms, we arrive at the result consistent with Equation (69) in your text:

% $$G_c(\omega) = \frac{1}{\omega_c - \omega - \Sigma(\omega)}$$



% %%%%%%%%%%%%%%%%%%%%%%%%%%%%%%%%%%%%%%%%%%%%
% \section{Cavity--Waveguide Composites}
% \label{sec:composite}
% %%%%%%%%%%%%%%%%%%%%%%%%%%%%%%%%%%%%%%%%%%%%

% Section~\ref{sec:beyond} treated coupled discrete resonances.  Here we consider the structurally distinct case in which one or more cavity modes interact with a waveguide continuum.  The waveguide contributes a branch-cut continuum rather than isolated poles; eliminating it dresses the cavity poles with a frequency-dependent self-energy.  The quantum input--output relation~\eqref{eq:quantum_io} applies unchanged---only the representation of the Green function changes.

% \paragraph{Self-energy and Markov limit.}
% \label{sec:cav_wg}

% Consider a discrete cavity resonance coupled to a waveguide continuum---the geometry underlying side-coupled ring resonators, photonic-crystal defect modes, and cavity QED in a waveguide.  Before the two subsystems interact, the Green function decomposes as
% \begin{equation}
% g_0(\mathbf{r},\mathbf{r}',\omega) = g_\mathrm{wg}^{(0)}(\mathbf{r},\mathbf{r}',\omega) + \frac{\mathcal{E}_c(\mathbf{r})\,\mathcal{E}_c^\dagger(\mathbf{r}')}{\omega - \tilde\omega_c},
% \label{eq:bare_decomp}
% \end{equation}
% where $g_\mathrm{wg}^{(0)}$ is the bare waveguide Green function from Sec.~\ref{sec:wg_green} and $\tilde\omega_c = \omega_c - i\kappa_i/2$ is the intrinsic cavity frequency.  The coupling is treated exactly by a Dyson equation: letting $W$ denote the coupling operator between the cavity and waveguide subspaces, the full Green function satisfies $g = g_0 + g_0\,W\,g$.  Projecting onto the cavity subspace yields the dressed cavity Green function
% \begin{equation}
% G_c(\omega) = \frac{1}{\omega - \omega_c - \Sigma(\omega)},
% \label{eq:dressed_cavity}
% \end{equation}
% where the self-energy
% \begin{equation}
% \Sigma(\omega) = \sum_n \frac{|V_{cn}|^2}{\omega - \omega_n + i0^+}
% \label{eq:self_energy}
% \end{equation}
% encodes the effect of the waveguide continuum on the cavity, with $V_{cn}$ the coupling amplitude to the $n$th waveguide mode.  Using the Sokhotski--Plemelj identity, the self-energy separates into a Lamb-shift-like frequency renormalization and a waveguide-induced decay rate,
% \begin{equation}
% \Sigma(\omega) = \Delta_\mathrm{L}(\omega) - i\frac{\Gamma_\mathrm{wg}(\omega)}{2},
% \label{eq:self_energy_split}
% \end{equation}
% where $\Delta_\mathrm{L}(\omega) = \mathcal{P}\sum_n |V_{cn}|^2/(\omega - \omega_n)$ and
% \begin{equation}
% \Gamma_\mathrm{wg}(\omega) = 2\pi \sum_\alpha \frac{|V_{c,k_\alpha}|^2}{|v_g(k_\alpha)|}, \qquad \omega_{k_\alpha} = \omega.
% \label{eq:gamma_wg}
% \end{equation}
% The factor $1/|v_g|$ is the waveguide density of states: a slow-light mode enhances the cavity decay rate, in direct analogy with the Purcell effect.

% Solving the Dyson equation for the full Green function gives the cavity-mediated correction to the bare waveguide propagator,
% \begin{multline}
% g(\omega) \approx g_\mathrm{wg}^{(0)}(\omega) \\
% + g_\mathrm{wg}^{(0)}(\omega)\,W\,G_c(\omega)\,W^\dagger\,g_\mathrm{wg}^{(0)}(\omega),
% \label{eq:full_cav_wg_green}
% \end{multline}
% a rank-one (separable) modification of $g_\mathrm{wg}^{(0)}$ whose pole is the dressed cavity resonance.

% When the cavity linewidth is narrow compared to the scale on which $\Sigma(\omega)$ varies, the self-energy may be evaluated at the bare cavity frequency (the Markov approximation), giving
% \begin{equation}
% G_c(\omega) \approx \frac{1}{\omega - \omega_c - \Delta_\mathrm{L} + i(\kappa_i + \kappa_\mathrm{wg})/2},
% \label{eq:markov_cavity}
% \end{equation}
% with $\kappa_\mathrm{wg} = \Gamma_\mathrm{wg}(\omega_c)$.  The waveguide transmission amplitude then takes the canonical form
% \begin{multline}
% t(\omega) = 1 \\
% - \frac{\kappa_\mathrm{wg}}{i(\omega - \omega_c - \Delta_\mathrm{L}) + (\kappa_i + \kappa_\mathrm{wg})/2},
% \label{eq:tcmt_transmission}
% \end{multline}
% reproducing the standard result of temporal coupled-mode theory~\cite{fan2003temporal,suh2004temporal}.  Substituting the dressed $g$ from~\eqref{eq:full_cav_wg_green} into the quantum input--output relation~\eqref{eq:quantum_io} yields the quantum version, with Langevin noise determined by the optical theorem.


% \paragraph{Multiport extension.}
% \label{sec:cav_two_wg}

% For a cavity coupled to two distinct waveguide channels---the geometry of add--drop filters and ring resonators with bus and drop ports---each waveguide contributes an independent self-energy, so the dressed cavity Green function generalizes to
% \begin{equation}
% G_c(\omega) = \frac{1}{\omega - \omega_c - \Sigma_1(\omega) - \Sigma_2(\omega)}.
% \label{eq:dressed_cavity_two_wg}
% \end{equation}
% The scattering matrix element connecting input channel $n$ on waveguide $b$ to output channel $m$ on waveguide $a$ is
% \begin{multline}
% S_{mn}^{(ab)}(\omega) = \delta_{ab}\,S_{mn}^{(a,\mathrm{direct})} \\
% + \frac{d_m^{(a)}\,c_n^{(b)}}{\omega - \omega_c - \Sigma_1 - \Sigma_2},
% \label{eq:S_two_wg}
% \end{multline}
% where $c_n^{(b)}$ and $d_m^{(a)}$ are the input and output coupling amplitudes.  For a side-coupled ring resonator with no direct path between bus and drop ports, $S^{(12,\mathrm{direct})} = 0$ and the drop-port transmission is purely cavity-mediated:
% \begin{equation}
% t_\mathrm{drop}(\omega) = \frac{\sqrt{\kappa_1\kappa_2}}{i(\omega - \omega_c) + (\kappa_i + \kappa_1 + \kappa_2)/2}.
% \label{eq:drop_transmission}
% \end{equation}
% This is the standard add--drop result~\cite{fan2003temporal}, here derived directly from the Green function.  The quantum version follows from~\eqref{eq:quantum_io}, with the Langevin noise compensating the non-unitarity of the multiport scattering matrix due to intrinsic loss.


% \paragraph{Waveguide-mediated cavity coupling.}
% \label{sec:two_cav_one_wg}

% When two cavities couple to a shared waveguide continuum, eliminating the waveguide degrees of freedom via the Dyson equation produces a \emph{matrix-valued} self-energy $[\Sigma_\mathrm{wg}(\omega)]_{\mu\nu}$.  The two-cavity Green function is
% \begin{equation}
% G_\mathrm{cav}(\omega) = \bigl[\omega I - H_\mathrm{cav} - \Sigma_\mathrm{wg}(\omega)\bigr]^{-1},
% \label{eq:dressed_two_cav}
% \end{equation}
% where
% \begin{equation}
% [\Sigma_\mathrm{wg}(\omega)]_{\mu\nu} = \sum_n \frac{V_{\mu n}\,V_{\nu n}^*}{\omega - \omega_n + i0^+}.
% \label{eq:matrix_self_energy}
% \end{equation}
% The diagonal elements dress each cavity individually (Lamb shift plus waveguide-induced linewidth), while the off-diagonal element $[\Sigma_\mathrm{wg}]_{12} = J_\mathrm{wg}(\omega) - i\Gamma_{12}(\omega)/2$ provides two new effects: a waveguide-mediated coherent coupling $J_\mathrm{wg}$ that adds to the direct coupling $J$, and a collective dissipative coupling $\Gamma_{12}$ through which the two cavities decay cooperatively into the shared continuum---the photonic analogue of super- and subradiance~\cite{dicke1954coherence}.

% In the Markov limit, the total effective Hamiltonian $H_\mathrm{eff} = H_\mathrm{cav} + \Sigma_\mathrm{wg}$ reduces to
% \begin{widetext}
% \begin{equation}
% H_\mathrm{eff} = \begin{pmatrix} \omega_1 - i(\kappa_{1,i} + \kappa_{1,\mathrm{wg}})/2 & J + J_\mathrm{wg} - i\Gamma_{12}/2 \\ J + J_\mathrm{wg} - i\Gamma_{12}/2 & \omega_2 - i(\kappa_{2,i} + \kappa_{2,\mathrm{wg}})/2 \end{pmatrix},
% \label{eq:Heff_markov_two_cav}
% \end{equation}
% \end{widetext}
% which has exactly the structure of the phenomenological Hamiltonian~\eqref{eq:Heff_coupled} introduced in Sec.~\ref{sec:beyond}, but now the couplings and linewidths are determined microscopically by the cavity--waveguide coupling amplitudes and waveguide dispersion.  The full composite Green function is
% \begin{multline}
% g(\mathbf{r},\mathbf{r}',\omega) \approx g_\mathrm{wg}^{(0)}(\mathbf{r},\mathbf{r}',\omega) \\
% + \sum_{\mu,\nu=1}^{2} \mathcal{U}_\mu(\mathbf{r},\omega)\,\bigl[G_\mathrm{cav}(\omega)\bigr]_{\mu\nu}\,\mathcal{U}_\nu^\dagger(\mathbf{r}',\omega),
% \label{eq:full_two_cav_wg}
% \end{multline}
% where $\mathcal{U}_\mu(\mathbf{r},\omega) = \int g_\mathrm{wg}^{(0)}(\mathbf{r},\mathbf{r}'')\,W_\mu(\mathbf{r}'')\,dV''$ is the cavity mode profile dressed by waveguide propagation---the rank-two generalization of~\eqref{eq:full_cav_wg_green}.

% Beyond the Markov regime, near photonic band edges where $v_g \to 0$ the density of states diverges and $\Sigma(\omega)$ acquires strong frequency dependence on the scale of the cavity linewidth.  This produces asymmetric Fano lineshapes~\cite{fano1961effects} from interference between the direct and cavity-mediated paths, and can lead to cavity-photon bound states~\cite{john1994quantum} when the cavity frequency lies inside a bandgap ($\Gamma_\mathrm{wg} = 0$).  Throughout this regime, the Dyson form~\eqref{eq:full_cav_wg_green} and the quantum input--output relation~\eqref{eq:quantum_io} remain valid; what changes is only the complexity of $\Sigma(\omega)$.



%%%%%%%%%%%%%%%%%%%%%%%%%%%%%%%%%%%%%%%%%%%%
\section{Single-emitter decay in the first-order input--output formalism}
\label{app:single_emitter}
%%%%%%%%%%%%%%%%%%%%%%%%%%%%%%%%%%%%%%%%%%%%
We derive the Heisenberg--Langevin equations for a single two-level emitter in an arbitrary photonic environment that may include cavities, waveguides, or absorbing media.  Three processes govern the emitter dynamics: the atom interacts with its own retarded self-field, which produces the radiative decay rate and frequency shift; it is driven by vacuum fluctuations propagated from the boundary; and, in a lossy medium, it is driven by Langevin polarization noise from the absorbing bulk.  The generalized optical theorem connects these three contributions, guaranteeing that the total noise strength equals the dissipation rate.  

Consider a two-level emitter at position $\mathbf{r}_A$, with excited state $|e\rangle$, ground state $|g\rangle$, transition frequency $\omega_A$, and lowering operator
\begin{equation}
\hat\sigma = |g\rangle\langle e|,
\qquad
\hat\sigma^\dagger = |e\rangle\langle g|.
\end{equation}
The atomic Hamiltonian is
\begin{equation}
\hat H_A = \hbar \omega_A \, \hat\sigma^\dagger \hat\sigma = \frac{\hbar\omega_A}{2}(1+\hat\sigma_z).
\end{equation}
The dipole operator is
\begin{equation}
\hat{\mathbf{d}} = \mathbf{d}\,\hat\sigma + \mathbf{d}^*\,\hat\sigma^\dagger,
\end{equation}
and the interaction Hamiltonian in the rotating-wave and electric-dipole approximations is
\begin{equation}
\hat H_{\mathrm{int}}
\simeq
- \mathbf{d}^*\cdot \hat{\mathbf{E}}^{(+)}(\mathbf{r}_A)\,\hat\sigma^\dagger
- \mathbf{d}\cdot \hat{\mathbf{E}}^{(-)}(\mathbf{r}_A)\,\hat\sigma.
\end{equation}

From $\dot O = (i/\hbar)[\hat H,O]$ and using $[\hat\sigma_z, \hat\sigma] = -2\hat\sigma$, $[\hat\sigma_z, \hat\sigma^\dagger] = 2\hat\sigma^\dagger$
and $[\hat\sigma^\dagger, \hat\sigma] = \hat\sigma_z$, one obtains
\begin{equation}
\dot{\hat\sigma}(t)
=
-i\omega_A\hat\sigma(t)
- \frac{i}{\hbar}\,\mathbf{d}^*\cdot \hat{\mathbf{E}}^{(+)}(\mathbf{r}_A,t)\,\hat\sigma_z(t),
\end{equation}
\begin{multline}
\dot{\hat\sigma}_z(t)
=
\frac{2i}{\hbar}
\Big[
\mathbf{d}^*\cdot \hat{\mathbf{E}}^{(+)}(\mathbf{r}_A,t)\,\hat\sigma^\dagger(t)-
\\\mathbf{d}\cdot \hat{\mathbf{E}}^{(-)}(\mathbf{r}_A,t)\,\hat\sigma(t)
\Big].
\end{multline}
At this point nothing has been approximated beyond the rotating-wave and dipole approximations.


To connect the atomic dynamics to the input--output formalism of~\cite{partI}, we express the field at the emitter in terms of the first-order fields and Green kernel.  The quantum field at the emitter position receives three contributions: the boundary input field propagated inward by the retarded Green kernel, the emitter's own retarded self-field, and, in a lossy medium, the Langevin polarization noise propagated from the absorbing bulk.  In the frequency domain,
\begin{equation}
\hat{\mathcal{E}}(\mathbf{r}_A,\omega)
=
\hat{\mathcal{E}}_{\mathrm{in}}(\mathbf{r}_A,\omega)
+
\hat{\mathcal{E}}_{\mathrm{self}}(\mathbf{r}_A,\omega)
+
\hat{\mathcal{E}}_P(\mathbf{r}_A,\omega),
\end{equation}
The three terms are
\begin{equation}\label{eq:three_terms}
\begin{aligned}
\hat{\mathcal{E}}_{\mathrm{in}}(\mathbf{r}_A,\omega)
&=
-i\oint_S dS\; g(\mathbf{r}_A,\mathbf{s},\omega)\,
(\bar{n}\times)\,
\hat{\mathcal{E}}_{\mathrm{in}}(\mathbf{s},\omega),
\\
\hat{\mathcal{E}}_{\mathrm{self}}(\mathbf{r}_A,\omega)
&=
g(\mathbf{r}_A,\mathbf{r}_A,\omega)\,\mathcal{D}\,\hat\sigma(\omega),
\\
\hat{\mathcal{E}}_P(\mathbf{r}_A,\omega)
&=
-ik_0\!\int_V dV'\; g(\mathbf{r}_A,\mathbf{r}',\omega)\,
\hat{\mathcal{P}}_N(\mathbf{r}',\omega).
\end{aligned}
\end{equation}
Although the emitter couples only to the electric-field block of $\hat{\mathcal{E}}$, both $\mathbf{E}$ and $\mathbf{H}$ components of the boundary and bulk fields contribute to the propagated field at $\mathbf{r}_A$.  The dipole coupling to the dual field is captured by the coupling vector $\mathcal{D} = [\mathbf{d},\,\mathbf{0}]^T$, so that $\mathbf{d}^*\!\cdot\hat{\mathbf{E}}^{(+)} = \mathcal{D}^\dagger\hat{\mathcal{E}}$.

Substituting the three-term decomposition into the Heisenberg equations, the field enters only through the scalar contractions $\mathcal{D}^\dagger\hat{\mathcal{E}}_{\mathrm{in}}$, $\mathcal{D}^\dagger\hat{\mathcal{E}}_{\mathrm{self}}$, and $\mathcal{D}^\dagger\hat{\mathcal{E}}_P$.  We define three time-domain quantities, one for each contribution:
\begin{align}
&\hat F(t)
\equiv
\frac{1}{\hbar}\,\mathcal{D}^\dagger \hat{\mathcal{E}}_{\mathrm{in}}(\mathbf{r}_A,t)
\\
\notag
&=-\frac{i}{\hbar}\oint_S dS\int_0^\infty \frac{d\omega}{2\pi}\; \mathcal{D}^\dagger g(\mathbf{r}_A,\mathbf{s})\,
(\bar{n}\times)\,
\hat{\mathcal{E}}_{\mathrm{in}}(\mathbf{s}) e^{-i\omega t},
\label{eq:F_def}
\\
&\hat P(t)
\equiv
\frac{1}{\hbar}\,\mathcal{D}^\dagger \hat{\mathcal{E}}_P(\mathbf{r}_A,t).
\\
\notag
&=-\frac{ik_0}{\hbar}\!\int_V dV' \int_0^\infty \frac{d\omega}{2\pi} \mathcal{D}^\dagger g(\mathbf{r}_A,\mathbf{r}')\,
\hat{\mathcal{P}}_N(\mathbf{r}')e^{-i\omega t}.
\label{eq:P_def}
\end{align}
\begin{equation}
    K(\omega)
\equiv
\frac{i}{\hbar}\,\mathcal{D}^\dagger\, g(\mathbf{r}_A,\mathbf{r}_A,\omega)\,\mathcal{D}
\label{eq:K_def}
\end{equation}
Transforming $\frac{i}{\hbar} \mathcal{D}^\dagger\hat{\mathcal{E}}_{\mathrm{self}}(\mathbf r_A, \omega)=K(\omega)\sigma(\omega)$ to time domain, 
\begin{equation}
K(\omega)\sigma(\omega)\rightarrow \int_0^t d\tau K(t-\tau) \sigma(\tau) 
\end{equation}
% \begin{equation}
%     K(t)
% \equiv
% \frac{i}{\hbar}\,\mathcal{D}^\dagger\, g(\mathbf{r}_A,\mathbf{r}_A,t)\,\mathcal{D},
% \quad K(t)=0\;(t<0),
% \label{eq:K_def}
% \end{equation}
\ishita{mention subtelty about the positive frequency part}
Here $\hat F$ is the Langevin force from the boundary input field, $K$ is the retarded memory kernel encoding the self-field, and $\hat P$ is the Langevin force from bulk absorption noise.  In terms of these quantities the exact non-Markovian Heisenberg--Langevin equations are
\begin{multline}
\dot{\hat\sigma}(t)
=
-i\omega_A \hat\sigma(t)
-
i\bigl[\hat F(t)+\hat P(t)\bigr]\hat\sigma_z(t)
\\
-
\hat\sigma_z(t)\int_0^t d\tau\,K(t-\tau)\hat\sigma(\tau)\,,
\end{multline}
and
\begin{align}
\dot{\hat\sigma}_z(t)
&=
2i\bigl[\hat F(t)+\hat P(t)\bigr]\hat\sigma^\dagger(t)
\notag\\
&\qquad
+
2\;\hat\sigma^\dagger(t)\int_0^t \!d\tau
K(t\!-\!\tau)\hat\sigma(\tau) +\text{h.c.}
\end{align}
At this stage the dynamics is exact and non-Markovian; all three contributions enter on equal footing.  In a lossless environment $\hat P=0$ and the equations reduce to the two-term form.




\paragraph{Markov approximation.}

To make the equations local in time we invoke the Markov approximation: when the reservoir correlation time is much shorter than the emitter dynamics, the memory kernel acts as a delta function,
\begin{equation}\label{eq:markov-kernel}
K(t-\tau)
\;\longrightarrow\;
\left(-\frac{\Gamma_{\mathrm{self}}}{2} - i\Delta\right)\delta(t-\tau),
\end{equation}
where
\begin{equation}\label{eq:self-energy}
\frac{-\Gamma_{\mathrm{self}}}{2} - i\Delta
\;\equiv\;
\int_0^\infty ds\, K(s)\,e^{i\omega_A s}
\end{equation}
is the one-sided Fourier transform of the kernel evaluated at the emitter frequency.  Here $\Gamma_{\mathrm{self}}$ is the radiative decay rate generated by the self-field and $\Delta$ is the corresponding Lamb shift.  The convolution collapses to a local term, $\int_0^t d\tau\,K(t-\tau)\hat\sigma(\tau)\to(-\Gamma_{\mathrm{self}}/2 - i\Delta)\,\hat\sigma(t)$, and the equations become
\begin{multline}
\dot{\hat\sigma}(t)
=
-\left[i\omega_A+\big(i\Delta+\frac{\Gamma_{\mathrm{self}}}{2}\big)\hat{\sigma}_z(t)\right]\hat\sigma(t)
\\
-\,
i\bigl[\hat F(t)+\hat P(t)\bigr]\hat\sigma_z(t),\\
% =-i\omega_A\sigma(t)-\big(i\Delta+\frac{\Gamma_{\mathrm{self}}}{2}\big)\hat\sigma(t)\\
% =-\,
% i\bigl[\hat F(t)+\hat P(t)\bigr]\hat\sigma_z(t),\\
=-\Big(i(\omega_A+\Delta)+\frac{\Gamma_{\mathrm{self}}}{2}\Big)\hat\sigma(t)
\\
-\,
i\bigl[\hat F(t)+\hat P(t)\bigr]\hat\sigma_z(t),
\end{multline}
\begin{multline}
\dot{\hat\sigma}_z(t)
=
-\Gamma_{\mathrm{self}}\,(1+\hat\sigma_z(t))\,
\\
-\,
2i\bigl[\hat F^\dagger(t)+\hat P^\dagger(t)\bigr]\hat\sigma(t)
+
2i\bigl[\hat F(t)+\hat P(t)\bigr]\hat\sigma^\dagger(t).
\end{multline}

Although $\hat F$, $K$, and $\hat P$ are defined through independent physical processes (boundary input, self-field, and bulk absorption), they are not independent: the generalized optical theorem connects them.  The imaginary part of the Green kernel at the emitter position decomposes as
\begin{equation}\label{eq:gen-optical-thm}
\mathrm{Im}\,g(\mathbf{r}_A,\mathbf{r}_A,\omega)
=
\mathrm{Im}\,g\big|_{\mathrm{boundary}}
+
\mathrm{Im}\,g\big|_{\mathrm{absorption}},
\end{equation}
so the total decay rate $\Gamma_{\mathrm{self}}\propto \mathcal{D}^\dagger\,\mathrm{Im}\,g(\mathbf{r}_A,\mathbf{r}_A,\omega_A)\,\mathcal{D}$ receives contributions from radiation through the boundary and from absorption in the bulk, exactly the two channels that supply the Langevin forces $\hat F$ and $\hat P$.  Energy leaving the emitter via the self-field is balanced by fluctuations entering through the same two channels, ensuring the commutator algebra is preserved.




\paragraph{Mean-field dynamics and the role of vacuum fluctuations.}

Because $\hat F$ is built from the freely propagated boundary input field, $\langle\hat F\rangle=0$ for vacuum input.
In the Markov limit the input field at time $t$ is uncorrelated with the system state at time $t$, so the noise terms drop out of first moments and we obtain
\begin{align}
\frac{d}{dt}\langle\hat\sigma\rangle
&=
-\left[i(\omega_A+\Delta)+\frac{\Gamma_{\mathrm{self}}}{2}\right]\langle\hat\sigma\rangle,
\\
\frac{d}{dt}\langle\hat\sigma_z\rangle
&=
-\Gamma_{\mathrm{self}}\bigl(1+\langle\hat\sigma_z\rangle\bigr).
\end{align}
For vacuum input an initially excited emitter therefore obeys $\langle\hat\sigma_z(t)\rangle=-1+2e^{-\Gamma_{\mathrm{self}}t}$: spontaneous emission is already visible in the deterministic drift.  Likewise, $\langle\hat P\rangle=0$ for a medium in its ground state, so the mean-field equations are identical in the lossy and lossless cases.

\paragraph{Fluctuation-dissipation closure.}

Although the mean-field dynamics is self-contained, the fluctuation operators $\hat F$ and $\hat P$ are not dispensable.  The exact two-level algebra requires $[\hat\sigma^\dagger,\hat\sigma]=\hat\sigma_z$ at all times.  If the Langevin forces are discarded while the Markov damping is retained, the damping-only equation $\dot{\hat\sigma}=-(\Gamma_{\mathrm{self}}/2+i(\omega_A+\Delta))\hat\sigma$ implies
\begin{equation}\label{eq:comm-decay}
[\hat\sigma(t),\hat\sigma^\dagger(t)] = e^{-\Gamma_{\mathrm{self}}t}\,[\hat\sigma(0),\hat\sigma^\dagger(0)],
\end{equation}
so the commutator decays exponentially to zero.  Using the full Markov equations to compute $\tfrac{d}{dt}[\hat\sigma,\hat\sigma^\dagger]$, the damping produces a term $-\Gamma_{\mathrm{self}}[\hat\sigma,\hat\sigma^\dagger]$, while the noise terms produce a correction proportional to $\langle\hat F(t)\hat F^\dagger(t')\rangle + \langle\hat P(t)\hat P^\dagger(t')\rangle$.  Commutator preservation therefore demands that the total noise strength equal the dissipation rate.

This can be verified explicitly.  Defining the boundary operator $\hat B(\mathbf{s},\omega) \equiv (\bar{n}\times)\hat{\mathcal{E}}_{\mathrm{in}}(\mathbf{s},\omega)$, the force operator is $\hat F(\omega) = -(i/\hbar)\oint_S dS\;\mathcal{D}^\dagger g(\mathbf{r}_A,\mathbf{s},\omega)\,\hat B(\mathbf{s},\omega)$.  For vacuum input $\langle\hat B^\dagger\hat B\rangle=0$, so the correlator reduces to the boundary commutator,
\begin{multline}
[\hat B_i(\mathbf{s},\omega),\hat B_j^\dagger(\mathbf{s}',\omega')]
\\
=
-\frac{\hbar k_0}{2\pi\varepsilon_0}\,
(\bar{n}\times)_{ij}\,
\delta^{(2)}(\mathbf{s}-\mathbf{s}')\,\delta(\omega-\omega'),
\end{multline}
which after substitution gives
\begin{multline}\label{eq:FF-surface}
[ \hat F(\omega)\hat F^\dagger(\omega')]
=
-\frac{k_0}{2\pi\varepsilon_0\hbar}\,
\delta(\omega-\omega')
\\
\times\mathcal{D}^\dagger
\left[
\oint_S dS\; g(\mathbf{r}_A,\mathbf{s},\omega)\,(\bar{n}\times)\,g^\dagger(\mathbf{s},\mathbf{r}_A,\omega)
\right]\mathcal{D}.
\end{multline}
which contains the boundary term of the generalized optical theorem~\eqref{eq:gen-optical-thm} inside the scalar contraction $\mathcal{D}^\dagger(\cdots)\mathcal{D}$, yielding
\begin{multline}\label{eq:FF-Img}
[ \hat F(\omega)\hat F^\dagger(\omega')]
=
\frac{1}{\hbar^2}\,
\delta(\omega-\omega')
\mathcal{D}^\dagger\,\mathrm{Im}\,g\big|_{\mathrm{bdy}}\,\mathcal{D}.
\end{multline}
where
\begin{equation}
    \mathrm{Im}\,g\big|_{\mathrm{bdy}}=-\frac{\hbar k_0}{2\pi \varepsilon_0}
\oint g(\mathbf{r}_A,s)\,
(\bar{n}\!\times)g^\dagger(s,\mathbf{r}_A)\,dS\;
\end{equation}
An analogous calculation gives $\langle\hat P(\omega)\hat P^\dagger(\omega')\rangle\propto\mathcal{D}^\dagger\,\mathrm{Im}\,g|_{\mathrm{absorption}}\,\mathcal{D}$.  Adding the two reproduces the full $\mathrm{Im}\,g(\mathbf{r}_A,\mathbf{r}_A,\omega)$, so
\begin{equation}\label{eq:FD-closure}
\Gamma_F + \Gamma_P = \Gamma_{\mathrm{self}} \equiv \Gamma.
\end{equation}
Henceforth we write simply $\Gamma$ for the common rate.  The self-field kernel produces $\Gamma$ and the Lamb shift $\Delta$; the boundary and absorption channels produce the Langevin forces $\hat F$ and $\hat P$; and the optical theorem ties them together, guaranteeing that the noise strength matches the dissipation rate.  The single-emitter spontaneous-emission law $P_e(t)=e^{-\Gamma t}$ and the preservation of $[\hat\sigma,\hat\sigma^\dagger]=-\hat\sigma_z$ both follow from this consistency.  In a lossless medium $\Gamma_P=0$ and the balance reduces to $\Gamma_F=\Gamma$.
\paragraph{Transmission}
\ishita{need to add transmission derivation. all the equations in this section make sense (I think?) but i need to rewrite all of it}

\section{Multi-emitter transmission.}
\label{app:multi_emitter_transmission}

We now generalize to $N$ emitters at positions $\{\mathbf{r}_j\}_{j=1}^N$ with coupling vectors $\mathcal{D}_j = [\mathbf{d}_j,\,\mathbf{0}]^T$.  The field at emitter $j$ receives the same three contributions as in the single-emitter case---boundary input, self-fields, and (in a lossy medium) polarization noise---except that the self-field sum now runs over all emitters:
\begin{multline}\label{eq:field_at_j}
\hat{\mathcal{E}}(\mathbf{r}_j,\omega)
=
\hat{\mathcal{E}}_{\mathrm{in}}(\mathbf{r}_j,\omega)
\\
+
\sum_{k=1}^N
g(\mathbf{r}_j,\mathbf{r}_k,\omega)\,\mathcal{D}_k\,\hat\sigma_k(\omega)
+
\hat{\mathcal{E}}_P(\mathbf{r}_j,\omega).
\end{multline}
This decomposition is exact in the frequency domain and does not invoke the Markov approximation.  The Heisenberg equations for each emitter have the same form as the single-emitter equations above, with $j$ indices on all operators.

In the low-saturation regime we set $\hat\sigma_{z,j}\simeq -1$, which linearizes the equations and allows us to work entirely in the frequency domain.  Unlike the single-emitter Markov approximation above, no approximation is made on the reservoir correlation time: the Green matrix $G_{jk}(\omega)$ retains its full frequency dependence.  The linearized equation for emitter $j$ reads
\begin{equation}
(\omega-\omega_A)\hat\sigma_j(\omega)
=
-\frac{1}{\hbar}\,\mathcal{D}_j^\dagger\hat{\mathcal{E}}(\mathbf{r}_j,\omega).
\end{equation}
Substituting the field decomposition~\eqref{eq:field_at_j} and defining the projected Green matrix
\begin{equation}
G_{jk}(\omega)
\equiv
\frac{1}{\hbar}\,\mathcal{D}_j^\dagger\, g(\mathbf{r}_j,\mathbf{r}_k,\omega)\,\mathcal{D}_k,
\end{equation}
and the total drive (boundary input plus polarization noise),
\begin{equation}
\hat\eta_j(\omega)
\equiv
\frac{1}{\hbar}\,\mathcal{D}_j^\dagger\bigl[\hat{\mathcal{E}}_{\mathrm{in}}(\mathbf{r}_j,\omega)
+
\hat{\mathcal{E}}_P(\mathbf{r}_j,\omega)\bigr],
\end{equation}
gives the linear system
\begin{equation}\label{eq:linear_system}
\sum_{k=1}^N
\left[
(\omega-\omega_A)\delta_{jk}+G_{jk}(\omega)
\right]
\hat\sigma_k(\omega)
=
-\hat\eta_j(\omega).
\end{equation}
The diagonal element $G_{jj}$ is the single-emitter self-energy whose Markov limit was analyzed above; the off-diagonal elements $G_{jk}$ ($j\neq k$) encode the retarded dipole-dipole coupling mediated by the full photonic Green kernel.  Both noise contributions have zero expectation value ($\langle\hat{\mathcal{E}}_{\mathrm{in}}\rangle = \langle\hat{\mathcal{E}}_P\rangle = 0$ for vacuum input and a ground-state medium), so they do not affect the coherent transmission derived below.

To connect the emitter response to the modal input-output formalism of~\cite{partI}, we decompose the boundary input field into a selected driven channel with amplitude $\hat a(\omega)$ and mode profile $\mathcal{E}_n^{\mathrm{in}}(\mathbf{r},\omega)$, plus an orthogonal complement $\hat{\mathcal{E}}_{\mathrm{in}}^{\perp}$\ankit{orthogonal to what? i don't understand}.  The bare Green kernel $g_0$ (without emitters) propagates the selected channel into the structure, producing the effective input field
\begin{multline}\label{eq:eff_input}
\mathcal{E}_n^{\mathrm{eff}}(\mathbf{r},\omega)
=
-i\int_{S_{\mathrm{in}}} dS_{\mathbf{r}'}\,
g_0(\mathbf{r},\mathbf{r}',\omega)
\\
\times\,
(\bar{n}_{\mathrm{in}}\times\mathcal{E}_n^{\mathrm{in}}(\mathbf{r}',\omega)).
\end{multline}
The drive vector then separates as $\hat\eta_j = [w_{\mathrm{in}}]_j\,\hat a + \hat\eta_j^{\perp}+\hat\eta_P$, where
\begin{equation}\label{eq:w_in_def}
[w_{\mathrm{in}}(\omega)]_j
\equiv
\frac{1}{\hbar}\,\mathcal{D}_j^\dagger\,\mathcal{E}_n^{\mathrm{eff}}(\mathbf{r}_j,\omega)
\end{equation}
is the input coupling vector and $\hat\eta_j^{\perp}=\frac{1}{\hbar}\mathcal{D}^\dagger \hat{\mathcal E}^\perp_{\text{in}}(\mathbf r_j,\omega)$, $\hat\eta_P=\frac{1}{\hbar}\mathcal{D}^\dagger \hat{\mathcal E}_P(\mathbf r_j,\omega)$.The direct background transmission (no emitters) is
\begin{multline}\label{eq:t0_def}
t_0(\omega)
=
\int_{S_{\mathrm{out}}} dS_{\mathbf{r}}\,
\bigl(\mathcal{E}^{\mathrm{out}}\bigr)^\dagger
\cdot (\bar{n}_{\mathrm{out}}\times)
\\
\times\left[
\int_{S_{\mathrm{in}}} dS_{\mathbf{r}'}\,
g_0(\mathbf{r},\mathbf{r}',\omega)\,
(\bar{n}_{\mathrm{in}}\times\mathcal{E}^{\mathrm{in}})
\right].
\end{multline}

\paragraph{Formal solution and collective eigenmodes.}

In matrix form the linear system~\eqref{eq:linear_system} reads $M(\omega)\,\hat{\boldsymbol\sigma}=-\hat{\boldsymbol\eta}$, with
\begin{equation}
M(\omega)\equiv (\omega-\omega_A)I+G(\omega),
\qquad
\hat{\boldsymbol\sigma}=-M^{-1}\hat{\boldsymbol\eta}.
\end{equation}
For a reciprocal background, $g_{EE}(\mathbf{r}_j,\mathbf{r}_k)=g_{EE}^T(\mathbf{r}_k,\mathbf{r}_j)$, so the projected Green matrix is complex symmetric, $G^T=G$.  Its eigendecomposition $G\,v_\xi=\lambda_\xi\,v_\xi$ with transpose orthogonality $v_\xi^T v_{\xi'}=\delta_{\xi\xi'}$ gives
\begin{equation}\label{eq:resolvent}
M^{-1}(\omega)=
\sum_{\xi=1}^N
\frac{v_\xi(\omega)\,v_\xi^T(\omega)}
{(\omega-\omega_A)+\lambda_\xi(\omega)}.
\end{equation}
The poles $\lambda_\xi$ are the collective eigenvalues of the emitter array; their imaginary parts give collective decay rates and their real parts give collective frequency shifts.

\paragraph{Channel-resolved transmission.}

Substituting $\hat{\boldsymbol\sigma} = -M^{-1}\hat{\boldsymbol\eta}$ back into the field and projecting onto a selected output mode $\mathcal{E}^{\mathrm{out}}(\mathbf{r},\omega)$ on the output surface $S_{\mathrm{out}}$ defines the output coupling vector
\begin{multline}\label{eq:w_out_def}
[w_{\mathrm{out}}(\omega)]_k
\equiv
\int_{S_{\mathrm{out}}} dS_{\mathbf{r}}\,
\bigl(\mathcal{E}^{\mathrm{out}}(\mathbf{r},\omega)\bigr)^\dagger
\\
\cdot (\bar{n}_{\mathrm{out}}\times)\,
g(\mathbf{r},\mathbf{r}_k,\omega)\,\mathcal{D}_k.
\end{multline}
For vacuum in all orthogonal channels the coherent transmission coefficient is
\begin{equation}
\label{eq:transmission}
t(\omega)=t_0(\omega)+w_{\mathrm{out}}^T(\omega)\,M^{-1}(\omega)\,w_{\mathrm{in}}(\omega),
\end{equation}
cleanly separating the direct background $t_0$, the collective response $M^{-1}$, and the channel coupling $w_{\mathrm{in}}$, $w_{\mathrm{out}}$.  Inserting the eigendecomposition~\eqref{eq:resolvent} gives the collective-mode expansion
\begin{equation}
\label{eq:collective_mode_expansion}
t(\omega)
=
t_0(\omega)
+
\sum_{\xi=1}^N
\frac{(w_{\mathrm{out}}^T v_\xi)(v_\xi^T w_{\mathrm{in}})}
{(\omega-\omega_A)+\lambda_\xi},
\end{equation}
whose residues are the overlaps of each collective mode with the chosen input and output channels.

\paragraph{Determinant-ratio and single-channel forms.}

Dividing by $t_0$ and applying the matrix determinant lemma, $\det(M+uv^T)=\det M\,(1+v^T M^{-1}u)$, with $u=w_{\mathrm{in}}/t_0$ and $v^T=w_{\mathrm{out}}^T$, gives
\begin{equation}
\label{eq:determinant_ratio}
\frac{t(\omega)}{t_0(\omega)}
=
\frac{\det\!\bigl[M(\omega)+w_{\mathrm{in}}(\omega)\,w_{\mathrm{out}}^T(\omega)/t_0(\omega)\bigr]}
{\det M(\omega)}.
\end{equation}
In the effectively one-dimensional single-channel setting of the main text, the diagonal self-energy $G_{jj}$ separates into a guided-mode contribution (absorbed into the off-diagonal coupling and the channel vectors) and a non-guided remainder $-i\Gamma'/2$ accounting for radiation into all other channels.  Writing $M=\Delta_A I+i\Gamma' I/2-G$ with $\Delta_A\equiv\omega-\omega_A$ and $G$ containing only guided-mode couplings, the determinant ratio becomes
\begin{equation}
\frac{t(\omega)}{t_0(\omega)}
=
\prod_{\xi=1}^N
\frac{\Delta_A+i\Gamma'/2}
{\Delta_A+i\Gamma'/2+\lambda_\xi},
\end{equation}
making the collective pole structure completely explicit.  The channel coupling is handled by true modal projections on the input and output surfaces, eliminating the need for virtual source or receiver dipoles used in earlier derivations.
---------

\paragraph{Channel-resolved transmission.}

To connect $\hat{\boldsymbol\sigma}$ to a measurable output amplitude
we must project the total field at the output surface onto a selected
output mode.
The total field at $\mathbf{r}\in S_{\mathrm{out}}$ receives three
contributions from the same Green-function decomposition used at the
emitter positions: the background input field propagated through the
bare structure, the field radiated by all emitters, and the
polarization noise from the absorbing bulk:
\begin{multline}\label{eq:field_at_out}
\hat{\mathcal{E}}(\mathbf{r},\omega)
=
\hat{\mathcal{E}}_{\mathrm{in}}(\mathbf{r},\omega)
+
\sum_{k=1}^N
g(\mathbf{r},\mathbf{r}_k,\omega)\,\mathcal{D}_k\,\hat\sigma_k(\omega)
\\
+\,\hat{\mathcal{E}}_P(\mathbf{r},\omega).
\end{multline}
Projecting onto the output mode
$\mathcal{E}^{\mathrm{out}}(\mathbf{r},\omega)$ by integrating
$(\mathcal{E}^{\mathrm{out}})^\dagger\cdot(\bar{n}_{\mathrm{out}}\times)$
over $S_{\mathrm{out}}$ extracts the output amplitude operator.
The three terms contribute separately.

The background term gives the direct transmission amplitude
$t_0(\omega)\hat{a}(\omega)$ from the driven channel plus vacuum
fluctuations from all orthogonal input channels; $t_0$ is defined
in~\eqref{eq:t0_def}.

The emitter-radiated term defines the output coupling vector
\begin{multline}\label{eq:w_out_def}
[w_{\mathrm{out}}(\omega)]_k
\equiv
\int_{S_{\mathrm{out}}} dS_{\mathbf{r}}\,
\bigl(\mathcal{E}^{\mathrm{out}}(\mathbf{r},\omega)\bigr)^\dagger
\\
\cdot\,(\bar{n}_{\mathrm{out}}\times)\,
g(\mathbf{r},\mathbf{r}_k,\omega)\,\mathcal{D}_k,
\end{multline}
which encodes the overlap of emitter $k$'s radiation pattern with the
output mode, weighted by the full (dressed) Green tensor.

The polarization-noise term
\begin{equation}
\hat\nu^{\mathrm{out}}(\omega)
\equiv
\int_{S_{\mathrm{out}}} dS_{\mathbf{r}}\,
\bigl(\mathcal{E}^{\mathrm{out}}(\mathbf{r},\omega)\bigr)^\dagger
\cdot\,(\bar{n}_{\mathrm{out}}\times)\,
\hat{\mathcal{E}}_P(\mathbf{r},\omega)
\end{equation}
is the projection of the bulk Langevin noise onto the output mode.
Collecting all three contributions, the full output amplitude operator
is
\begin{multline}\label{eq:aout_full}
\hat{a}_{\mathrm{out}}(\omega)
=
t_0(\omega)\,\hat{a}(\omega)
+
w_{\mathrm{out}}^T(\omega)\,\hat{\boldsymbol\sigma}(\omega)
\\
+\,\hat\nu^{\mathrm{out}}(\omega)
+\hat{a}_{\mathrm{vac}}^{\perp}(\omega),
\end{multline}
where $\hat{a}_{\mathrm{vac}}^{\perp}$ collects the vacuum
fluctuations from all input channels orthogonal to the driven mode.
Substituting the full operator solution
\begin{equation}
\hat{\boldsymbol\sigma}
=
-M^{-1}\!\left[
w_{\mathrm{in}}\hat{a}
+\hat{\boldsymbol\eta}^{\perp}
+\hat{\boldsymbol\eta}^{P}
\right]
\end{equation}
into~\eqref{eq:aout_full} gives
\begin{multline}\label{eq:aout_operator}
\hat{a}_{\mathrm{out}}
=
t_0\hat{a}
-w_{\mathrm{out}}^T M^{-1}w_{\mathrm{in}}\hat{a}
\\
-w_{\mathrm{out}}^T M^{-1}
\bigl(\hat{\boldsymbol\eta}^{\perp}+\hat{\boldsymbol\eta}^{P}\bigr)
+\hat\nu^{\mathrm{out}}
+\hat{a}_{\mathrm{vac}}^{\perp}.
\end{multline}
Equation~\eqref{eq:aout_operator} is the complete input--output
relation: it is an operator identity that holds in every quantum
state and retains all noise sources required for the preservation of
canonical commutation relations.

\paragraph{Coherent transmission.}

The coherent (mean-field) transmission is the ratio
$t=\langle\hat{a}_{\mathrm{out}}\rangle/\langle\hat{a}\rangle$
evaluated in any state with a nonzero input amplitude.
Taking expectation values of~\eqref{eq:aout_operator}, all four noise
operators vanish independently.
The orthogonal vacuum fluctuations satisfy
$\langle\hat{a}_{\mathrm{vac}}^{\perp}\rangle=0$ and
$\langle\hat{\boldsymbol\eta}^{\perp}\rangle=0$ because every
orthogonal channel is in the vacuum state, which is annihilated by
the field annihilation operators.
The polarization noise satisfies
$\langle\hat{\boldsymbol\eta}^{P}\rangle=0$ and
$\langle\hat\nu^{\mathrm{out}}\rangle=0$ because the absorbing medium
is in its ground state: the Langevin polarization
$\hat{\mathcal{P}}_N$ has zero mean by construction, being a
zero-mean quantum noise source with no classical drive.
Consequently,
\begin{equation}
\langle\hat{a}_{\mathrm{out}}\rangle
=
t_0\langle\hat{a}\rangle
-w_{\mathrm{out}}^T M^{-1}w_{\mathrm{in}}\langle\hat{a}\rangle,
\end{equation}
and dividing through by $\langle\hat{a}\rangle$ gives the coherent
transmission coefficient
\begin{equation}\label{eq:transmission}
t(\omega)
=
t_0(\omega)
-
w_{\mathrm{out}}^T(\omega)\,M^{-1}(\omega)\,w_{\mathrm{in}}(\omega).
\end{equation}
The result cleanly separates the direct background $t_0$, the
collective emitter response $M^{-1}$, and the channel--emitter
couplings $w_{\mathrm{in}}$ and $w_{\mathrm{out}}$.
All four noise operators---$\hat{\boldsymbol\eta}^{\perp}$,
$\hat{\boldsymbol\eta}^{P}$, $\hat\nu^{\mathrm{out}}$, and
$\hat{a}_{\mathrm{vac}}^{\perp}$---are invisible to the coherent
transmission but are indispensable in the full operator
relation~\eqref{eq:aout_operator}: they preserve the canonical
commutator $[\hat{a}_{\mathrm{out}},\hat{a}_{\mathrm{out}}^\dagger]=1$
in the presence of dissipation, in exact analogy with the
single-emitter fluctuation--dissipation balance established
in~\eqref{eq:FD-closure}.

Inserting the eigendecomposition~\eqref{eq:resolvent}
into~\eqref{eq:transmission} gives the collective-mode expansion
\begin{equation}\label{eq:collective_mode_expansion}
t(\omega)
=
t_0(\omega)
-
\sum_{\xi=1}^N
\frac{(w_{\mathrm{out}}^T v_\xi)(v_\xi^T w_{\mathrm{in}})}
{(\omega-\omega_A)+\lambda_\xi(\omega)},
\end{equation}
whose residues $(w_{\mathrm{out}}^T v_\xi)(v_\xi^T w_{\mathrm{in}})$
are the products of the input and output overlaps with collective
eigenmode $\xi$.
A mode that is orthogonal to either $w_{\mathrm{in}}$ or
$w_{\mathrm{out}}$ contributes nothing to the transmission regardless
of its linewidth, which is the mechanism underlying dark states and
bound states in the continuum.

\section{Extra: Cavity-waveguide}

\paragraph{Multiport extension.}
\label{sec:cav_two_wg}

For a cavity coupled to two distinct waveguide channels---the geometry of add--drop filters and ring resonators with bus and drop ports---each waveguide contributes an independent self-energy, so the dressed cavity Green function generalizes to
\begin{equation}
G_c(\omega) = \frac{1}{\omega - \omega_c - \Sigma_1(\omega) - \Sigma_2(\omega)}.
\label{eq:dressed_cavity_two_wg}
\end{equation}
The scattering matrix element connecting input channel $n$ on waveguide $b$ to output channel $m$ on waveguide $a$ is
\begin{multline}
S_{mn}^{(ab)}(\omega) = \delta_{ab}\,S_{mn}^{(a,\mathrm{direct})} \\
+ \frac{d_m^{(a)}\,c_n^{(b)}}{\omega - \omega_c - \Sigma_1 - \Sigma_2},
\label{eq:S_two_wg}
\end{multline}
where $c_n^{(b)}$ and $d_m^{(a)}$ are the input and output coupling amplitudes.  For a side-coupled ring resonator with no direct path between bus and drop ports, $S^{(12,\mathrm{direct})} = 0$ and the drop-port transmission is purely cavity-mediated:
\begin{equation}
t_\mathrm{drop}(\omega) = \frac{\sqrt{\kappa_1\kappa_2}}{i(\omega - \omega_c) + (\kappa_i + \kappa_1 + \kappa_2)/2}.
\label{eq:drop_transmission}
\end{equation}
This is the standard add--drop result~\cite{fan2003temporal}, here derived directly from the Green function.  The quantum version follows from~\eqref{eq:quantum_io}, with the Langevin noise compensating the non-unitarity of the multiport scattering matrix due to intrinsic loss.


\paragraph{Waveguide-mediated cavity coupling.}
\label{sec:two_cav_one_wg}

When two cavities couple to a shared waveguide continuum, eliminating the waveguide degrees of freedom via the Dyson equation produces a \emph{matrix-valued} self-energy $[\Sigma_\mathrm{wg}(\omega)]_{\mu\nu}$.  The two-cavity Green function is
\begin{equation}
G_\mathrm{cav}(\omega) = \bigl[\omega I - H_\mathrm{cav} - \Sigma_\mathrm{wg}(\omega)\bigr]^{-1},
\label{eq:dressed_two_cav}
\end{equation}
where
\begin{equation}
[\Sigma_\mathrm{wg}(\omega)]_{\mu\nu} = \sum_n \frac{V_{\mu n}\,V_{\nu n}^*}{\omega - \omega_n + i0^+}.
\label{eq:matrix_self_energy}
\end{equation}
The diagonal elements dress each cavity individually (Lamb shift plus waveguide-induced linewidth), while the off-diagonal element $[\Sigma_\mathrm{wg}]_{12} = J_\mathrm{wg}(\omega) - i\Gamma_{12}(\omega)/2$ provides two new effects: a waveguide-mediated coherent coupling $J_\mathrm{wg}$ that adds to the direct coupling $J$, and a collective dissipative coupling $\Gamma_{12}$ through which the two cavities decay cooperatively into the shared continuum---the photonic analogue of super- and subradiance~\cite{dicke1954coherence}.

In the Markov limit, the total effective Hamiltonian $H_\mathrm{eff} = H_\mathrm{cav} + \Sigma_\mathrm{wg}$ reduces to
\begin{widetext}
\begin{equation}
H_\mathrm{eff} = \begin{pmatrix} \omega_1 - i(\kappa_{1,i} + \kappa_{1,\mathrm{wg}})/2 & J + J_\mathrm{wg} - i\Gamma_{12}/2 \\ J + J_\mathrm{wg} - i\Gamma_{12}/2 & \omega_2 - i(\kappa_{2,i} + \kappa_{2,\mathrm{wg}})/2 \end{pmatrix},
\label{eq:Heff_markov_two_cav}
\end{equation}
\end{widetext}
which has exactly the structure of the phenomenological Hamiltonian~\eqref{eq:Heff_coupled} introduced in Sec.~\ref{sec:coupled_cavities}, but now the couplings and linewidths are determined microscopically by the cavity--waveguide coupling amplitudes and waveguide dispersion.  The full composite Green function is
\begin{multline}
g(\mathbf{r},\mathbf{r}',\omega) \approx g_\mathrm{wg}^{(0)}(\mathbf{r},\mathbf{r}',\omega) \\
+ \sum_{\mu,\nu=1}^{2} \mathcal{U}_\mu(\mathbf{r},\omega)\,\bigl[G_\mathrm{cav}(\omega)\bigr]_{\mu\nu}\,\mathcal{U}_\nu^\dagger(\mathbf{r}',\omega),
\label{eq:full_two_cav_wg}
\end{multline}
where $\mathcal{U}_\mu(\mathbf{r},\omega) = \int g_\mathrm{wg}^{(0)}(\mathbf{r},\mathbf{r}'')\,W_\mu(\mathbf{r}'')\,dV''$ is the cavity mode profile dressed by waveguide propagation---the rank-two generalization of~\eqref{eq:full_cav_wg_green}.

Beyond the Markov regime, near photonic band edges where $v_g \to 0$ the density of states diverges and $\Sigma(\omega)$ acquires strong frequency dependence on the scale of the cavity linewidth.  This produces asymmetric Fano lineshapes~\cite{fano1961effects} from interference between the direct and cavity-mediated paths, and can lead to cavity-photon bound states~\cite{john1994bound} when the cavity frequency lies inside a bandgap ($\Gamma_\mathrm{wg} = 0$).  Throughout this regime, the Dyson form~\eqref{eq:full_cav_wg_green} and the quantum input--output relation~\eqref{eq:quantum_io} remain valid; what changes is only the complexity of $\Sigma(\omega)$.


\ankit{we need to rewrite this last para, I am not able to make the right connection to the transmission amplitude}
When the cavity linewidth is narrow compared to the scale on which $\Sigma(\omega)$ varies, the self-energy may be evaluated at the bare cavity frequency (the Markov approximation), giving
\begin{equation}
G_c(\omega) \approx \frac{1}{\omega - \omega_c - \Delta_\mathrm{L} + i(\kappa_i + \kappa_\mathrm{wg})/2},
\label{eq:markov_cavity}
\end{equation}
with $\kappa_\mathrm{wg} = \Gamma_\mathrm{wg}(\omega_c)$.  The waveguide transmission amplitude then takes the canonical form
\begin{multline}
t(\omega) = 1 \\
- \frac{\kappa_\mathrm{wg}}{i(\omega - \omega_c - \Delta_\mathrm{L}) + (\kappa_i + \kappa_\mathrm{wg})/2},
\label{eq:tcmt_transmission}
\end{multline}
reproducing the standard result of temporal coupled-mode theory~\cite{fan2003temporal,suh2004temporal}.  Substituting the dressed $g$ from~\eqref{eq:full_cav_wg_green} into the quantum input--output relation~\eqref{eq:quantum_io} yields the quantum version, with Langevin noise determined by the optical theorem.
