# Supplementary material for: Modal input-output theory for quantum nanophotonics from the first-order Maxwell operator
Source: arXiv:2610.04043 source file (2026-10-02)
Supplement: Supplementary file 7 [file appendix_output_commutator.tex]

\section{Output commutators in dielectric leads}
\label{app:output_commutator_full}

This appendix derives the canonical output commutator in Eq.~\eqref{eq:output_comm} using the finite-volume optical theorem and an independent evaluation of the projected Green operator. The interior may be structured, dispersive, absorbing, and nonreciprocal. No expansion in eigenmodes of the interior and no Markov approximation are required. We first combine the scattering and material-noise contributions into a projected spectral Green function, and then derive its normalization without assuming the output commutator.

\subsection{Lead assumptions and conventions}

The input and output ports are longitudinally invariant, lossless dielectric leads. Their permittivity and permeability may vary across the transverse plane, so dielectric waveguides and other transversely patterned ports are allowed. A lead mode has the form $\mathcal E_n(\mathbf r_\perp,z)=\mathcal e_n(\mathbf r_\perp)e^{i\beta_n z}$ and solves the Maxwell equation of that dielectric structure. Longitudinal invariance does not mean vacuum or transverse homogeneity. The leads continue outward without returning reflections; any exterior structure that feeds light back must be included in the scattering region, with the port cuts placed beyond it. We work at frequencies where the scattering problem is well defined, away from channel cutoffs and singular poles.

At fixed real frequency, write
\begin{equation}
\begin{gathered}
M=H-k_0\bar\varepsilon,\qquad H=i\bar\nabla\times,
\qquad MG=I,\\
\bar\varepsilon_I=\frac{\bar\varepsilon-\bar\varepsilon^\dagger}{2i}\succeq0.
\end{gathered}
\label{eq:full_oc_M}
\end{equation}
Here $G$ denotes the retarded Green operator whose kernel is $g$ in the main text. Its adjoint $G^\dagger$ includes exchange of source and observation coordinates and has the advanced radiation condition. It is not ordinary retarded propagation through the same absorbing medium.

For the dual field $\mathcal E=[\mathbf E,Z_0\mathbf H]^T$ and outward normal $\hat n$, define
\begin{equation}
B=\bar n\times=
\begin{pmatrix}0&\hat n\times\\-\hat n\times&0\end{pmatrix},
\qquad B^\dagger=B.
\label{eq:full_oc_B}
\end{equation}
This convention gives $\langle\mathcal E|B|\mathcal E\rangle=-4Z_0P_{\rm outward}$. Accordingly, the flux-orthogonal channels satisfy
\begin{equation}
\begin{aligned}
\langle\mathcal E_p^{\rm in}|B|\mathcal E_q^{\rm in}\rangle&=\delta_{pq},\\
\langle\mathcal E_m^{\rm out}|B|\mathcal E_n^{\rm out}\rangle&=-\delta_{mn},\\
\langle\mathcal E_p^{\rm in}|B|\mathcal E_m^{\rm out}\rangle&=0.
\end{aligned}
\label{eq:full_oc_flux}
\end{equation}
All propagating input channels are included, including unoccupied ports and radiation channels; channel sums include continuum integrals where appropriate. This is completeness for the propagating flux channels, not a resolution of arbitrary evanescent boundary fields.

Let $D$ denote the output detector cross-sections. Enclose both the scatterer and $D$ in a larger volume $V$, whose outer port cuts $S=\partial V$ lie farther out in the lossless leads. We distinguish the detector operator $B_D$ from the outer boundary operator $B_S$. The added lead segments contain no absorption, and mode phases are transported consistently between reference planes. Surface and volume integrals are implicit in the operator products below. Coincident detector pairings use the same averaged source and test prescription defined in Sec.~\ref{sec:full_oc_trace}; the detector profiles lie strictly inside $V$.

\subsection{Scattering and material-noise contributions}

Using the output phase convention $\hat b_m=\alpha\langle\mathcal E_m^{\rm out}|B_D|\hat{\mathcal E}\rangle$, write
\begin{equation}
\hat b_m=\sum_pS_{mp}\hat a_p+\hat\xi_m,
\qquad \alpha^2=\frac{2\pi\varepsilon_0}{\hbar k_0},
\label{eq:full_oc_b}
\end{equation}
with
\begin{equation}
S_{mp}=-i\langle\mathcal E_m^{\rm out}|B_DGB_S|
\mathcal E_p^{\rm in}\rangle,
\label{eq:full_oc_S}
\end{equation}
\begin{equation}
\hat\xi_m=\alpha k_0\langle\mathcal E_m^{\rm out}|
B_DG|\hat{\mathcal P}_N\rangle.
\label{eq:full_oc_xi}
\end{equation}
Because the outgoing flux norm is negative, this $\hat b_m$ differs by a common minus sign from the physical outgoing expansion coefficient. Changing that output phase changes the corresponding rows of $S$ and $\hat\xi$ together and leaves their commutators unchanged. Frequency arguments are suppressed except in the operator algebra.

The independent input and material-bath algebras are
\begin{equation}
[\hat a_p(\omega),\hat a_q^\dagger(\omega')]
=\delta_{pq}\delta(\omega-\omega'),
\label{eq:full_oc_a_comm}
\end{equation}
\begin{multline}
[\hat{\mathcal P}_{N,i}(\mathbf x,\omega),
\hat{\mathcal P}_{N,j}^\dagger(\mathbf y,\omega')]
=\frac{\hbar}{\pi\varepsilon_0}
(\bar\varepsilon_I)_{ij}(\mathbf x,\omega)\\
\times\delta^{(3)}(\mathbf x-\mathbf y)\delta(\omega-\omega').
\label{eq:full_oc_P_comm}
\end{multline}
Input--bath cross commutators and annihilation--annihilation commutators vanish. Hence
\begin{equation}
\begin{aligned}
[\hat b_m(\omega),\hat b_n^\dagger(\omega')]
&=C_{mn}(\omega)\delta(\omega-\omega'),\\
C_{mn}&=(SS^\dagger)_{mn}+N_{mn}.
\end{aligned}
\label{eq:full_oc_C}
\end{equation}
Substitution of Eqs.~\eqref{eq:full_oc_S} and~\eqref{eq:full_oc_xi} gives
\begin{multline}
(SS^\dagger)_{mn}
=\langle\mathcal E_m^{\rm out}|B_DGB_S
\left(\sum_p|\mathcal E_p^{\rm in}\rangle
\langle\mathcal E_p^{\rm in}|\right)\\
\times B_SG^\dagger B_D|\mathcal E_n^{\rm out}\rangle,
\label{eq:full_oc_SS}
\end{multline}
\begin{equation}
N_{mn}=2k_0\langle\mathcal E_m^{\rm out}|
B_DG\bar\varepsilon_I G^\dagger B_D|\mathcal E_n^{\rm out}\rangle.
\label{eq:full_oc_N}
\end{equation}
The noise prefactor is $\alpha^2k_0^2\hbar/(\pi\varepsilon_0)=2k_0$. Thus the noise covariance has been obtained from the bath algebra, not from an assumed output commutator.

\subsection{Incoming-mode completeness at the outer boundary}

The incoming projector is
\begin{equation}
P_{\rm in}=\sum_p|\mathcal E_p^{\rm in}\rangle
\langle\mathcal E_p^{\rm in}|B_S.
\label{eq:full_oc_Pin}
\end{equation}
Consequently,
\begin{equation}
(SS^\dagger)_{mn}
=\langle\mathcal E_m^{\rm out}|
B_DGB_SP_{\rm in}G^\dagger B_D|\mathcal E_n^{\rm out}\rangle.
\label{eq:full_oc_SS_Pin}
\end{equation}
To use this closure, consider the auxiliary adjoint field
\begin{equation}
|\psi_n\rangle=G^\dagger B_D|\mathcal E_n^{\rm out}\rangle.
\label{eq:full_oc_psi}
\end{equation}
Its detector source lies inside $S$. The advanced radiation condition therefore leaves only incoming propagating components at the outer cuts. Exterior-decaying evanescent components have zero mutual flux and zero cross-flux with propagating channels; equivalently, evaluate the flux on asymptotic cuts where these components vanish. Within this flux pairing,
\begin{equation}
\langle\psi_m|B_SP_{\rm in}|\psi_n\rangle
=\langle\psi_m|B_S|\psi_n\rangle.
\label{eq:full_oc_Pin_flux}
\end{equation}
This does not assert $P_{\rm in}=I$ on arbitrary boundary traces. Combining the scattering and noise terms now gives
\begin{multline}
C_{mn}=\langle\mathcal E_m^{\rm out}|B_D
\left(GB_SG^\dagger+2k_0G\bar\varepsilon_I G^\dagger\right)\\
\times B_D|\mathcal E_n^{\rm out}\rangle.
\label{eq:full_oc_before_OT}
\end{multline}

\subsection{Finite-volume optical theorem}

To fix the boundary sign and operator ordering explicitly, introduce the formal adjoint differential operator $M^\sharp=H-k_0\bar\varepsilon^\dagger$. Integration by parts gives
\begin{multline}
\langle f|M^\sharp h\rangle_V
-\langle M^\sharp f|h\rangle_V
=i\langle f|B_S|h\rangle_S\\
+2ik_0\langle f|\bar\varepsilon_I|h\rangle_V.
\label{eq:full_oc_green_identity}
\end{multline}
Take arbitrary sources $q_m,q_n$ supported strictly inside $V$ and set $\psi_j=G^\dagger q_j$, so that $M^\sharp\psi_j=q_j$. The left side of Eq.~\eqref{eq:full_oc_green_identity} becomes $\langle q_m|(G-G^\dagger)|q_n\rangle$. Dividing by $i$ yields the optical theorem, understood as an equality for interior source pairings,
\begin{equation}
2\operatorname{Im}G
=GB_SG^\dagger+2k_0G\bar\varepsilon_I G^\dagger,
\label{eq:full_oc_OT}
\end{equation}
where $\operatorname{Im}G=(G-G^\dagger)/(2i)$. The boundary sign is positive for this ordering and the convention in Eq.~\eqref{eq:full_oc_B}. Substituting into Eq.~\eqref{eq:full_oc_before_OT},
\begin{equation}
C_{mn}=2\langle\mathcal E_m^{\rm out}|
B_D\operatorname{Im}G B_D|\mathcal E_n^{\rm out}\rangle.
\label{eq:full_oc_C_ImG}
\end{equation}
It remains to derive this projected spectral normalization independently.

\subsection{Matched-source evaluation of the projected Green operator}
\label{sec:full_oc_trace}

Let $z$ increase outward along a detector lead. Longitudinal invariance allows us to write
\begin{equation}
M=iB_D\partial_z+M_t,
\qquad M\mathcal E_n^{\rm out}=0.
\label{eq:full_oc_lead_M}
\end{equation}
The transverse operator $M_t$ contains the actual dielectric profile and is self-adjoint under transverse integration in the lossless lead, with its physical transverse boundary conditions. No transverse homogeneity is assumed.

Choose a real longitudinal weight $w$ localized around the detector, with
\begin{equation}
\int w(z)\,dz=1,
\qquad W(z)=\int_{-\infty}^z w(t)\,dt.
\label{eq:full_oc_weight}
\end{equation}
Define the averaged modal projection by
\begin{multline}
\langle\mathcal E_m^{\rm out}|B_D|v\rangle_w
=\int dz\,w(z)\\
\times\langle\mathcal E_m^{\rm out}(z)|B_D|v(z)\rangle_\perp.
\label{eq:full_oc_average}
\end{multline}
The mode includes its full longitudinal phase. The adjoint of this same functional is the matched electric-and-magnetic source
\begin{equation}
q_n(z)=w(z)B_D\mathcal E_n^{\rm out}(z).
\label{eq:full_oc_source}
\end{equation}
Consider the field
\begin{equation}
v_n(z)=-iW(z)\mathcal E_n^{\rm out}(z).
\label{eq:full_oc_v}
\end{equation}
Direct substitution gives
\begin{equation}
\begin{aligned}
Mv_n
&=iB_D(-iw\mathcal E_n^{\rm out})
-iW M\mathcal E_n^{\rm out}\\
&=wB_D\mathcal E_n^{\rm out}=q_n.
\end{aligned}
\label{eq:full_oc_source_check}
\end{equation}
This field vanishes toward the scatterer, is purely outgoing beyond the source, and is zero in the other leads. Uniqueness of the retarded problem therefore identifies $v_n=Gq_n$. The matched source sends no field toward the interior, so its response in this construction is independent of interior scattering and absorption. A generic electric-only source would not have this property.

Using Eq.~\eqref{eq:full_oc_flux}, the paired source and detector average gives
\begin{multline}
\langle\mathcal E_m^{\rm out}|B_DGB_D|
\mathcal E_n^{\rm out}\rangle_w
=-i\int dz\,w(z)W(z)\\
\times\langle\mathcal E_m^{\rm out}(z)|B_D|
\mathcal E_n^{\rm out}(z)\rangle_\perp
=i\delta_{mn}\int wW\,dz.
\label{eq:full_oc_project_G_integral}
\end{multline}
Since $W'=w$ and $W$ changes from zero to one,
\begin{equation}
\int wW\,dz=\frac12[W^2]_{-\infty}^{+\infty}=\frac12.
\label{eq:full_oc_half}
\end{equation}
Thus
\begin{equation}
\langle\mathcal E_m^{\rm out}|B_DGB_D|
\mathcal E_n^{\rm out}\rangle_w=\frac{i}{2}\delta_{mn}.
\label{eq:full_oc_project_G}
\end{equation}
Modes supported on different leads have zero overlap because the matched response is confined to its source lead. The result is exact for the paired modal functional and does not use a weak-loss or large-distance approximation.

The averaging does not change the physical output operator. For a physical source-free field $\mathcal E$ in the lossless detector region, both it and the test mode satisfy Eq.~\eqref{eq:full_oc_lead_M}. Hence
\begin{multline}
\partial_z\langle\mathcal E_m^{\rm out}(z)|B_D|
\mathcal E(z)\rangle_\perp
=-i\langle\mathcal E_m^{\rm out}|M_t|\mathcal E\rangle_\perp\\
+i\langle\mathcal E_m^{\rm out}|M_t|\mathcal E\rangle_\perp=0.
\label{eq:full_oc_flux_constancy}
\end{multline}
A normalized longitudinal average therefore measures the same physical modal amplitude as projection at any cross-section in that source-free region. It is not a normalization chosen to enforce a desired commutator.

The artificially driven field $v_n$ does have a source in the detector layer. In the thin-sheet limit, its inward and outward projected traces are zero and $i\delta_{mn}$, respectively. Using the same source and test averaging gives their mean, as derived in Eq.~\eqref{eq:full_oc_half}. Thus the coincident-sheet Green pairing requires this prescription; neither one-sided trace alone equals Eq.~\eqref{eq:full_oc_project_G}.

\subsection{Canonical output algebra}

Taking the adjoint of the projected matrix, using $B_D^\dagger=B_D$ and the same source and test prescription, gives
\begin{equation}
\langle\mathcal E_m^{\rm out}|B_DG^\dagger B_D|
\mathcal E_n^{\rm out}\rangle_w=-\frac{i}{2}\delta_{mn}.
\label{eq:full_oc_project_Gadj}
\end{equation}
This follows by conjugating the matrix element with $m$ and $n$ exchanged; it does not assume $G$ is Hermitian or reciprocal. Equations~\eqref{eq:full_oc_project_G} and~\eqref{eq:full_oc_project_Gadj} imply
\begin{multline}
2\langle\mathcal E_m^{\rm out}|B_D\operatorname{Im}G B_D|
\mathcal E_n^{\rm out}\rangle_w\\
=\frac1i\left(\frac{i}{2}\delta_{mn}
-\left[-\frac{i}{2}\delta_{mn}\right]\right)=\delta_{mn}.
\label{eq:full_oc_project_spectral}
\end{multline}
Combining with Eq.~\eqref{eq:full_oc_C_ImG}, we obtain
\begin{equation}
SS^\dagger+N=I,
\label{eq:full_oc_deficit}
\end{equation}
and therefore
\begin{equation}
[\hat b_m(\omega),\hat b_n^\dagger(\omega')]
=\delta_{mn}\delta(\omega-\omega').
\label{eq:full_oc_final}
\end{equation}
Also $[\hat b_m(\omega),\hat b_n(\omega')]=0$, because the independent input and bath annihilation operators commute. In particular,
\begin{equation}
[\hat\xi_m(\omega),\hat\xi_n^\dagger(\omega')]
=[I-SS^\dagger]_{mn}\delta(\omega-\omega').
\label{eq:full_oc_noise_deficit}
\end{equation}
The optical theorem combines scattering and absorption into the projected $\operatorname{Im}G$, while the matched-source calculation independently fixes its normalization. The proof requires longitudinally invariant lossless port regions with no exterior feedback, but allows transversely patterned dielectric leads and general passive loss inside the scattering volume. It does not establish a local delta-function commutator for arbitrary surface fields.
