# Supplementary material for: Modal input-output theory for quantum nanophotonics from the first-order Maxwell operator
Source: arXiv:2610.04043 source file (2026-10-02)
Supplement: Supplementary file 8 [file appendix_waveguide_green.tex]

\section{Uniform lossless waveguide Green function}
\label{app:waveguide_green}

This appendix derives the propagating-mode contribution used in Eq.~\eqref{eq:guided_green}. The material is lossless and translationally invariant along $z$, but may be patterned across the transverse plane. We use the mode normalization and self-adjoint transverse domain of Appendix~\ref{app:dual_modes}, and work away from channel cutoffs.

Writing $B=\bar{\mathbf z}\times$ and $\mathcal M=\mathcal M_t+iB\partial_z$, translation invariance permits the longitudinal Fourier representation
\begin{equation}
\begin{aligned}
g(\mathbf r,\mathbf r',\omega)
&=\int\frac{d\beta}{2\pi}\,
g_t(\mathbf r_\perp,\mathbf r'_\perp;\beta,\omega)
e^{i\beta(z-z')},\\
(\mathcal M_t-\beta B)g_t
&=\mathbb I_6\delta^{(2)}(\mathbf r_\perp-\mathbf r'_\perp).
\end{aligned}
\label{eq:wgd_fourier}
\end{equation}
The transverse modes satisfy $\mathcal M_t\mathcal E_n=\beta_n B\mathcal E_n$ and $\langle\mathcal E_m|B|\mathcal E_n\rangle_S=s_n\delta_{mn}$. With the block convention in Eq.~\eqref{eq:app_modes_wg_block_operators}, this pairing measures minus the longitudinal power. Thus the energy-flow direction is $\tau_n=-s_n$, with $\tau_n=+1$ for forward propagation.

At a real propagating pole, self-adjointness gives
\begin{equation}
(\beta_n-\beta)\langle\mathcal E_n|B g_t
=\langle\mathcal E_n|.
\label{eq:wgd_residue_projection}
\end{equation}
Consequently the pole residue is fixed by the flux norm, and the propagating part of the transverse Green function is
\begin{equation}
g_{t,\rm prop}
=\sum_{n\in\mathscr P}
\frac{s_n|\mathcal E_n\rangle\langle\mathcal E_n|}
{\beta_n-\beta+i0^+\tau_n}.
\label{eq:wgd_transverse_poles}
\end{equation}
There is no extra $B$ on the right of this Green kernel: its source in Eq.~\eqref{eq:wgd_fourier} is the identity, not the flux operator. For degeneracies, the sum is taken over a flux-orthogonal basis in the degenerate subspace. This pole contribution need not be the full transverse inverse; evanescent and longitudinal/contact contributions must also be retained when reconstructing arbitrary near fields.

The pole shift follows from the retarded limit $\omega\to\omega+i\eta$: $\beta_n(\omega+i\eta)\simeq\beta_n(\omega)+i\eta/v_{g,n}$. For the positive-energy lossless branches considered here, the group and energy velocities have the same sign, so forward poles lie above the real $\beta$ axis and backward poles below it~\cite{collin1990field,felsen1994radiation}. Let $Z=z-z'$. Closing the Fourier contour in the upper half-plane for $Z>0$ and the lower half-plane for $Z<0$ gives
\begin{equation}
\int\frac{d\beta}{2\pi}
\frac{e^{i\beta Z}}{\beta_n-\beta+i0^+\tau_n}
=-i\tau_n\Theta(\tau_n Z)e^{i\beta_n Z}.
\label{eq:wgd_contour}
\end{equation}
Since $s_n=-\tau_n$, the propagating Green kernel is therefore
\begin{multline}
g_{\rm prop}(\mathbf r,\mathbf r',\omega)
=i\sum_{n\in\mathscr P}\Theta\!\bigl(\tau_n(z-z')\bigr)\\
\times\mathcal E_n(\mathbf r_\perp)
\mathcal E_n^\dagger(\mathbf r'_\perp)
e^{i\beta_n(z-z')}.
\label{eq:wgd_real_space}
\end{multline}
Restricting the sum to guided modes gives Eq.~\eqref{eq:guided_green}; radiation channels contribute analogous integrals. Each term propagates away from the source in the direction of the mode's energy flow. Coincident-source traces require a specified averaging prescription, as in Appendix~\ref{app:output_commutator_full}.

For transmission through a uniform guide from $z_L$ to $z_R>z_L$, take $B_{\rm in}=-B$ and $B_{\rm out}=B$. Forward modes have $\langle\mathcal E_m|B|\mathcal E_n\rangle=-\delta_{mn}$. Inserting Eq.~\eqref{eq:wgd_real_space} into the raw positive-flux projection of Eq.~\eqref{eq:S_matrix_braket} therefore gives $-e^{i\beta_n(z_R-z_L)}\delta_{mn}$. The physical outgoing expansion coefficient is minus that projected coefficient, as discussed in Appendix~\ref{app:output_commutator_full}. Equations~\eqref{eq:S_waveguide} and~\eqref{eq:wg_io} display the conventional positive propagation phase using this physical outgoing-amplitude convention. Switching conventions multiplies the entire output row, including its noise term, by $-1$ and leaves observable powers and commutators unchanged.
